# Supplementary material for: Fast and automated biomarker detection in breath samples with machine learning
Source: arXiv:2006.01772 ancillary file (2020-05-24)
Supplement: Supplementary file 1 [file Supplementary_Information.pdf]

Supplementary Information

# Fast and automated biomarker detection in breath samples with machine learning

A.Skarysz et al.

# Contents


**1 Target VOCs** **3**

**2 Network architectures** **4**

**3 VGG-8-1D model – Results** **21**

**4 DenseNet-40-1D model – Results** **65**

**5 ResNet-34-1D model – Results** **71**

**6 Intersection of the models – Results** **77**

**7 GC-MS instrumentation** **83**

# 1 Target VOCs

Supplementary Table 1: Target volotile organic compound properties.

_Label_ - the class label of VOC. _VOC_ - target volatile organic compound. _VOCCluster Code_ - VOC code derived from [1]. _IUPAC Name_ - International Union of Pure and Applied Chemistry name of each VOC. CAS - a unique numerical identifier assigned by the Chemical Abstracts Service to each VOC. _5 Top m/z Peaks_ - m/z values of 5 top ions from the VOC mass spectrum, derived from VOC dataset and according to NIST library. _Mean peakRT 1_ - mean retention time value of the VOC before GC column change. _Min peakRT 1_ - minimum retention time value of the VOC before GC column change. _Max peakRT 1_ - maximum retention time value of the VOC before GC column change. _Mean peakRT 2_ - mean retention time value of the VOC after GC column change. _Min peakRT 2_ - minimum retention time value of the VOC after GC column change. _Max peakRT 2_ - maximum retention time value of the VOC after GC column change. _Mean EIC-Area_ - mean value of VOC peak area on extracted ion chromatogram (EIC) of a top VOC ion; marker of VOC concentration. _Quantity in VOC dataset_ - number of the VOC data-points in the (non-augmented) training set (BS – breath sample, ES – environmental sample). _Quantity in Testset_ - number of the target VOC instances reported by the ground truth in the GC-MS samples from test set.

| Label | VOC | VOCCluster Code [1] | IUPAC Name | CAS | 5 Top m/z Peaks | Mean peakRT 1 | Min peakRT 1 | Max peakRT 1 | Mean peakRT 2 | Min peakRT 2 | Max peakRT 2 | Mean EIC-Area | Quantity in VOC dataset | Quantity in Testset |
|---|---|---|---|---|---|---|---|---|---|---|---|---|---|---|
| 1 | Ethanol | BRI-686-45-46-43-42-44 | ethanol | 64-17-5 | dataset 45 - 46 - 43 - 42 - 44<br>NIST 45 - 46 - 43 - 42 - 41 | 2.926 | 2.873 | 2.942 | 3.178 | 3.136 | 3.236 | 203414 | BS / ES 38 / 15<br>total 53 | BS / ES 15 / 5<br>total 20 |
| 2 | Dimethyl sulfide | BRI-692-62-47-45-46-61 | methylsulfanylmethane | 75-18-3 | dataset 62 - 47 - 45 - 46 - 61<br>NIST 62 - 47 - 45 - 46 - 61 | 3.059 | 3.001 | 3.085 | 3.390 | 3.120 | 3.469 | 50868 | BS / ES 52 / 3<br>total 55 | BS / ES 29 / 0<br>total 29 |
| 3 | 2-Methylfuran | BRI-689-82-53-81-50-51 | 2-methylfuran | 534-22-5 | dataset 82 - 53 - 81 - 50 - 51<br>NIST 82 - 53 - 81 - 54 - 51 | 3.409 | 3.332 | 3.443 | 3.931 | 3.812 | 4.061 | 86179 | BS / ES 59 / 2<br>total 61 | BS / ES 30 / 0<br>total 30 |
| 4 | Trichloromethane-d | BRI-712-84-86-47-49-88 | trichloro(deuterio)methane | 865-49-6 | dataset 84 - 86 - 47 - 49 - 88<br>NIST 84 - 86 - 47 - 49 - 88 | 3.488 | 3.413 | 3.523 | 3.959 | 3.387 | 4.125 | 104989 | BS / ES 65 / 17<br>total 82 | BS / ES 30 / 8<br>total 38 |
| 5 | Benzene | BRI-707-78-77-51-50-52 | benzene | 71-43-2 | dataset 78 - 77 - 51 - 50 - 52<br>NIST 78 - 77 - 51 - 50 - 52 | 3.774 | 3.219 | 4.273 | 4.431 | 4.263 | 4.648 | 168917 | BS / ES 58 / 16<br>total 74 | BS / ES 28 / 8<br>total 36 |
| 6 | Propionic acid | BRI-724-45-74-73-57-55 | propanoic acid | 79-09-4 | dataset 45 - 74 - 73 - 57 - 55<br>NIST 74 - 45 - 73 - 57 - 55 | 3.973 | 3.875 | 4.325 | 4.752 | 4.464 | 5.580 | 8586 | BS / ES 9 / 13<br>total 22 | BS / ES 7 / 4<br>total 11 |
| 7 | Dimethyl disulfide | BRI-767-94-45-79-46-47 | (methyldisulfanyl)methane | 624-92-0 | dataset 94 - 45 - 79 - 46 - 47<br>NIST 94 - 79 - 45 - 46 - 47 | 4.693 | 4.574 | 4.746 | 5.656 | 5.393 | 5.968 | 282724 | BS / ES 46 / 1<br>total 47 | BS / ES 23 / 0<br>total 23 |
| 8 | Toluene-D8 | BRI-780-98-100-42-70-54 | 1,2,3,4,5-pentadeuterio-6-(trideuteriomethyl)benzene | 2037-26-5 | dataset 98 - 100 - 42 - 70 - 54<br>NIST 98 - 100 - 42 - 70 - 99 | 4.936 | 4.816 | 5.000 | 5.969 | 5.696 | 6.338 | 63756 | BS / ES 59 / 17<br>total 76 | BS / ES 29 / 8<br>total 37 |
| 9 | Toluene | BRI-782-91-92-65-63-51 | toluene | 108-88-3 | dataset 91 - 92 - 65 - 63 - 51<br>NIST 91 - 92 - 65 - 63 - 51 | 5.001 | 4.879 | 5.067 | 6.058 | 5.769 | 6.423 | 134743 | BS / ES 64 / 17<br>total 81 | BS / ES 30 / 8<br>total 38 |
| 10 | 3-Methylthiophene | BRI-792-97-98-45-53-69 | 3-methylthiophene | 616-44-4 | dataset 97 - 98 - 45 - 53 - 69<br>NIST 97 - 98 - 45 - 53 - 99 | 5.214 | 5.089 | 5.284 | 6.318 | 6.020 | 6.690 | 120621 | BS / ES 57 / 2<br>total 59 | BS / ES 30 / 0<br>total 30 |
| 11 | Octane | BRI-803-43-41-85-57-71 | octane | 111-65-9 | dataset 43 - 41 - 85 - 57 - 71<br>NIST 43 - 41 - 57 - 85 - 71 | 5.493 | 5.307 | 5.865 | 6.691 | 6.192 | 7.215 | 13121 | BS / ES 36 / 4<br>total 40 | BS / ES 18 / 1<br>total 19 |
| 12 | Hexanal | BRI-808-44-41-56-43-57 | hexanal | 66-25-1 | dataset 44 - 41 - 56 - 43 - 57<br>NIST 44 - 56 - 41 - 43 - 57 | 5.564 | 5.472 | 5.616 | 6.672 | 6.357 | 7.092 | 11611 | BS / ES 42 / 14<br>total 56 | BS / ES 19 /6<br>total 25 |
| 13 | 2,4-Dimethylheptane | BRI-805-43-85-41-57-71 | 2,4-dimethylheptane | 2213-23-2 | dataset 43 - 85 - 41 - 57 - 71<br>NIST 43 - 85 - 57 - 71 - 41 | 5.817 | 5.305 | 5.917 | 7.145 | 6.831 | 7.599 | 76791 | BS / ES 59 / 11<br>total 70 | BS / ES 28 / 5<br>total 33 |
| 14 | 2,4-Dimethylheptane | BRI-835-43-70-55-41-56 | 2,4-dimethylhept-1-ene | 19549-87-2 | dataset 43 - 70 - 55 - 41 - 56<br>NIST 43 - 70 - 55 - 57 - 41 | 6.307 | 6.085 | 7.160 | 7.708 | 7.301 | 9.079 | 33738 | BS / ES 59 / 7<br>total 66 | BS / ES 30 / 3<br>total 33 |
| 15 | 3-Heptanone | BRI-881-57-41-85-72-43 | heptan-3-one | 106-35-4 | dataset 57 - 41 - 85 - 72 - 43<br>NIST 57 - 85 - 41 - 72 - 114 | 7.403 | 7.264 | 7.511 | 8.839 | 8.436 | 9.380 | 21034 | BS / ES 46 / 13<br>total 59 | BS / ES 18 / 5<br>total 23 |
| 16 | Heptanal | BRI-887-44-41-43-70-55 | heptanal | 111-71-7 | dataset 44 - 41 - 43 - 70 - 55<br>NIST 70 - 41 - 44 - 43 - 55 | 7.816 | 7.685 | 7.886 | 9.324 | 8.704 | 11.035 | 5482 | BS / ES 40 / 15<br>total 55 | BS / ES 17 / 6<br>total 23 |
| 17 | Benzaldehyde | BRI-958-77-105-106-51-50 | benzaldehyde | 100-52-7 | dataset 77 - 105 - 106 - 51 - 50<br>NIST 77 - 106 - 105 - 51 - 50 | 9.545 | 9.369 | 9.646 | 11.060 | 10.579 | 11.689 | 52375 | BS / ES 65 / 17<br>total 82 | BS / ES 30 / 8<br>total 38 |
| 18 | Benzonitrile | BRI-984-103-76-50-51-75 | benzonitrile | 100-47-0 | dataset 103 - 76 - 50 - 51 - 75<br>NIST 103 - 76 - 50 - 51 - 75 | 10.197 | 10.029 | 10.301 | 11.803 | 11.285 | 12.430 | 18154 | BS / ES 60 / 17<br>total 77 | BS / ES 29 / 7<br>total 36 |
| 19 | Octanal | BRI-998-41-43-44-57-55 | octanal | 124-13-0 | dataset 41 - 43 - 44 - 57 - 55<br>NIST 43 - 44 - 41 - 56 - 84 | 10.628 | 10.438 | 11.592 | 12.235 | 11.755 | 12.966 | 6407 | BS / ES 45 / 14<br>total 59 | BS / ES 20 / 6<br>total 26 |
| 20 | Limonene | BRI-1002-68-67-93-79-41 | 1-methyl-4-prop-1-en-2-ylcyclohexene | 138-86-3 | dataset 68 - 67 - 93 - 79 - 41<br>NIST 68 - 93 - 67 - 79 - 136 | 11.298 | 11.079 | 11.421 | 13.115 | 12.613 | 13.756 | 156328 | BS / ES 65 / 14<br>total 79 | BS / ES 30 / 7<br>total 37 |
| 21 | 2-Ethylhexanol | BRI-999-57-41-43-55-56 | 2-ethylhexan-1-ol | 104-76-7 | dataset 57 - 41 - 43 - 55 - 56<br>NIST 57 - 41 - 43 - 55 - 56 | 11.543 | 10.883 | 12.898 | 13.026 | 12.529 | 14.059 | 104600 | BS / ES 45 / 14<br>total 59 | BS / ES 19 / 8<br>total 27 |
| 22 | Nonanal | BRI-1102-41-57-43-55-56 | nonanal | 124-19-6 | dataset 41 - 57 - 43 - 55 - 56<br>NIST 57 - 41 - 43 - 56 - 44 | 13.559 | 13.335 | 13.657 | 15.286 | 14.781 | 15.962 | 20544 | BS / ES 57 / 15<br>total 72 | BS / ES 25 / 7<br>total 32 |
| 23 | Dodecane | BRI-1171-57-43-41-71-85 | dodecane | 112-40-3 | dataset 57 - 43 - 41 - 71 - 85<br>NIST 57 - 43 - 71 - 41 - 85 | 16.162 | 15.928 | 16.303 | 18.069 | 17.562 | 18.735 | 65787 | BS / ES 64 / 14<br>total 78 | BS / ES 30 / 6<br>total 36 |
| 24 | Decanal | BRI-1217-41-43-57-55-44 | decanal | 112-31-2 | dataset 41 - 43 - 57 - 55 - 44<br>NIST 43 - 41 - 57 - 55 - 44 | 16.507 | 16.316 | 16.603 | 18.289 | 17.748 | 18.974 | 9868 | BS / ES 38 / 13<br>total 51 | BS / ES 18 / 6<br>total 24 |
| 25 | 2-Phenoxyethanol | BRI-1194-94-77-138-66-51 | 2-phenoxyethanol | 122-99-6 | dataset 94 - 77 - 138 - 66 - 51<br>NIST 94 - 77 - 138 - 66 - 51 | 16.897 | 16.835 | 17.016 | 18.733 | 18.223 | 19.508 | 21743 | BS / ES 21 / 12<br>total 33 | BS / ES 2 / 5<br>total 7 |
| 26 | Phthalic acid | BRI-1325-104-76-50-74-148 | phthalic acid | 88-99-3 | dataset 104 - 76 - 50 - 74 - 148<br>NIST 104 - 76 - 50 - 148 - 74 | 19.695 | 19.510 | 19.803 | 21.464 | 20.923 | 22.324 | 17780 | BS / ES 41 / 16<br>total 57 | BS / ES 15 / 7<br>total 22 |
| 27 | Tetradecane | BRI-1415-57-43-71-41-85 | tetradecane | 629-59-4 | dataset 57 - 43 - 71 - 41 - 85<br>NIST 57 - 43 - 71 - 85 - 41 | 21.610 | 21.375 | 21.760 | 23.544 | 23.005 | 24.224 | 45778 | BS / ES 61 / 14<br>total 75 | BS / ES 27 / 5<br>total 32 |
| 28 | 1,4-Diacetylbenzene | BRI-1459-147-43-91-119-162 | 1-(4-acetylphenyl)ethanone | 1009-61-6 | dataset 147 - 43 - 91 - 119 - 162<br>NIST 147 - 43 - 91 - 119 - 162 | 22.753 | 22.518 | 22.875 | 24.588 | 24.020 | 25.402 | 37343 | BS / ES 47 / 8<br>total 55 | BS / ES 13 / 4<br>total 17 |
| 29 | 3,3,6,6-Tetraphenyl-1,2,4,5-tetroxane | BRI-1644-105-77-182-51-50 | 3,3,6,6-tetraphenyl-1,2,4,5-tetraoxane | 16204-36-7 | dataset 105 - 77 - 182 - 51 - 50<br>NIST 105 - 77 - 182 - 51 - 107 | 27.550 | 27.338 | 27.678 | 29.416 | 28.829 | 30.272 | 4301 | BS / ES 49 / 12<br>total 61 | BS / ES 25 / 6<br>total 31 |
| 30 | 2,5-Diphenyl-1,4-benzoquinone | BRI-2344-102-260-76-232-0 | 2,5-diphenylcyclohexa-2,5-diene-1,4-dione | 844-51-9 | dataset 102 - 260 - 76 - 232 - 0<br>NIST 102 - 260 - 259 - 232 - 76 | 41.891 | 41.629 | 42.043 | 43.825 | 43.187 | 44.741 | 84612 | BS / ES 58 / 16<br>total 74 | BS / ES 27 / 5<br>total 32 |
| | | | | | | | | | | | | | **Total Trainset** **1868** | **Total Testset** **845** |
| | | | | | | | | | | | | | + | |
| | | | | | | | | | | | | | Negative class 1868 | |

[1] - Alkhalifah Y. et al., 2009. _VOCCluster: Untargeted Metabolomics Feature Clustering Approach for Clinical Breath Gas Chromatography - Mass Spectrometry Data_

## 2 Network architectures

Supplementary Table 2.1: VGG-4-1D network architecture. Network was implemented using Keras with Tensorflow backend and trained for 10 epochs with 32 batch size.

| Layer | | (type) | Output Shape | # Param | Filter size | Stride | Padding | Activation |
|---|---|---|---|---|---|---|---|---|
| | input_1 | (InputLayer) | (None, 80, 411, 1) | 0 | — | — | — | — |
| 1 | conv2d_1 | (Conv2D) | (None, 78, 411, 32) | 128 | (3, 1) | (1, 1) | valid | relu |
| 2 | conv2d_2 | (Conv2D) | (None, 76, 411, 32) | 3104 | (3, 1) | (1, 1) | valid | relu |
| | max_pooling2d_1 | (MaxPooling2D) | (None, 38, 411, 32) | 0 | (2, 1) | (2, 1) | valid | — |
| | dropout_1 | (Dropout) | (None, 38, 411, 32) | 0 | — | — | — | — |
| | flatten_1 | (Flatten) | (None, 499776) | 0 | — | — | — | — |
| 3 | dense_1 | (Dense) | (None, 256) | 127942912 | — | — | — | relu |
| | dropout_4 | (Dropout) | (None, 256) | 0 | — | — | — | — |
| 4 | dense_2 | (Dense) | (None, 31) | 7967 | — | — | — | softmax |

| | |
|---|---|
| **Total parameters:** | **127,954,111** |
| **Trainable parameters:** | **127,954,111** |
| **Non-trainable parameters:** | **0** |

Supplementary Table 2.2: VGG-4-2D network architecture. Network was implemented using Keras with Tensorflow backend and trained for 10 epochs with 32 batch size.

| | Layer | (type) | Output Shape | # Param | Filter size | Stride | Padding | Activation |
|---|---|---|---|---|---|---|---|---|
| | input_1 | (InputLayer) | (None, 80, 411, 1) | 0 | — | — | — | — |
| 1 | conv2d_1 | (Conv2D) | (None, 78, 409, 32) | 320 | (3, 3) | (1, 1) | valid | relu |
| 2 | conv2d_2 | (Conv2D) | (None, 76, 407, 32) | 9248 | (3, 3) | (1, 1) | valid | relu |
| | max_pooling2d_1 | (MaxPooling2D) | (None, 38, 203, 32) | 0 | (2, 2) | (2, 2) | valid | — |
| | dropout_1 | (Dropout) | (None, 38, 203, 32) | 0 | — | — | — | — |
| | flatten_1 | (Flatten) | (None, 246848) | 0 | — | — | — | — |
| 3 | dense_1 | (Dense) | (None, 256) | 63193344 | — | — | — | relu |
| | dropout_4 | (Dropout) | (None, 256) | 0 | — | — | — | — |
| 4 | dense_2 | (Dense) | (None, 31) | 7967 | — | — | — | softmax |

| | |
|---|---|
| **Total parameters:** | **63,210,879** |
| **Trainable parameters:** | **63,210,879** |
| **Non-trainable parameters:** | **0** |

Supplementary Table 2.3: VGG-6-1D network architecture. Network was implemented using Keras with Tensorflow backend and trained for 10 epochs with 32 batch size.

| Layer | (type) | Output Shape | # Param | Filter size | Stride | Padding | Activation |
|---|---|---|---|---|---|---|---|
| input_1 | (InputLayer) | (None, 80, 411, 1) | 0 | — | — | — | — |
| 1 conv2d_1 | (Conv2D) | (None, 78, 411, 32) | 128 | (3, 1) | (1, 1) | valid | relu |
| 2 conv2d_2 | (Conv2D) | (None, 76, 411, 32) | 3104 | (3, 1) | (1, 1) | valid | relu |
| max_pooling2d_1 | (MaxPooling2D) | (None, 38, 411, 32) | 0 | (2, 1) | (2, 1) | valid | — |
| dropout_1 | (Dropout) | (None, 38, 411, 32) | 0 | — | — | — | — |
| 3 conv2d_3 | (Conv2D) | (None, 36, 411, 64) | 6208 | (3, 1) | (1, 1) | valid | relu |
| 4 conv2d_4 | (Conv2D) | (None, 34, 411, 64) | 12352 | (3, 1) | (1, 1) | valid | relu |
| max_pooling2d_2 | (MaxPooling2D) | (None, 17, 411, 64) | 0 | (2, 1) | (2, 1) | valid | — |
| dropout_2 | (Dropout) | (None, 17, 411, 64) | 0 | — | — | — | — |
| flatten_1 | (Flatten) | (None, 447168) | 0 | — | — | — | — |
| 5 dense_1 | (Dense) | (None, 256) | 114475264 | — | — | — | relu |
| dropout_4 | (Dropout) | (None, 256) | 0 | — | — | — | — |
| 6 dense_2 | (Dense) | (None, 31) | 7967 | — | — | — | softmax |

| | |
|---|---|
| **Total parameters:** | **114,505,023** |
| **Trainable parameters:** | **114,505,023** |
| **Non-trainable parameters:** | **0** |

Supplementary Table 2.4: VGG-6-2D network architecture. Network was implemented using Keras with Tensorflow backend and trained for 10 epochs with 32 batch size.

| | Layer | (type) | Output Shape | # Param | Filter size | Stride | Padding | Activation |
|---|---|---|---|---|---|---|---|---|
| | input_1 | (InputLayer) | (None, 80, 411, 1) | 0 | — | — | — | — |
| 1 | conv2d_1 | (Conv2D) | (None, 78, 409, 32) | 320 | (3, 3) | (1, 1) | valid | relu |
| 2 | conv2d_2 | (Conv2D) | (None, 76, 407, 32) | 9248 | (3, 3) | (1, 1) | valid | relu |
| | max_pooling2d_1 | (MaxPooling2D) | (None, 38, 203, 32) | 0 | (2, 2) | (2, 2) | valid | — |
| | dropout_1 | (Dropout) | (None, 38, 203, 32) | 0 | — | — | — | — |
| 3 | conv2d_3 | (Conv2D) | (None, 36, 201, 64) | 18496 | (3, 3) | (1, 1) | valid | relu |
| 4 | conv2d_4 | (Conv2D) | (None, 34, 199, 64) | 36928 | (3, 3) | (1, 1) | valid | relu |
| | max_pooling2d_2 | (MaxPooling2D) | (None, 17, 99, 64) | 0 | (2, 2) | (2, 2) | valid | — |
| | dropout_2 | (Dropout) | (None, 17, 99, 64) | 0 | — | — | — | — |
| | flatten_1 | (Flatten) | (None, 107712) | 0 | — | — | — | — |
| 5 | dense_1 | (Dense) | (None, 256) | 27574528 | — | — | — | relu |
| | dropout_4 | (Dropout) | (None, 256) | 0 | — | — | — | — |
| 6 | dense_2 | (Dense) | (None, 31) | 7967 | — | — | — | softmax |

| | |
|---|---|
| **Total parameters:** | **27,647,487** |
| **Trainable parameters:** | **27,647,487** |
| **Non-trainable parameters:** | **0** |

Supplementary Table 2.5: VGG-8-1D network architecture. Network was implemented using Keras with Tensorflow backend and trained for 10 epochs with 32 batch size.

| Layer | (type) | Output Shape | # Param | Filter size | Stride | Padding | Activation |
|---|---|---|---|---|---|---|---|
| input_1 | (InputLayer) | (None, 80, 411, 1) | 0 | — | — | — | — |
| 1 conv2d_1 | (Conv2D) | (None, 78, 411, 32) | 128 | (3, 1) | (1, 1) | valid | relu |
| 2 conv2d_2 | (Conv2D) | (None, 76, 411, 32) | 3104 | (3, 1) | (1, 1) | valid | relu |
| max_pooling2d_1 | (MaxPooling2D) | (None, 38, 411, 32) | 0 | (2, 1) | (2, 1) | valid | — |
| dropout_1 | (Dropout) | (None, 38, 411, 32) | 0 | — | — | — | — |
| 3 conv2d_3 | (Conv2D) | (None, 36, 411, 64) | 6208 | (3, 1) | (1, 1) | valid | relu |
| 4 conv2d_4 | (Conv2D) | (None, 34, 411, 64) | 12352 | (3, 1) | (1, 1) | valid | relu |
| max_pooling2d_2 | (MaxPooling2D) | (None, 17, 411, 64) | 0 | (2, 1) | (2, 1) | valid | — |
| dropout_2 | (Dropout) | (None, 17, 411, 64) | 0 | — | — | — | — |
| 5 conv2d_5 | (Conv2D) | (None, 15, 411, 128) | 24704 | (3, 1) | (1, 1) | valid | relu |
| 6 conv2d_6 | (Conv2D) | (None, 13, 411, 128) | 49280 | (3, 1) | (1, 1) | valid | relu |
| max_pooling2d_3 | (MaxPooling2D) | (None, 6, 411, 128) | 0 | (2, 1) | (2, 1) | valid | — |
| dropout_3 | (Dropout) | (None, 6, 411, 128) | 0 | — | — | — | — |
| flatten_1 | (Flatten) | (None, 315648) | 0 | — | — | — | — |
| 7 dense_1 | (Dense) | (None, 256) | 80806144 | — | — | — | relu |
| dropout_4 | (Dropout) | (None, 256) | 0 | — | — | — | — |
| 8 dense_2 | (Dense) | (None, 31) | 7967 | — | — | — | softmax |

| | |
|---|---|
| **Total parameters:** | **80,909,887** |
| **Trainable parameters:** | **80,909,887** |
| **Non-trainable parameters:** | **0** |

Supplementary Table 2.6: VGG-8-2D network architecture. Network was implemented using Keras with Tensorflow backend and trained for 10 epochs with 32 batch size.

| | Layer | (type) | Output Shape | # Param | Filter size | Stride | Padding | Activation |
|---|---|---|---|---|---|---|---|---|
| | input_1 | (InputLayer) | (None, 80, 411, 1) | 0 | — | — | — | — |
| 1 | conv2d_1 | (Conv2D) | (None, 78, 409, 32) | 320 | (3, 3) | (1, 1) | valid | relu |
| 2 | conv2d_2 | (Conv2D) | (None, 76, 407, 32) | 9248 | (3, 3) | (1, 1) | valid | relu |
| | max_pooling2d_1 | (MaxPooling2 | (None, 38, 203, 32) | 0 | (2, 2) | (2, 2) | valid | — |
| | dropout_1 | (Dropout) | (None, 38, 203, 32) | 0 | — | — | — | — |
| 3 | conv2d_3 | (Conv2D) | (None, 36, 201, 64) | 18496 | (3, 3) | (1, 1) | valid | relu |
| 4 | conv2d_4 | (Conv2D) | (None, 34, 199, 64) | 36928 | (3, 3) | (1, 1) | valid | relu |
| | max_pooling2d_2 | (MaxPooling2 | (None, 17, 99, 64) | 0 | (2, 2) | (2, 2) | valid | — |
| | dropout_2 | (Dropout) | (None, 17, 99, 64) | 0 | — | — | — | — |
| 5 | conv2d_5 | (Conv2D) | (None, 15, 97, 128) | 73856 | (3, 3) | (1, 1) | valid | relu |
| 6 | conv2d_6 | (Conv2D) | (None, 13, 95, 128) | 147584 | (3, 3) | (1, 1) | valid | relu |
| | max_pooling2d_3 | (MaxPooling2 | (None, 6, 47, 128) | 0 | (2, 2) | (2, 2) | valid | — |
| | dropout_3 | (Dropout) | (None, 6, 47, 128) | 0 | — | — | — | — |
| | flatten_1 | (Flatten) | (None, 36096) | 0 | — | — | — | — |
| 7 | dense_1 | (Dense) | (None, 256) | 9240832 | — | — | — | relu |
| | dropout_4 | (Dropout) | (None, 256) | 0 | — | — | — | — |
| 8 | dense_2 | (Dense) | (None, 31) | 7967 | — | — | — | softmax |

| | |
|---|---|
| **Total parameters:** | **9,535,231** |
| **Trainable parameters:** | **9,535,231** |
| **Non-trainable parameters:** | **0** |

Supplementary Table 2.7: VGG-16-2D network architecture. Network was implemented using Keras with Tensorflow backend and trained for 10 epochs with 32 batch size.

| Layer | (type) | Output Shape | # Param | Filter size | Stride | Padding | Activation |
|---|---|---|---|---|---|---|---|
| input_1 | (InputLayer) | (None, 80, 411, 1) | 0 | — | — | — | — |
| 1 conv2d_1 | (Conv2D) | (None, 80, 411, 64) | 640 | (3, 3) | (1, 1) | same | — |
| batch_normalization_1 | (BatchNormalization) | (None, 80, 411, 64) | 256 | — | — | — | — |
| activation_1 | (Activation) | (None, 80, 411, 64) | 0 | — | — | — | relu |
| 2 conv2d_2 | (Conv2D) | (None, 80, 411, 64) | 36928 | (3, 3) | (1, 1) | same | — |
| batch_normalization_2 | (BatchNormalization) | (None, 80, 411, 64) | 256 | — | — | — | — |
| activation_2 | (Activation) | (None, 80, 411, 64) | 0 | — | — | — | relu |
| max_pooling2d_1 | (MaxPooling2D) | (None, 40, 205, 64) | 0 | (2, 2) | (2, 2) | valid | — |
| 3 conv2d_3 | (Conv2D) | (None, 40, 205, 128) | 73856 | (3, 3) | (1, 1) | same | — |
| batch_normalization_3 | (BatchNormalization) | (None, 40, 205, 128) | 512 | — | — | — | — |
| activation_3 | (Activation) | (None, 40, 205, 128) | 0 | — | — | — | relu |
| 4 conv2d_4 | (Conv2D) | (None, 40, 205, 128) | 147584 | (3, 3) | (1, 1) | same | — |
| batch_normalization_4 | (BatchNormalization) | (None, 40, 205, 128) | 512 | — | — | — | — |
| activation_4 | (Activation) | (None, 40, 205, 128) | 0 | — | — | — | relu |
| max_pooling2d_2 | (MaxPooling2D) | (None, 20, 102, 128) | 0 | (2, 2) | (2, 2) | valid | — |
| 5 conv2d_5 | (Conv2D) | (None, 20, 102, 256) | 295168 | (3, 3) | (1, 1) | same | — |
| batch_normalization_5 | (BatchNormalization) | (None, 20, 102, 256) | 1024 | — | — | — | — |
| activation_5 | (Activation) | (None, 20, 102, 256) | 0 | — | — | — | relu |
| 6 conv2d_6 | (Conv2D) | (None, 20, 102, 256) | 590080 | (3, 3) | (1, 1) | same | — |
| batch_normalization_6 | (BatchNormalization) | (None, 20, 102, 256) | 1024 | — | — | — | — |
| activation_6 | (Activation) | (None, 20, 102, 256) | 0 | — | — | — | relu |
| 7 conv2d_7 | (Conv2D) | (None, 20, 102, 256) | 590080 | (3, 3) | (1, 1) | same | — |
| batch_normalization_7 | (BatchNormalization) | (None, 20, 102, 256) | 1024 | — | — | — | — |
| activation_7 | (Activation) | (None, 20, 102, 256) | 0 | — | — | — | relu |
| max_pooling2d_3 | (MaxPooling2D) | (None, 10, 51, 256) | 0 | (2, 2) | (2, 2) | valid | — |
| 8 conv2d_8 | (Conv2D) | (None, 10, 51, 512) | 1180160 | (3, 3) | (1, 1) | same | — |
| batch_normalization_8 | (BatchNormalization) | (None, 10, 51, 512) | 2048 | — | — | — | — |
| activation_8 | (Activation) | (None, 10, 51, 512) | 0 | — | — | — | relu |
| 9 conv2d_9 | (Conv2D) | (None, 10, 51, 512) | 2359808 | (3, 3) | (1, 1) | same | — |
| batch_normalization_9 | (BatchNormalization) | (None, 10, 51, 512) | 2048 | — | — | — | — |
| activation_9 | (Activation) | (None, 10, 51, 512) | 0 | — | — | — | relu |
| 10 conv2d_10 | (Conv2D) | (None, 10, 51, 512) | 2359808 | (3, 3) | (1, 1) | same | — |
| batch_normalization_10 | (BatchNormalization) | (None, 10, 51, 512) | 2048 | — | — | — | — |
| activation_10 | (Activation) | (None, 10, 51, 512) | 0 | — | — | — | relu |
| max_pooling2d_4 | (MaxPooling2D) | (None, 5, 25, 512) | 0 | (2, 2) | (2, 2) | valid | — |
| 11 conv2d_11 | (Conv2D) | (None, 5, 25, 512) | 2359808 | (3, 3) | (1, 1) | same | — |
| batch_normalization_11 | (BatchNormalization) | (None, 5, 25, 512) | 2048 | — | — | — | — |
| activation_11 | (Activation) | (None, 5, 25, 512) | 0 | — | — | — | relu |
| 12 conv2d_12 | (Conv2D) | (None, 5, 25, 512) | 2359808 | (3, 3) | (1, 1) | same | — |
| batch_normalization_12 | (BatchNormalization) | (None, 5, 25, 512) | 2048 | — | — | — | — |
| activation_12 | (Activation) | (None, 5, 25, 512) | 0 | — | — | — | relu |
| 13 conv2d_13 | (Conv2D) | (None, 5, 25, 512) | 2359808 | (3, 3) | (1, 1) | same | — |
| batch_normalization_13 | (BatchNormalization) | (None, 5, 25, 512) | 2048 | — | — | — | — |
| activation_13 | (Activation) | (None, 5, 25, 512) | 0 | — | — | — | relu |
| max_pooling2d_5 | (MaxPooling2D) | (None, 2, 12, 512) | 0 | (2, 2) | (2, 2) | valid | — |
| flatten_1 | (Flatten) | (None, 12288) | 0 | — | — | — | — |
| 14 dense_1 | (Dense) | (None, 4096) | 50335744 | — | — | — | relu |
| dropout_1 | (Dropout) | (None, 4096) | 0 | — | — | — | — |
| 15 dense_2 | (Dense) | (None, 4096) | 16781312 | — | — | — | relu |
| dropout_2 | (Dropout) | (None, 4096) | 0 | — | — | — | — |
| 16 dense_3 | (Dense) | (None, 31) | 127007 | — | — | — | softmax |

| | |
|---|---|
| **Total parameters:** | **81,974,495** |
| **Trainable parameters:** | **81,966,047** |
| **Non-trainable parameters:** | **8448** |

Supplementary Table 2.8: DenseNet-40-1D network architecture. Network was implemented using Keras with Tensorflow backend and trained for 10 epochs with 32 batch size. The network architectre was adopted from http://github.com/titu1994/DenseNet.

| Layer | (type) | Output Shape | # Param | Filter size | Stride | Padding | Activation | Connected to |
|---|---|---|---|---|---|---|---|---|
| input_1 | (InputLayer) | (None, 80, 411, 1) | 0 | — | — | — | — | — |
| 1 conv2d_1 | (Conv2D) | (None, 40, 411, 24) | 168 | (7, 1) | (2, 1) | same | — | input_1 |
| batch_normalization_1 | (BatchNormalization) | (None, 40, 411, 24) | 96 | — | — | — | — | conv2d_1 |
| activation_1 | (Activation) | (None, 40, 411, 24) | 0 | — | — | — | — | batch_normalization_1 |
| max_pooling2d_1 | (MaxPooling2D) | (None, 20, 411, 24) | 0 | (3, 1) | (2, 1) | same | — | activation_1 |
| batch_normalization_2 | (BatchNormalization) | (None, 20, 411, 24) | 96 | — | — | — | — | max_pooling2d_1 |
| activation_2 | (Activation) | (None, 20, 411, 24) | 0 | — | — | — | relu | batch_normalization_2 |
| 2 conv2d_2 | (Conv2D) | (None, 20, 411, 12) | 864 | (3, 1) | (3, 1) | same | — | activation_2 |
| concatenate_1 | (Concatenate) | (None, 20, 411, 36) | 0 | — | — | — | — | max_pooling2d_1<br>conv2d_2 |
| batch_normalization_3 | (BatchNormalization) | (None, 20, 411, 36) | 144 | — | — | — | — | concatenate_1 |
| activation_3 | (Activation) | (None, 20, 411, 36) | 0 | — | — | — | relu | batch_normalization_3 |
| 3 conv2d_3 | (Conv2D) | (None, 20, 411, 12) | 1296 | (3, 1) | (3, 1) | same | — | activation_3 |
| concatenate_2 | (Concatenate) | (None, 20, 411, 48) | 0 | — | — | — | — | concatenate_1<br>conv2d_3 |
| batch_normalization_4 | (BatchNormalization) | (None, 20, 411, 48) | 192 | — | — | — | — | concatenate_2 |
| activation_4 | (Activation) | (None, 20, 411, 48) | 0 | — | — | — | relu | batch_normalization_4 |
| 4 conv2d_4 | (Conv2D) | (None, 20, 411, 12) | 1728 | (3, 1) | (3, 1) | same | — | activation_4 |
| concatenate_3 | (Concatenate) | (None, 20, 411, 60) | 0 | — | — | — | — | concatenate_2<br>conv2d_4 |
| batch_normalization_5 | (BatchNormalization) | (None, 20, 411, 60) | 240 | — | — | — | — | concatenate_3 |
| activation_5 | (Activation) | (None, 20, 411, 60) | 0 | — | — | — | relu | batch_normalization_5 |
| 5 conv2d_5 | (Conv2D) | (None, 20, 411, 12) | 2160 | (3, 1) | (3, 1) | same | — | activation_5 |
| concatenate_4 | (Concatenate) | (None, 20, 411, 72) | 0 | — | — | — | — | concatenate_3<br>conv2d_5 |
| batch_normalization_6 | (BatchNormalization) | (None, 20, 411, 72) | 288 | — | — | — | — | concatenate_4 |
| activation_6 | (Activation) | (None, 20, 411, 72) | 0 | — | — | — | relu | batch_normalization_6 |
| 6 conv2d_6 | (Conv2D) | (None, 20, 411, 12) | 2592 | (3, 1) | (3, 1) | same | — | activation_6 |
| concatenate_5 | (Concatenate) | (None, 20, 411, 84) | 0 | — | — | — | — | concatenate_4<br>conv2d_6 |
| batch_normalization_7 | (BatchNormalization) | (None, 20, 411, 84) | 336 | — | — | — | — | concatenate_5 |
| activation_7 | (Activation) | (None, 20, 411, 84) | 0 | — | — | — | relu | batch_normalization_7 |
| 7 conv2d_7 | (Conv2D) | (None, 20, 411, 12) | 3024 | (3, 1) | (3, 1) | same | — | activation_7 |
| concatenate_6 | (Concatenate) | (None, 20, 411, 96) | 0 | — | — | — | — | concatenate_5<br>conv2d_7 |
| batch_normalization_8 | (BatchNormalization) | (None, 20, 411, 96) | 384 | — | — | — | — | concatenate_6 |
| activation_8 | (Activation) | (None, 20, 411, 96) | 0 | — | — | — | relu | batch_normalization_8 |
| 8 conv2d_8 | (Conv2D) | (None, 20, 411, 12) | 3456 | (3, 1) | (3, 1) | same | — | activation_8 |
| concatenate_7 | (Concatenate) | (None, 20, 411, 108) | 0 | — | — | — | — | concatenate_6<br>conv2d_8 |
| batch_normalization_9 | (BatchNormalization) | (None, 20, 411, 108) | 432 | — | — | — | — | concatenate_7 |
| activation_9 | (Activation) | (None, 20, 411, 108) | 0 | — | — | — | relu | batch_normalization_9 |
| 9 conv2d_9 | (Conv2D) | (None, 20, 411, 12) | 3888 | (3, 1) | (3, 1) | same | — | activation_9 |
| concatenate_8 | (Concatenate) | (None, 20, 411, 120) | 0 | — | — | — | — | concatenate_7<br>conv2d_9 |
| batch_normalization_10 | (BatchNormalization) | (None, 20, 411, 120) | 480 | — | — | — | — | concatenate_8 |
| activation_10 | (Activation) | (None, 20, 411, 120) | 0 | — | — | — | relu | batch_normalization_10 |
| 10 conv2d_10 | (Conv2D) | (None, 20, 411, 12) | 4320 | (3, 1) | (3, 1) | same | — | activation_10 |
| concatenate_9 | (Concatenate) | (None, 20, 411, 132) | 0 | — | — | — | — | concatenate_8<br>conv2d_10 |
| batch_normalization_11 | (BatchNormalization) | (None, 20, 411, 132) | 528 | — | — | — | — | concatenate_9 |
| activation_11 | (Activation) | (None, 20, 411, 132) | 0 | — | — | — | relu | batch_normalization_11 |
| 11 conv2d_11 | (Conv2D) | (None, 20, 411, 12) | 4752 | (3, 1) | (3, 1) | same | — | activation_11 |
| concatenate_10 | (Concatenate) | (None, 20, 411, 144) | 0 | — | — | — | — | concatenate_9<br>conv2d_11 |
| batch_normalization_12 | (BatchNormalization) | (None, 20, 411, 144) | 576 | — | — | — | — | concatenate_10 |
| activation_12 | (Activation) | (None, 20, 411, 144) | 0 | — | — | — | relu | batch_normalization_12 |
| 12 conv2d_12 | (Conv2D) | (None, 20, 411, 12) | 5184 | (3, 1) | (3, 1) | same | — | activation_12 |
| concatenate_11 | (Concatenate) | (None, 20, 411, 156) | 0 | — | — | — | — | concatenate_10<br>conv2d_12 |
| batch_normalization_13 | (BatchNormalization) | (None, 20, 411, 156) | 624 | — | — | — | — | concatenate_11 |
| activation_13 | (Activation) | (None, 20, 411, 156) | 0 | — | — | — | relu | batch_normalization_13 |
| 13 conv2d_13 | (Conv2D) | (None, 20, 411, 12) | 5616 | (3, 1) | (3, 1) | same | — | activation_13 |
| concatenate_12 | (Concatenate) | (None, 20, 411, 168) | 0 | — | — | — | — | concatenate_11<br>conv2d_13 |
| batch_normalization_14 | (BatchNormalization) | (None, 20, 411, 168) | 672 | — | — | — | — | concatenate_12 |
| activation_14 | (Activation) | (None, 20, 411, 168) | 0 | — | — | — | relu | batch_normalization_14 |
| 14 conv2d_14 | (Conv2D) | (None, 20, 411, 168) | 28224 | (1, 1) | (1, 1) | same | — | activation_14 |
| average_pooling2d_1 | (AveragePooling2D) | (None, 10, 411, 168) | 0 | (2, 1) | (2, 1) | valid | — | conv2d_14 |
| batch_normalization_15 | (BatchNormalization) | (None, 10, 411, 168) | 672 | — | — | — | — | average_pooling2d_1 |
| activation_15 | (Activation) | (None, 10, 411, 168) | 0 | — | — | — | relu | batch_normalization_15 |

| | | | | | | | | |
|---|---|---|---|---|---|---|---|---|
| 15 conv2d_15 | (Conv2D) | (None, 10, 411, 12) | 6048 | (3, 1) | (3, 1) | same | — | activation_15 |
| concatenate_13 | (Concatenate) | (None, 10, 411, 180) | 0 | — | — | — | — | average_pooling2d_1<br>conv2d_15 |
| batch_normalization_16 | (BatchNormalization) | (None, 10, 411, 180) | 720 | — | — | — | — | concatenate_13 |
| activation_16 | (Activation) | (None, 10, 411, 180) | 0 | — | — | — | relu | batch_normalization_16 |
| 16 conv2d_16 | (Conv2D) | (None, 10, 411, 12) | 6480 | (3, 1) | (3, 1) | same | — | activation_16 |
| concatenate_14 | (Concatenate) | (None, 10, 411, 192) | 0 | — | — | — | — | concatenate_13<br>conv2d_16 |
| batch_normalization_17 | (BatchNormalization) | (None, 10, 411, 192) | 768 | — | — | — | — | concatenate_14 |
| activation_17 | (Activation) | (None, 10, 411, 192) | 0 | — | — | — | relu | batch_normalization_17 |
| 17 conv2d_17 | (Conv2D) | (None, 10, 411, 12) | 6912 | (3, 1) | (3, 1) | same | — | activation_17 |
| concatenate_15 | (Concatenate) | (None, 10, 411, 204) | 0 | — | — | — | — | concatenate_14<br>conv2d_17 |
| batch_normalization_18 | (BatchNormalization) | (None, 10, 411, 204) | 816 | — | — | — | — | concatenate_15 |
| activation_18 | (Activation) | (None, 10, 411, 204) | 0 | — | — | — | relu | batch_normalization_18 |
| 18 conv2d_18 | (Conv2D) | (None, 10, 411, 12) | 7344 | (3, 1) | (3, 1) | same | — | activation_18 |
| concatenate_16 | (Concatenate) | (None, 10, 411, 216) | 0 | — | — | — | — | concatenate_15<br>conv2d_18 |
| batch_normalization_19 | (BatchNormalization) | (None, 10, 411, 216) | 864 | — | — | — | — | concatenate_16 |
| activation_19 | (Activation) | (None, 10, 411, 216) | 0 | — | — | — | relu | batch_normalization_19 |
| 19 conv2d_19 | (Conv2D) | (None, 10, 411, 12) | 7776 | (3, 1) | (3, 1) | same | — | activation_19 |
| concatenate_17 | (Concatenate) | (None, 10, 411, 228) | 0 | — | — | — | — | concatenate_16<br>conv2d_19 |
| batch_normalization_20 | (BatchNormalization) | (None, 10, 411, 228) | 912 | — | — | — | — | concatenate_17 |
| activation_20 | (Activation) | (None, 10, 411, 228) | 0 | — | — | — | relu | batch_normalization_20 |
| 20 conv2d_20 | (Conv2D) | (None, 10, 411, 12) | 8208 | (3, 1) | (3, 1) | same | — | activation_20 |
| concatenate_18 | (Concatenate) | (None, 10, 411, 240) | 0 | — | — | — | — | concatenate_17<br>conv2d_20 |
| batch_normalization_21 | (BatchNormalization) | (None, 10, 411, 240) | 960 | — | — | — | — | concatenate_18 |
| activation_21 | (Activation) | (None, 10, 411, 240) | 0 | — | — | — | relu | batch_normalization_21 |
| 21 conv2d_21 | (Conv2D) | (None, 10, 411, 12) | 8640 | (3, 1) | (3, 1) | same | — | activation_21 |
| concatenate_19 | (Concatenate) | (None, 10, 411, 252) | 0 | — | — | — | — | concatenate_18<br>conv2d_21 |
| batch_normalization_22 | (BatchNormalization) | (None, 10, 411, 252) | 1008 | — | — | — | — | concatenate_19 |
| activation_22 | (Activation) | (None, 10, 411, 252) | 0 | — | — | — | relu | batch_normalization_22 |
| 22 conv2d_22 | (Conv2D) | (None, 10, 411, 12) | 9072 | (3, 1) | (3, 1) | same | — | activation_22 |
| concatenate_20 | (Concatenate) | (None, 10, 411, 264) | 0 | — | — | — | — | concatenate_19<br>conv2d_22 |
| batch_normalization_23 | (BatchNormalization) | (None, 10, 411, 264) | 1056 | — | — | — | — | concatenate_20 |
| activation_23 | (Activation) | (None, 10, 411, 264) | 0 | — | — | — | relu | batch_normalization_23 |
| 23 conv2d_23 | (Conv2D) | (None, 10, 411, 12) | 9504 | (3, 1) | (3, 1) | same | — | activation_23 |
| concatenate_21 | (Concatenate) | (None, 10, 411, 276) | 0 | — | — | — | — | concatenate_20<br>conv2d_23 |
| batch_normalization_24 | (BatchNormalization) | (None, 10, 411, 276) | 1104 | — | — | — | — | concatenate_21 |
| activation_24 | (Activation) | (None, 10, 411, 276) | 0 | — | — | — | relu | batch_normalization_24 |
| 24 conv2d_24 | (Conv2D) | (None, 10, 411, 12) | 9936 | (3, 1) | (3, 1) | same | — | activation_24 |
| concatenate_22 | (Concatenate) | (None, 10, 411, 288) | 0 | — | — | — | — | concatenate_21<br>conv2d_24 |
| batch_normalization_25 | (BatchNormalization) | (None, 10, 411, 288) | 1152 | — | — | — | — | concatenate_22 |
| activation_25 | (Activation) | (None, 10, 411, 288) | 0 | — | — | — | relu | batch_normalization_25 |
| 25 conv2d_25 | (Conv2D) | (None, 10, 411, 12) | 10368 | (3, 1) | (3, 1) | same | — | activation_25 |
| concatenate_23 | (Concatenate) | (None, 10, 411, 300) | 0 | — | — | — | — | concatenate_22<br>conv2d_25 |
| batch_normalization_26 | (BatchNormalization) | (None, 10, 411, 300) | 1200 | — | — | — | — | concatenate_23 |
| activation_26 | (Activation) | (None, 10, 411, 300) | 0 | — | — | — | relu | batch_normalization_26 |
| 26 conv2d_26 | (Conv2D) | (None, 10, 411, 12) | 10800 | (3, 1) | (3, 1) | same | — | activation_26 |
| concatenate_24 | (Concatenate) | (None, 10, 411, 312) | 0 | — | — | — | — | concatenate_23<br>conv2d_26 |
| batch_normalization_27 | (BatchNormalization) | (None, 10, 411, 312) | 1248 | — | — | — | — | concatenate_24 |
| activation_27 | (Activation) | (None, 10, 411, 312) | 0 | — | — | — | relu | batch_normalization_27 |
| 27 conv2d_27 | (Conv2D) | (None, 10, 411, 312) | 97344 | (1, 1) | (1, 1) | same | — | activation_27 |
| average_pooling2d_2 | (AveragePooling2D) | (None, 5, 411, 312) | 0 | (2, 1) | (2, 1) | valid | — | conv2d_27 |
| batch_normalization_28 | (BatchNormalization) | (None, 5, 411, 312) | 1248 | — | — | — | — | average_pooling2d_2 |
| activation_28 | (Activation) | (None, 5, 411, 312) | 0 | — | — | — | relu | batch_normalization_28 |
| 28 conv2d_28 | (Conv2D) | (None, 5, 411, 12) | 11232 | (3, 1) | (3, 1) | same | — | activation_28 |
| concatenate_25 | (Concatenate) | (None, 5, 411, 324) | 0 | — | — | — | — | average_pooling2d_2<br>conv2d_28 |
| batch_normalization_29 | (BatchNormalization) | (None, 5, 411, 324) | 1296 | — | — | — | — | concatenate_25 |
| activation_29 | (Activation) | (None, 5, 411, 324) | 0 | — | — | — | relu | batch_normalization_29 |
| 29 conv2d_29 | (Conv2D) | (None, 5, 411, 12) | 11664 | (3, 1) | (3, 1) | same | — | activation_29 |
| concatenate_26 | (Concatenate) | (None, 5, 411, 336) | 0 | — | — | — | — | concatenate_25<br>conv2d_29 |

| | | | | | | | | | |
|---|---|---|---|---|---|---|---|---|---|
| | batch_normalization_30 | (BatchNormalization) | (None, 5, 411, 336) | 1344 | — | — | — | — | concatenate_26 |
| | activation_30 | (Activation) | (None, 5, 411, 336) | 0 | — | — | — | relu | batch_normalization_30 |
| 30 | conv2d_30 | (Conv2D) | (None, 5, 411, 12) | 12096 | (3, 1) | (3, 1) | same | — | activation_30 |
| | concatenate_27 | (Concatenate) | (None, 5, 411, 348) | 0 | — | — | — | — | concatenate_26<br>conv2d_30 |
| | batch_normalization_31 | (BatchNormalization) | (None, 5, 411, 348) | 1392 | — | — | — | — | concatenate_27 |
| | activation_31 | (Activation) | (None, 5, 411, 348) | 0 | — | — | — | relu | batch_normalization_31 |
| 31 | conv2d_31 | (Conv2D) | (None, 5, 411, 12) | 12528 | (3, 1) | (3, 1) | same | — | activation_31 |
| | concatenate_28 | (Concatenate) | (None, 5, 411, 360) | 0 | — | — | — | — | concatenate_27<br>conv2d_31 |
| | batch_normalization_32 | (BatchNormalization) | (None, 5, 411, 360) | 1440 | — | — | — | — | concatenate_28 |
| | activation_32 | (Activation) | (None, 5, 411, 360) | 0 | — | — | — | relu | batch_normalization_32 |
| 32 | conv2d_32 | (Conv2D) | (None, 5, 411, 12) | 12960 | (3, 1) | (3, 1) | same | — | activation_32 |
| | concatenate_29 | (Concatenate) | (None, 5, 411, 372) | 0 | — | — | — | — | concatenate_28<br>conv2d_32 |
| | batch_normalization_33 | (BatchNormalization) | (None, 5, 411, 372) | 1488 | — | — | — | — | concatenate_29 |
| | activation_33 | (Activation) | (None, 5, 411, 372) | 0 | — | — | — | relu | batch_normalization_33 |
| 33 | conv2d_33 | (Conv2D) | (None, 5, 411, 12) | 13392 | (3, 1) | (3, 1) | same | — | activation_33 |
| | concatenate_30 | (Concatenate) | (None, 5, 411, 384) | 0 | — | — | — | — | concatenate_29<br>conv2d_33 |
| | batch_normalization_34 | (BatchNormalization) | (None, 5, 411, 384) | 1536 | — | — | — | — | concatenate_30 |
| | activation_34 | (Activation) | (None, 5, 411, 384) | 0 | — | — | — | relu | batch_normalization_34 |
| 34 | conv2d_34 | (Conv2D) | (None, 5, 411, 12) | 13824 | (3, 1) | (3, 1) | same | — | activation_34 |
| | concatenate_31 | (Concatenate) | (None, 5, 411, 396) | 0 | — | — | — | — | concatenate_30<br>conv2d_34 |
| | batch_normalization_35 | (BatchNormalization) | (None, 5, 411, 396) | 1584 | — | — | — | — | concatenate_31 |
| | activation_35 | (Activation) | (None, 5, 411, 396) | 0 | — | — | — | relu | batch_normalization_35 |
| 35 | conv2d_35 | (Conv2D) | (None, 5, 411, 12) | 14256 | (3, 1) | (3, 1) | same | — | activation_35 |
| | concatenate_32 | (Concatenate) | (None, 5, 411, 408) | 0 | — | — | — | — | concatenate_31<br>conv2d_35 |
| | batch_normalization_36 | (BatchNormalization) | (None, 5, 411, 408) | 1632 | — | — | — | — | concatenate_32 |
| | activation_36 | (Activation) | (None, 5, 411, 408) | 0 | — | — | — | relu | batch_normalization_36 |
| 36 | conv2d_36 | (Conv2D) | (None, 5, 411, 12) | 14688 | (3, 1) | (3, 1) | same | — | activation_36 |
| | concatenate_33 | (Concatenate) | (None, 5, 411, 420) | 0 | — | — | — | — | concatenate_32<br>conv2d_36 |
| | batch_normalization_37 | (BatchNormalization) | (None, 5, 411, 420) | 1680 | — | — | — | — | concatenate_33 |
| | activation_37 | (Activation) | (None, 5, 411, 420) | 0 | — | — | — | relu | batch_normalization_37 |
| 37 | conv2d_37 | (Conv2D) | (None, 5, 411, 12) | 15120 | (3, 1) | (3, 1) | same | — | activation_37 |
| | concatenate_34 | (Concatenate) | (None, 5, 411, 432) | 0 | — | — | — | — | concatenate_33<br>conv2d_37 |
| | batch_normalization_38 | (BatchNormalization) | (None, 5, 411, 432) | 1728 | — | — | — | — | concatenate_34 |
| | activation_38 | (Activation) | (None, 5, 411, 432) | 0 | — | — | — | relu | batch_normalization_38 |
| 38 | conv2d_38 | (Conv2D) | (None, 5, 411, 12) | 15552 | (3, 1) | (3, 1) | same | — | activation_38 |
| | concatenate_35 | (Concatenate) | (None, 5, 411, 444) | 0 | — | — | — | — | concatenate_34<br>conv2d_38 |
| | batch_normalization_39 | (BatchNormalization) | (None, 5, 411, 444) | 1776 | — | — | — | — | concatenate_35 |
| | activation_39 | (Activation) | (None, 5, 411, 444) | 0 | — | — | — | relu | batch_normalization_39 |
| 39 | conv2d_39 | (Conv2D) | (None, 5, 411, 12) | 15984 | (3, 1) | (3, 1) | same | — | activation_39 |
| | concatenate_36 | (Concatenate) | (None, 5, 411, 456) | 0 | — | — | — | — | concatenate_35<br>conv2d_39 |
| | batch_normalization_40 | (BatchNormalization) | (None, 5, 411, 456) | 1824 | — | — | — | — | concatenate_36 |
| | activation_40 | (Activation) | (None, 5, 411, 456) | 0 | — | — | — | relu | batch_normalization_40 |
| | average_pooling2d_3 | (AveragePooling2D) | (None, 1, 411, 456) | 0 | (5, 1) | (5, 1) | valid | — | activation_40 |
| | flatten_1 | (Flatten) | (None, 187416) | 0 | — | — | — | — | average_pooling2d_3 |
| 40 | dense_1 | (Dense) | (None, 31) | 5809927 | — | — | — | softmax | flatten_1 |

| | |
|---|---|
| **Total parameters:** | **6,276,463** |
| **Trainable parameters:** | **6,257,695** |
| **Non-trainable parameters:** | **18768** |

Supplementary Table 2.9: DenseNet-40-2D network architecture. Network was implemented using Keras with Tensorflow backend and trained for 10 epochs with 32 batch size. The network architectre was adopted from http://github.com/titu1994/DenseNet.

| | Layer | (type) | Output Shape | # Param | Filter size | Stride | Padding | Activation | Connected to |
|---|---|---|---|---|---|---|---|---|---|
| | input_1 | (InputLayer) | (None, 80, 411, 1) | 0 | — | — | — | — | — |
| 1 | conv2d_1 | (Conv2D) | (None, 40, 206, 24) | 1176 | (7, 7) | (2, 2) | same | — | input_1 |
| | batch_normalization_1 | (BatchNormalization) | (None, 40, 206, 24) | 96 | — | — | — | — | conv2d_1 |
| | activation_1 | (Activation) | (None, 40, 206, 24) | 0 | — | — | — | — | batch_normalization_1 |
| | max_pooling2d_1 | (MaxPooling2D) | (None, 20, 103, 24) | 0 | (3, 3) | (2, 2) | same | — | activation_1 |
| | batch_normalization_2 | (BatchNormalization) | (None, 20, 103, 24) | 96 | — | — | — | — | max_pooling2d_1 |
| | activation_2 | (Activation) | (None, 20, 103, 24) | 0 | — | — | — | relu | batch_normalization_2 |
| 2 | conv2d_2 | (Conv2D) | (None, 20, 103, 12) | 2592 | (3, 3) | (3, 3) | same | — | activation_2 |
| | concatenate_1 | (Concatenate) | (None, 20, 103, 36) | 0 | — | — | — | — | max_pooling2d_1<br>conv2d_2 |
| | batch_normalization_3 | (BatchNormalization) | (None, 20, 103, 36) | 144 | — | — | — | — | concatenate_1 |
| | activation_3 | (Activation) | (None, 20, 103, 36) | 0 | — | — | — | relu | batch_normalization_3 |
| 3 | conv2d_3 | (Conv2D) | (None, 20, 103, 12) | 3888 | (3, 3) | (3, 3) | same | — | activation_3 |
| | concatenate_2 | (Concatenate) | (None, 20, 103, 48) | 0 | — | — | — | — | concatenate_1<br>conv2d_3 |
| | batch_normalization_4 | (BatchNormalization) | (None, 20, 103, 48) | 192 | — | — | — | — | concatenate_2 |
| | activation_4 | (Activation) | (None, 20, 103, 48) | 0 | — | — | — | relu | batch_normalization_4 |
| 4 | conv2d_4 | (Conv2D) | (None, 20, 103, 12) | 5184 | (3, 3) | (3, 3) | same | — | activation_4 |
| | concatenate_3 | (Concatenate) | (None, 20, 103, 60) | 0 | — | — | — | — | concatenate_2<br>conv2d_4 |
| | batch_normalization_5 | (BatchNormalization) | (None, 20, 103, 60) | 240 | — | — | — | — | concatenate_3 |
| | activation_5 | (Activation) | (None, 20, 103, 60) | 0 | — | — | — | relu | batch_normalization_5 |
| 5 | conv2d_5 | (Conv2D) | (None, 20, 103, 12) | 6480 | (3, 3) | (3, 3) | same | — | activation_5 |
| | concatenate_4 | (Concatenate) | (None, 20, 103, 72) | 0 | — | — | — | — | concatenate_3<br>conv2d_5 |
| | batch_normalization_6 | (BatchNormalization) | (None, 20, 103, 72) | 288 | — | — | — | — | concatenate_4 |
| | activation_6 | (Activation) | (None, 20, 103, 72) | 0 | — | — | — | relu | batch_normalization_6 |
| 6 | conv2d_6 | (Conv2D) | (None, 20, 103, 12) | 7776 | (3, 3) | (3, 3) | same | — | activation_6 |
| | concatenate_5 | (Concatenate) | (None, 20, 103, 84) | 0 | — | — | — | — | concatenate_4<br>conv2d_6 |
| | batch_normalization_7 | (BatchNormalization) | (None, 20, 103, 84) | 336 | — | — | — | — | concatenate_5 |
| | activation_7 | (Activation) | (None, 20, 103, 84) | 0 | — | — | — | relu | batch_normalization_7 |
| 7 | conv2d_7 | (Conv2D) | (None, 20, 103, 12) | 9072 | (3, 3) | (3, 3) | same | — | activation_7 |
| | concatenate_6 | (Concatenate) | (None, 20, 103, 96) | 0 | — | — | — | — | concatenate_5<br>conv2d_7 |
| | batch_normalization_8 | (BatchNormalization) | (None, 20, 103, 96) | 384 | — | — | — | — | concatenate_6 |
| | activation_8 | (Activation) | (None, 20, 103, 96) | 0 | — | — | — | relu | batch_normalization_8 |
| 8 | conv2d_8 | (Conv2D) | (None, 20, 103, 12) | 10368 | (3, 3) | (3, 3) | same | — | activation_8 |
| | concatenate_7 | (Concatenate) | (None, 20, 103, 108) | 0 | — | — | — | — | concatenate_6<br>conv2d_8 |
| | batch_normalization_9 | (BatchNormalization) | (None, 20, 103, 108) | 432 | — | — | — | — | concatenate_7 |
| | activation_9 | (Activation) | (None, 20, 103, 108) | 0 | — | — | — | relu | batch_normalization_9 |
| 9 | conv2d_9 | (Conv2D) | (None, 20, 103, 12) | 11664 | (3, 3) | (3, 3) | same | — | activation_9 |
| | concatenate_8 | (Concatenate) | (None, 20, 103, 120) | 0 | — | — | — | — | concatenate_7<br>conv2d_9 |
| | batch_normalization_10 | (BatchNormalization) | (None, 20, 103, 120) | 480 | — | — | — | — | concatenate_8 |
| | activation_10 | (Activation) | (None, 20, 103, 120) | 0 | — | — | — | relu | batch_normalization_10 |
| 10 | conv2d_10 | (Conv2D) | (None, 20, 103, 12) | 12960 | (3, 3) | (3, 3) | same | — | activation_10 |
| | concatenate_9 | (Concatenate) | (None, 20, 103, 132) | 0 | — | — | — | — | concatenate_8<br>conv2d_10 |
| | batch_normalization_11 | (BatchNormalization) | (None, 20, 103, 132) | 528 | — | — | — | — | concatenate_9 |
| | activation_11 | (Activation) | (None, 20, 103, 132) | 0 | — | — | — | relu | batch_normalization_11 |
| 11 | conv2d_11 | (Conv2D) | (None, 20, 103, 12) | 14256 | (3, 3) | (3, 3) | same | — | activation_11 |
| | concatenate_10 | (Concatenate) | (None, 20, 103, 144) | 0 | — | — | — | — | concatenate_9<br>conv2d_11 |
| | batch_normalization_12 | (BatchNormalization) | (None, 20, 103, 144) | 576 | — | — | — | — | concatenate_10 |
| | activation_12 | (Activation) | (None, 20, 103, 144) | 0 | — | — | — | relu | batch_normalization_12 |
| 12 | conv2d_12 | (Conv2D) | (None, 20, 103, 12) | 15552 | (3, 3) | (3, 3) | same | — | activation_12 |
| | concatenate_11 | (Concatenate) | (None, 20, 103, 156) | 0 | — | — | — | — | concatenate_10<br>conv2d_12 |
| | batch_normalization_13 | (BatchNormalization) | (None, 20, 103, 156) | 624 | — | — | — | — | concatenate_11 |
| | activation_13 | (Activation) | (None, 20, 103, 156) | 0 | — | — | — | relu | batch_normalization_13 |
| 13 | conv2d_13 | (Conv2D) | (None, 20, 103, 12) | 16848 | (3, 3) | (3, 3) | same | — | activation_13 |
| | concatenate_12 | (Concatenate) | (None, 20, 103, 168) | 0 | — | — | — | — | concatenate_11<br>conv2d_13 |
| | batch_normalization_14 | (BatchNormalization) | (None, 20, 103, 168) | 672 | — | — | — | — | concatenate_12 |
| | activation_14 | (Activation) | (None, 20, 103, 168) | 0 | — | — | — | relu | batch_normalization_14 |
| 14 | conv2d_14 | (Conv2D) | (None, 20, 103, 168) | 28224 | (1, 1) | (1, 1) | same | — | activation_14 |
| | average_pooling2d_1 | (AveragePooling2D) | (None, 10, 51, 168) | 0 | (2, 2) | (2, 2) | valid | — | conv2d_14 |
| | batch_normalization_15 | (BatchNormalization) | (None, 10, 51, 168) | 672 | — | — | — | — | average_pooling2d_1 |
| | activation_15 | (Activation) | (None, 10, 51, 168) | 0 | — | — | — | relu | batch_normalization_15 |

| | | | | | | | | |
|---|---|---|---|---|---|---|---|---|
| 15 conv2d_15 | (Conv2D) | (None, 10, 51, 12) | 18144 | (3, 3) | (3, 3) | same | — | activation_15 |
| concatenate_13 | (Concatenate) | (None, 10, 51, 180) | 0 | — | — | — | — | average_pooling2d_1<br>conv2d_15 |
| batch_normalization_16 | (BatchNormalization) | (None, 10, 51, 180) | 720 | — | — | — | — | concatenate_13 |
| activation_16 | (Activation) | (None, 10, 51, 180) | 0 | — | — | — | relu | batch_normalization_16 |
| 16 conv2d_16 | (Conv2D) | (None, 10, 51, 12) | 19440 | (3, 3) | (3, 3) | same | — | activation_16 |
| concatenate_14 | (Concatenate) | (None, 10, 51, 192) | 0 | — | — | — | — | concatenate_13<br>conv2d_16 |
| batch_normalization_17 | (BatchNormalization) | (None, 10, 51, 192) | 768 | — | — | — | — | concatenate_14 |
| activation_17 | (Activation) | (None, 10, 51, 192) | 0 | — | — | — | relu | batch_normalization_17 |
| 17 conv2d_17 | (Conv2D) | (None, 10, 51, 12) | 20736 | (3, 3) | (3, 3) | same | — | activation_17 |
| concatenate_15 | (Concatenate) | (None, 10, 51, 204) | 0 | — | — | — | — | concatenate_14<br>conv2d_17 |
| batch_normalization_18 | (BatchNormalization) | (None, 10, 51, 204) | 816 | — | — | — | — | concatenate_15 |
| activation_18 | (Activation) | (None, 10, 51, 204) | 0 | — | — | — | relu | batch_normalization_18 |
| 18 conv2d_18 | (Conv2D) | (None, 10, 51, 12) | 22032 | (3, 3) | (3, 3) | same | — | activation_18 |
| concatenate_16 | (Concatenate) | (None, 10, 51, 216) | 0 | — | — | — | — | concatenate_15<br>conv2d_18 |
| batch_normalization_19 | (BatchNormalization) | (None, 10, 51, 216) | 864 | — | — | — | — | concatenate_16 |
| activation_19 | (Activation) | (None, 10, 51, 216) | 0 | — | — | — | relu | batch_normalization_19 |
| 19 conv2d_19 | (Conv2D) | (None, 10, 51, 12) | 23328 | (3, 3) | (3, 3) | same | — | activation_19 |
| concatenate_17 | (Concatenate) | (None, 10, 51, 228) | 0 | — | — | — | — | concatenate_16<br>conv2d_19 |
| batch_normalization_20 | (BatchNormalization) | (None, 10, 51, 228) | 912 | — | — | — | — | concatenate_17 |
| activation_20 | (Activation) | (None, 10, 51, 228) | 0 | — | — | — | relu | batch_normalization_20 |
| 20 conv2d_20 | (Conv2D) | (None, 10, 51, 12) | 24624 | (3, 3) | (3, 3) | same | — | activation_20 |
| concatenate_18 | (Concatenate) | (None, 10, 51, 240) | 0 | — | — | — | — | concatenate_17<br>conv2d_20 |
| batch_normalization_21 | (BatchNormalization) | (None, 10, 51, 240) | 960 | — | — | — | — | concatenate_18 |
| activation_21 | (Activation) | (None, 10, 51, 240) | 0 | — | — | — | relu | batch_normalization_21 |
| 21 conv2d_21 | (Conv2D) | (None, 10, 51, 12) | 25920 | (3, 3) | (3, 3) | same | — | activation_21 |
| concatenate_19 | (Concatenate) | (None, 10, 51, 252) | 0 | — | — | — | — | concatenate_18<br>conv2d_21 |
| batch_normalization_22 | (BatchNormalization) | (None, 10, 51, 252) | 1008 | — | — | — | — | concatenate_19 |
| activation_22 | (Activation) | (None, 10, 51, 252) | 0 | — | — | — | relu | batch_normalization_22 |
| 22 conv2d_22 | (Conv2D) | (None, 10, 51, 12) | 27216 | (3, 3) | (3, 3) | same | — | activation_22 |
| concatenate_20 | (Concatenate) | (None, 10, 51, 264) | 0 | — | — | — | — | concatenate_19<br>conv2d_22 |
| batch_normalization_23 | (BatchNormalization) | (None, 10, 51, 264) | 1056 | — | — | — | — | concatenate_20 |
| activation_23 | (Activation) | (None, 10, 51, 264) | 0 | — | — | — | relu | batch_normalization_23 |
| 23 conv2d_23 | (Conv2D) | (None, 10, 51, 12) | 28512 | (3, 3) | (3, 3) | same | — | activation_23 |
| concatenate_21 | (Concatenate) | (None, 10, 51, 276) | 0 | — | — | — | — | concatenate_20<br>conv2d_23 |
| batch_normalization_24 | (BatchNormalization) | (None, 10, 51, 276) | 1104 | — | — | — | — | concatenate_21 |
| activation_24 | (Activation) | (None, 10, 51, 276) | 0 | — | — | — | relu | batch_normalization_24 |
| 24 conv2d_24 | (Conv2D) | (None, 10, 51, 12) | 29808 | (3, 3) | (3, 3) | same | — | activation_24 |
| concatenate_22 | (Concatenate) | (None, 10, 51, 288) | 0 | — | — | — | — | concatenate_21<br>conv2d_24 |
| batch_normalization_25 | (BatchNormalization) | (None, 10, 51, 288) | 1152 | — | — | — | — | concatenate_22 |
| activation_25 | (Activation) | (None, 10, 51, 288) | 0 | — | — | — | relu | batch_normalization_25 |
| 25 conv2d_25 | (Conv2D) | (None, 10, 51, 12) | 31104 | (3, 3) | (3, 3) | same | — | activation_25 |
| concatenate_23 | (Concatenate) | (None, 10, 51, 300) | 0 | — | — | — | — | concatenate_22<br>conv2d_25 |
| batch_normalization_26 | (BatchNormalization) | (None, 10, 51, 300) | 1200 | — | — | — | — | concatenate_23 |
| activation_26 | (Activation) | (None, 10, 51, 300) | 0 | — | — | — | relu | batch_normalization_26 |
| 26 conv2d_26 | (Conv2D) | (None, 10, 51, 12) | 32400 | (3, 3) | (3, 3) | same | — | activation_26 |
| concatenate_24 | (Concatenate) | (None, 10, 51, 312) | 0 | — | — | — | — | concatenate_23<br>conv2d_26 |
| batch_normalization_27 | (BatchNormalization) | (None, 10, 51, 312) | 1248 | — | — | — | — | concatenate_24 |
| activation_27 | (Activation) | (None, 10, 51, 312) | 0 | — | — | — | relu | batch_normalization_27 |
| 27 conv2d_27 | (Conv2D) | (None, 10, 51, 312) | 97344 | (1, 1) | (1, 1) | same | — | activation_27 |
| average_pooling2d_2 | (AveragePooling2D) | (None, 5, 25, 312) | 0 | (2, 2) | (2, 2) | valid | — | conv2d_27 |
| batch_normalization_28 | (BatchNormalization) | (None, 5, 25, 312) | 1248 | — | — | — | — | average_pooling2d_2 |
| activation_28 | (Activation) | (None, 5, 25, 312) | 0 | — | — | — | relu | batch_normalization_28 |
| 28 conv2d_28 | (Conv2D) | (None, 5, 25, 12) | 33696 | (3, 3) | (3, 3) | same | — | activation_28 |
| concatenate_25 | (Concatenate) | (None, 5, 25, 324) | 0 | — | — | — | — | average_pooling2d_2<br>conv2d_28 |
| batch_normalization_29 | (BatchNormalization) | (None, 5, 25, 324) | 1296 | — | — | — | — | concatenate_25 |
| activation_29 | (Activation) | (None, 5, 25, 324) | 0 | — | — | — | relu | batch_normalization_29 |
| 29 conv2d_29 | (Conv2D) | (None, 5, 25, 12) | 34992 | (3, 3) | (3, 3) | same | — | activation_29 |
| concatenate_26 | (Concatenate) | (None, 5, 25, 336) | 0 | — | — | — | — | concatenate_25<br>conv2d_29 |

| | | | | | | | | | |
|---|---|---|---|---|---|---|---|---|---|
| | batch_normalization_30 | (BatchNormalization) | (None, 5, 25, 336) | 1344 | — | — | — | — | concatenate_26 |
| | activation_30 | (Activation) | (None, 5, 25, 336) | 0 | — | — | — | relu | batch_normalization_30 |
| 30 | conv2d_30 | (Conv2D) | (None, 5, 25, 12) | 36288 | (3, 3) | (3, 3) | same | — | activation_30 |
| | concatenate_27 | (Concatenate) | (None, 5, 25, 348) | 0 | — | — | — | — | concatenate_26<br>conv2d_30 |
| | batch_normalization_31 | (BatchNormalization) | (None, 5, 25, 348) | 1392 | — | — | — | — | concatenate_27 |
| | activation_31 | (Activation) | (None, 5, 25, 348) | 0 | — | — | — | relu | batch_normalization_31 |
| 31 | conv2d_31 | (Conv2D) | (None, 5, 25, 12) | 37584 | (3, 3) | (3, 3) | same | — | activation_31 |
| | concatenate_28 | (Concatenate) | (None, 5, 25, 360) | 0 | — | — | — | — | concatenate_27<br>conv2d_31 |
| | batch_normalization_32 | (BatchNormalization) | (None, 5, 25, 360) | 1440 | — | — | — | — | concatenate_28 |
| | activation_32 | (Activation) | (None, 5, 25, 360) | 0 | — | — | — | relu | batch_normalization_32 |
| 32 | conv2d_32 | (Conv2D) | (None, 5, 25, 12) | 38880 | (3, 3) | (3, 3) | same | — | activation_32 |
| | concatenate_29 | (Concatenate) | (None, 5, 25, 372) | 0 | — | — | — | — | concatenate_28<br>conv2d_32 |
| | batch_normalization_33 | (BatchNormalization) | (None, 5, 25, 372) | 1488 | — | — | — | — | concatenate_29 |
| | activation_33 | (Activation) | (None, 5, 25, 372) | 0 | — | — | — | relu | batch_normalization_33 |
| 33 | conv2d_33 | (Conv2D) | (None, 5, 25, 12) | 40176 | (3, 3) | (3, 3) | same | — | activation_33 |
| | concatenate_30 | (Concatenate) | (None, 5, 25, 384) | 0 | — | — | — | — | concatenate_29<br>conv2d_33 |
| | batch_normalization_34 | (BatchNormalization) | (None, 5, 25, 384) | 1536 | — | — | — | — | concatenate_30 |
| | activation_34 | (Activation) | (None, 5, 25, 384) | 0 | — | — | — | relu | batch_normalization_34 |
| 34 | conv2d_34 | (Conv2D) | (None, 5, 25, 12) | 41472 | (3, 3) | (3, 3) | same | — | activation_34 |
| | concatenate_31 | (Concatenate) | (None, 5, 25, 396) | 0 | — | — | — | — | concatenate_30<br>conv2d_34 |
| | batch_normalization_35 | (BatchNormalization) | (None, 5, 25, 396) | 1584 | — | — | — | — | concatenate_31 |
| | activation_35 | (Activation) | (None, 5, 25, 396) | 0 | — | — | — | relu | batch_normalization_35 |
| 35 | conv2d_35 | (Conv2D) | (None, 5, 25, 12) | 42768 | (3, 3) | (3, 3) | same | — | activation_35 |
| | concatenate_32 | (Concatenate) | (None, 5, 25, 408) | 0 | — | — | — | — | concatenate_31<br>conv2d_35 |
| | batch_normalization_36 | (BatchNormalization) | (None, 5, 25, 408) | 1632 | — | — | — | — | concatenate_32 |
| | activation_36 | (Activation) | (None, 5, 25, 408) | 0 | — | — | — | relu | batch_normalization_36 |
| 36 | conv2d_36 | (Conv2D) | (None, 5, 25, 12) | 44064 | (3, 3) | (3, 3) | same | — | activation_36 |
| | concatenate_33 | (Concatenate) | (None, 5, 25, 420) | 0 | — | — | — | — | concatenate_32<br>conv2d_36 |
| | batch_normalization_37 | (BatchNormalization) | (None, 5, 25, 420) | 1680 | — | — | — | — | concatenate_33 |
| | activation_37 | (Activation) | (None, 5, 25, 420) | 0 | — | — | — | relu | batch_normalization_37 |
| 37 | conv2d_37 | (Conv2D) | (None, 5, 25, 12) | 45360 | (3, 3) | (3, 3) | same | — | activation_37 |
| | concatenate_34 | (Concatenate) | (None, 5, 25, 432) | 0 | — | — | — | — | concatenate_33<br>conv2d_37 |
| | batch_normalization_38 | (BatchNormalization) | (None, 5, 25, 432) | 1728 | — | — | — | — | concatenate_34 |
| | activation_38 | (Activation) | (None, 5, 25, 432) | 0 | — | — | — | relu | batch_normalization_38 |
| 38 | conv2d_38 | (Conv2D) | (None, 5, 25, 12) | 46656 | (3, 3) | (3, 3) | same | — | activation_38 |
| | concatenate_35 | (Concatenate) | (None, 5, 25, 444) | 0 | — | — | — | — | concatenate_34<br>conv2d_38 |
| | batch_normalization_39 | (BatchNormalization) | (None, 5, 25, 444) | 1776 | — | — | — | — | concatenate_35 |
| | activation_39 | (Activation) | (None, 5, 25, 444) | 0 | — | — | — | relu | batch_normalization_39 |
| 39 | conv2d_39 | (Conv2D) | (None, 5, 25, 12) | 47952 | (3, 3) | (3, 3) | same | — | activation_39 |
| | concatenate_36 | (Concatenate) | (None, 5, 25, 456) | 0 | — | — | — | — | concatenate_35<br>conv2d_39 |
| | batch_normalization_40 | (BatchNormalization) | (None, 5, 25, 456) | 1824 | — | — | — | — | concatenate_36 |
| | activation_40 | (Activation) | (None, 5, 25, 456) | 0 | — | — | — | relu | batch_normalization_40 |
| | global_average_pooling2d_1 | (GlobalAveragePooling2D) | (None, 456) | 0 | (5, 5) | (5, 5) | valid | — | activation_40 |
| 40 | dense_1 | (Dense) | (None, 31) | 14167 | — | — | — | softmax | global_average_pooling2d_1 |

| | |
|---|---|
| **Total parameters:** | **1,088,239** |
| **Trainable parameters:** | **1,069,471** |
| **Non-trainable parameters:** | **18768** |

Supplementary Table 2.10: ResNet-34-1D network architecture. Network was implemented using Keras with Tensorflow backend and trained for 10 epochs with 32 batch size. The network architectre was adopted from https://github.com/keras-team/keras-contrib/blob/master/keras_contrib/applications/resnet.py

| Layer | (type) | Output Shape | # Param | Filter size | Stride | Padding | Activation | Connected to |
|---|---|---|---|---|---|---|---|---|
| input_1 | (InputLayer) | (None, 80, 411, 1) | 0 | — | — | — | — | — |
| 1 conv2d_1 | (Conv2D) | (None, 40, 411, 64) | 512 | (7, 1) | (2, 1) | same | — | input_1 |
| batch_normalization_1 | (BatchNormalization) | (None, 40, 411, 64) | 256 | — | — | — | — | conv2d_1 |
| activation_1 | (Activation) | (None, 40, 411, 64) | 0 | — | — | — | relu | batch_normalization_1 |
| max_pooling2d_1 | (MaxPooling2D) | (None, 20, 411, 64) | 0 | (3, 1) | (2, 1) | same | — | activation_1 |
| 2 res0a_branch2a | (Conv2D) | (None, 20, 411, 64) | 12352 | (3, 1) | (1, 1) | same | — | max_pooling2d_1 |
| batch_normalization_2 | (BatchNormalization) | (None, 20, 411, 64) | 256 | — | — | — | — | res0a_branch2a |
| activation_2 | (Activation) | (None, 20, 411, 64) | 0 | — | — | — | relu | batch_normalization_2 |
| 3 conv2d_2 | (Conv2D) | (None, 20, 411, 64) | 12352 | (3, 1) | (1, 1) | same | — | activation_2 |
| add_1 | (Add) | (None, 20, 411, 64) | 0 | — | — | — | — | max_pooling2d_1<br>conv2d_2 |
| batch_normalization_3 | (BatchNormalization) | (None, 20, 411, 64) | 256 | — | — | — | — | add_1 |
| activation_3 | (Activation) | (None, 20, 411, 64) | 0 | — | — | — | relu | batch_normalization_3 |
| 4 conv2d_3 | (Conv2D) | (None, 20, 411, 64) | 12352 | (3, 1) | (1, 1) | same | — | activation_3 |
| batch_normalization_4 | (BatchNormalization) | (None, 20, 411, 64) | 256 | — | — | — | — | conv2d_3 |
| activation_4 | (Activation) | (None, 20, 411, 64) | 0 | — | — | — | relu | batch_normalization_4 |
| 5 conv2d_4 | (Conv2D) | (None, 20, 411, 64) | 12352 | (3, 1) | (1, 1) | same | — | activation_4 |
| add_2 | (Add) | (None, 20, 411, 64) | 0 | — | — | — | — | add_1<br>conv2d_4 |
| batch_normalization_5 | (BatchNormalization) | (None, 20, 411, 64) | 256 | — | — | — | — | add_2 |
| activation_5 | (Activation) | (None, 20, 411, 64) | 0 | — | — | — | relu | batch_normalization_5 |
| 6 conv2d_5 | (Conv2D) | (None, 20, 411, 64) | 12352 | (3, 1) | (1, 1) | same | — | activation_5 |
| batch_normalization_6 | (BatchNormalization) | (None, 20, 411, 64) | 256 | — | — | — | — | conv2d_5 |
| activation_6 | (Activation) | (None, 20, 411, 64) | 0 | — | — | — | relu | batch_normalization_6 |
| 7 conv2d_6 | (Conv2D) | (None, 20, 411, 64) | 12352 | (3, 1) | (1, 1) | same | — | activation_6 |
| add_3 | (Add) | (None, 20, 411, 64) | 0 | — | — | — | — | add_2<br>conv2d_6 |
| batch_normalization_7 | (BatchNormalization) | (None, 20, 411, 64) | 256 | — | — | — | — | add_3 |
| activation_7 | (Activation) | (None, 20, 411, 64) | 0 | — | — | — | relu | batch_normalization_7 |
| 8 conv2d_7 | (Conv2D) | (None, 10, 411, 128) | 24704 | (3, 1) | (2, 1) | same | — | activation_7 |
| batch_normalization_8 | (BatchNormalization) | (None, 10, 411, 128) | 512 | — | — | — | — | conv2d_7 |
| conv2d_9 | (Conv2D) | (None, 10, 411, 128) | 8320 | (1, 1) | | valid | — | add_3 |
| activation_8 | (Activation) | (None, 10, 411, 128) | 0 | — | — | — | relu | batch_normalization_8 |
| batch_normalization_9 | (BatchNormalization) | (None, 10, 411, 128) | 512 | — | — | — | — | conv2d_9 |
| 9 conv2d_8 | (Conv2D) | (None, 10, 411, 128) | 49280 | (3, 1) | (1, 1) | same | — | activation_8 |
| add_4 | (Add) | (None, 10, 411, 128) | 0 | — | — | — | — | batch_normalization_9<br>conv2d_8 |
| batch_normalization_10 | (BatchNormalization) | (None, 10, 411, 128) | 512 | — | — | — | — | add_4 |
| activation_9 | (Activation) | (None, 10, 411, 128) | 0 | — | — | — | relu | batch_normalization_10 |
| 10 conv2d_10 | (Conv2D) | (None, 10, 411, 128) | 49280 | (3, 1) | (1, 1) | same | — | activation_9 |
| batch_normalization_11 | (BatchNormalization) | (None, 10, 411, 128) | 512 | — | — | — | — | conv2d_10 |
| activation_10 | (Activation) | (None, 10, 411, 128) | 0 | — | — | — | relu | batch_normalization_11 |
| 11 conv2d_11 | (Conv2D) | (None, 10, 411, 128) | 49280 | (3, 1) | (1, 1) | same | — | activation_10 |
| add_5 | (Add) | (None, 10, 411, 128) | 0 | — | — | — | — | add_4<br>conv2d_11 |
| batch_normalization_12 | (BatchNormalization) | (None, 10, 411, 128) | 512 | — | — | — | — | add_5 |
| activation_11 | (Activation) | (None, 10, 411, 128) | 0 | — | — | — | relu | batch_normalization_12 |
| 12 conv2d_12 | (Conv2D) | (None, 10, 411, 128) | 49280 | (3, 1) | (1, 1) | same | — | activation_11 |
| batch_normalization_13 | (BatchNormalization) | (None, 10, 411, 128) | 512 | — | — | — | — | conv2d_12 |
| activation_12 | (Activation) | (None, 10, 411, 128) | 0 | — | — | — | relu | batch_normalization_13 |
| 13 conv2d_13 | (Conv2D) | (None, 10, 411, 128) | 49280 | (3, 1) | (1, 1) | same | — | activation_12 |
| add_6 | (Add) | (None, 10, 411, 128) | 0 | — | — | — | — | add_5<br>conv2d_13 |
| batch_normalization_14 | (BatchNormalization) | (None, 10, 411, 128) | 512 | — | — | — | — | add_6 |
| activation_13 | (Activation) | (None, 10, 411, 128) | 0 | — | — | — | relu | batch_normalization_14 |
| 14 conv2d_14 | (Conv2D) | (None, 10, 411, 128) | 49280 | (3, 1) | (1, 1) | same | — | activation_13 |
| batch_normalization_15 | (BatchNormalization) | (None, 10, 411, 128) | 512 | — | — | — | — | conv2d_14 |
| activation_14 | (Activation) | (None, 10, 411, 128) | 0 | — | — | — | relu | batch_normalization_15 |
| 15 conv2d_15 | (Conv2D) | (None, 10, 411, 128) | 49280 | (3, 1) | (1, 1) | same | — | activation_14 |
| add_7 | (Add) | (None, 10, 411, 128) | 0 | — | — | — | — | add_6<br>conv2d_15 |
| batch_normalization_16 | (BatchNormalization) | (None, 10, 411, 128) | 512 | — | — | — | — | add_7 |
| activation_15 | (Activation) | (None, 10, 411, 128) | 0 | — | — | — | relu | batch_normalization_16 |
| 16 conv2d_16 | (Conv2D) | (None, 5, 411, 256) | 98560 | (3, 1) | (2, 1) | same | — | activation_15 |
| batch_normalization_17 | (BatchNormalization) | (None, 5, 411, 256) | 1024 | — | — | — | — | conv2d_16 |
| conv2d_18 | (Conv2D) | (None, 5, 411, 256) | 33024 | (1, 1) | | valid | — | add_7 |
| activation_16 | (Activation) | (None, 5, 411, 256) | 0 | — | — | — | relu | batch_normalization_17 |
| batch_normalization_18 | (BatchNormalization) | (None, 5, 411, 256) | 1024 | — | — | — | — | conv2d_18 |
| 17 conv2d_17 | (Conv2D) | (None, 5, 411, 256) | 196864 | (3, 1) | (1, 1) | same | — | activation_16 |
| add_8 | (Add) | (None, 5, 411, 256) | 0 | — | — | — | — | batch_normalization_18<br>conv2d_17 |

| | | | | | | | | | |
|---|---|---|---|---|---|---|---|---|---|
| | batch_normalization_19 | (BatchNormalization) | (None, 5, 411, 256) | 1024 | — | — | — | — | add_8 |
| | activation_17 | (Activation) | (None, 5, 411, 256) | 0 | — | — | — | relu | batch_normalization_19 |
| 18 | conv2d_19 | (Conv2D) | (None, 5, 411, 256) | 196864 | (3, 1) | (1, 1) | same | — | activation_17 |
| | batch_normalization_20 | (BatchNormalization) | (None, 5, 411, 256) | 1024 | — | — | — | — | conv2d_19 |
| | activation_18 | (Activation) | (None, 5, 411, 256) | 0 | — | — | — | relu | batch_normalization_20 |
| 19 | conv2d_20 | (Conv2D) | (None, 5, 411, 256) | 196864 | (3, 1) | (1, 1) | same | — | activation_18 |
| | add_9 | (Add) | (None, 5, 411, 256) | 0 | — | — | — | — | add_8<br>conv2d_20 |
| | batch_normalization_21 | (BatchNormalization) | (None, 5, 411, 256) | 1024 | — | — | — | — | add_9 |
| | activation_19 | (Activation) | (None, 5, 411, 256) | 0 | — | — | — | relu | batch_normalization_21 |
| 20 | conv2d_21 | (Conv2D) | (None, 5, 411, 256) | 196864 | (3, 1) | (1, 1) | same | — | activation_19 |
| | batch_normalization_22 | (BatchNormalization) | (None, 5, 411, 256) | 1024 | — | — | — | — | conv2d_21 |
| | activation_20 | (Activation) | (None, 5, 411, 256) | 0 | — | — | — | relu | batch_normalization_22 |
| 21 | conv2d_22 | (Conv2D) | (None, 5, 411, 256) | 196864 | (3, 1) | (1, 1) | same | — | activation_20 |
| | add_10 | (Add) | (None, 5, 411, 256) | 0 | — | — | — | — | add_9<br>conv2d_22 |
| | batch_normalization_23 | (BatchNormalization) | (None, 5, 411, 256) | 1024 | — | — | — | — | add_10 |
| | activation_21 | (Activation) | (None, 5, 411, 256) | 0 | — | — | — | relu | batch_normalization_23 |
| 22 | conv2d_23 | (Conv2D) | (None, 5, 411, 256) | 196864 | (3, 1) | (1, 1) | same | — | activation_21 |
| | batch_normalization_24 | (BatchNormalization) | (None, 5, 411, 256) | 1024 | — | — | — | — | conv2d_23 |
| | activation_22 | (Activation) | (None, 5, 411, 256) | 0 | — | — | — | relu | batch_normalization_24 |
| 23 | conv2d_24 | (Conv2D) | (None, 5, 411, 256) | 196864 | (3, 1) | (1, 1) | same | — | activation_22 |
| | add_11 | (Add) | (None, 5, 411, 256) | 0 | — | — | — | — | add_10<br>conv2d_24 |
| | batch_normalization_25 | (BatchNormalization) | (None, 5, 411, 256) | 1024 | — | — | — | — | add_11 |
| | activation_23 | (Activation) | (None, 5, 411, 256) | 0 | — | — | — | relu | batch_normalization_25 |
| 24 | conv2d_25 | (Conv2D) | (None, 5, 411, 256) | 196864 | (3, 1) | (1, 1) | same | — | activation_23 |
| | batch_normalization_26 | (BatchNormalization) | (None, 5, 411, 256) | 1024 | — | — | — | — | conv2d_25 |
| | activation_24 | (Activation) | (None, 5, 411, 256) | 0 | — | — | — | relu | batch_normalization_26 |
| 25 | conv2d_26 | (Conv2D) | (None, 5, 411, 256) | 196864 | (3, 1) | (1, 1) | same | — | activation_24 |
| | add_12 | (Add) | (None, 5, 411, 256) | 0 | — | — | — | — | add_11<br>conv2d_26 |
| | batch_normalization_27 | (BatchNormalization) | (None, 5, 411, 256) | 1024 | — | — | — | — | add_12 |
| | activation_25 | (Activation) | (None, 5, 411, 256) | 0 | — | — | — | relu | batch_normalization_27 |
| 26 | conv2d_27 | (Conv2D) | (None, 5, 411, 256) | 196864 | (3, 1) | (1, 1) | same | — | activation_25 |
| | batch_normalization_28 | (BatchNormalization) | (None, 5, 411, 256) | 1024 | — | — | — | — | conv2d_27 |
| | activation_26 | (Activation) | (None, 5, 411, 256) | 0 | — | — | — | relu | batch_normalization_28 |
| 27 | conv2d_28 | (Conv2D) | (None, 5, 411, 256) | 196864 | (3, 1) | (1, 1) | same | — | activation_26 |
| | add_13 | (Add) | (None, 5, 411, 256) | 0 | — | — | — | — | add_12<br>conv2d_28 |
| | batch_normalization_29 | (BatchNormalization) | (None, 5, 411, 256) | 1024 | — | — | — | — | add_13 |
| | activation_27 | (Activation) | (None, 5, 411, 256) | 0 | — | — | — | relu | batch_normalization_29 |
| 28 | conv2d_29 | (Conv2D) | (None, 3, 411, 512) | 393728 | (3, 1) | (2, 1) | same | — | activation_27 |
| | batch_normalization_30 | (BatchNormalization) | (None, 3, 411, 512) | 2048 | — | — | — | — | conv2d_29 |
| | conv2d_31 | (Conv2D) | (None, 3, 411, 512) | 131584 | (1, 1) | | valid | — | add_13 |
| | activation_28 | (Activation) | (None, 3, 411, 512) | 0 | — | — | — | relu | batch_normalization_30 |
| | batch_normalization_31 | (BatchNormalization) | (None, 3, 411, 512) | 2048 | — | — | — | — | conv2d_31 |
| 29 | conv2d_30 | (Conv2D) | (None, 3, 411, 512) | 786944 | (3, 1) | (1, 1) | same | — | activation_28 |
| | add_14 | (Add) | (None, 3, 411, 512) | 0 | — | — | — | — | batch_normalization_31<br>conv2d_30 |
| | batch_normalization_32 | (BatchNormalization) | (None, 3, 411, 512) | 2048 | — | — | — | — | add_14 |
| | activation_29 | (Activation) | (None, 3, 411, 512) | 0 | — | — | — | relu | batch_normalization_32 |
| 30 | conv2d_32 | (Conv2D) | (None, 3, 411, 512) | 786944 | (3, 1) | (1, 1) | same | — | activation_29 |
| | batch_normalization_33 | (BatchNormalization) | (None, 3, 411, 512) | 2048 | — | — | — | — | conv2d_32 |
| | activation_30 | (Activation) | (None, 3, 411, 512) | 0 | — | — | — | relu | batch_normalization_33 |
| 31 | conv2d_33 | (Conv2D) | (None, 3, 411, 512) | 786944 | (3, 1) | (1, 1) | same | — | activation_30 |
| | add_15 | (Add) | (None, 3, 411, 512) | 0 | — | — | — | — | add_14<br>conv2d_33 |
| | batch_normalization_34 | (BatchNormalization) | (None, 3, 411, 512) | 2048 | — | — | — | — | add_15 |
| | activation_31 | (Activation) | (None, 3, 411, 512) | 0 | — | — | — | relu | batch_normalization_34 |
| 32 | conv2d_34 | (Conv2D) | (None, 3, 411, 512) | 786944 | (3, 1) | (1, 1) | same | — | activation_31 |
| | batch_normalization_35 | (BatchNormalization) | (None, 3, 411, 512) | 2048 | — | — | — | — | conv2d_34 |
| | activation_32 | (Activation) | (None, 3, 411, 512) | 0 | — | — | — | relu | batch_normalization_35 |
| 33 | conv2d_35 | (Conv2D) | (None, 3, 411, 512) | 786944 | (3, 1) | (1, 1) | same | — | activation_32 |
| | add_16 | (Add) | (None, 3, 411, 512) | 0 | — | — | — | — | add_15<br>conv2d_35 |
| | batch_normalization_36 | (BatchNormalization) | (None, 3, 411, 512) | 2048 | — | — | — | — | add_16 |
| | activation_33 | (Activation) | (None, 3, 411, 512) | 0 | — | — | — | relu | batch_normalization_36 |
| | average_pooling2d_1 | (AveragePooling2D) | (None, 1, 411, 512) | 0 | — | — | — | — | activation_33 |
| | flatten_1 | (Flatten) | (None, 210432) | 0 | — | — | — | — | average_pooling2d_1 |
| 34 | dense_1 | (Dense) | (None, 31) | 6523423 | — | — | — | softmax | flatten_1 |

| | |
|---|---|
| **Total parameters:** | **13,767,199** |
| **Trainable parameters:** | **13,750,175** |
| **Non-trainable parameters:** | **17024** |

Supplementary Table 2.11: ResNet-34-2D network architecture. Network was implemented using Keras with Tensorflow backend and trained for 10 epochs with 32 batch size. The network architectre was adopted from https://github.com/keras-team/keras-contrib/blob/master/keras_contrib/applications/resnet.py

| | Layer | (type) | Output Shape | # Param | Filter size | Stride | Padding | Activation | Connected to |
|---|---|---|---|---|---|---|---|---|---|
| | input_1 | (InputLayer) | (None, 80, 411, 1) | 0 | — | — | — | — | — |
| 1 | conv2d_1 | (Conv2D) | (None, 40, 206, 64) | 3200 | (7, 7) | (2, 2) | same | — | input_1 |
| | batch_normalization_1 | (BatchNormalization) | (None, 40, 206, 64) | 256 | — | — | — | — | conv2d_1 |
| | activation_1 | (Activation) | (None, 40, 206, 64) | 0 | — | — | — | relu | batch_normalization_1 |
| | max_pooling2d_1 | (MaxPooling2D) | (None, 20, 103, 64) | 0 | (3, 3) | (2, 2) | same | — | activation_1 |
| 2 | res0a_branch2a | (Conv2D) | (None, 20, 103, 64) | 36928 | (3, 3) | (1, 1) | same | — | max_pooling2d_1 |
| | batch_normalization_2 | (BatchNormalization) | (None, 20, 103, 64) | 256 | — | — | — | — | res0a_branch2a |
| | activation_2 | (Activation) | (None, 20, 103, 64) | 0 | — | — | — | relu | batch_normalization_2 |
| 3 | conv2d_2 | (Conv2D) | (None, 20, 103, 64) | 36928 | (3, 3) | (1, 1) | same | — | activation_2 |
| | add_1 | (Add) | (None, 20, 103, 64) | 0 | — | — | — | — | max_pooling2d_1<br>conv2d_2 |
| | batch_normalization_3 | (BatchNormalization) | (None, 20, 103, 64) | 256 | — | — | — | — | add_1 |
| | activation_3 | (Activation) | (None, 20, 103, 64) | 0 | — | — | — | relu | batch_normalization_3 |
| 4 | conv2d_3 | (Conv2D) | (None, 20, 103, 64) | 36928 | (3, 3) | (1, 1) | same | — | activation_3 |
| | batch_normalization_4 | (BatchNormalization) | (None, 20, 103, 64) | 256 | — | — | — | — | conv2d_3 |
| | activation_4 | (Activation) | (None, 20, 103, 64) | 0 | — | — | — | relu | batch_normalization_4 |
| 5 | conv2d_4 | (Conv2D) | (None, 20, 103, 64) | 36928 | (3, 3) | (1, 1) | same | — | activation_4 |
| | add_2 | (Add) | (None, 20, 103, 64) | 0 | — | — | — | — | add_1<br>conv2d_4 |
| | batch_normalization_5 | (BatchNormalization) | (None, 20, 103, 64) | 256 | — | — | — | — | add_2 |
| | activation_5 | (Activation) | (None, 20, 103, 64) | 0 | — | — | — | relu | batch_normalization_5 |
| 6 | conv2d_5 | (Conv2D) | (None, 20, 103, 64) | 36928 | (3, 3) | (1, 1) | same | — | activation_5 |
| | batch_normalization_6 | (BatchNormalization) | (None, 20, 103, 64) | 256 | — | — | — | — | conv2d_5 |
| | activation_6 | (Activation) | (None, 20, 103, 64) | 0 | — | — | — | relu | batch_normalization_6 |
| 7 | conv2d_6 | (Conv2D) | (None, 20, 103, 64) | 36928 | (3, 3) | (1, 1) | same | — | activation_6 |
| | add_3 | (Add) | (None, 20, 103, 64) | 0 | — | — | — | — | add_2<br>conv2d_6 |
| | batch_normalization_7 | (BatchNormalization) | (None, 20, 103, 64) | 256 | — | — | — | — | add_3 |
| | activation_7 | (Activation) | (None, 20, 103, 64) | 0 | — | — | — | relu | batch_normalization_7 |
| 8 | conv2d_7 | (Conv2D) | (None, 10, 52, 128) | 73856 | (3, 3) | (1, 1) | same | — | activation_7 |
| | batch_normalization_8 | (BatchNormalization) | (None, 10, 52, 128) | 512 | — | — | — | — | conv2d_7 |
| | conv2d_9 | (Conv2D) | (None, 10, 52, 128) | 8320 | (1, 1) | | valid | — | add_3 |
| | activation_8 | (Activation) | (None, 10, 52, 128) | 0 | — | — | — | relu | batch_normalization_8 |
| | batch_normalization_9 | (BatchNormalization) | (None, 10, 52, 128) | 512 | — | — | — | — | conv2d_9 |
| 9 | conv2d_8 | (Conv2D) | (None, 10, 52, 128) | 147584 | (3, 3) | (1, 1) | same | — | activation_8 |
| | add_4 | (Add) | (None, 10, 52, 128) | 0 | — | — | — | — | batch_normalization_9<br>conv2d_8 |
| | batch_normalization_10 | (BatchNormalization) | (None, 10, 52, 128) | 512 | — | — | — | — | add_4 |
| | activation_9 | (Activation) | (None, 10, 52, 128) | 0 | — | — | — | relu | batch_normalization_10 |
| 10 | conv2d_10 | (Conv2D) | (None, 10, 52, 128) | 147584 | (3, 3) | (1, 1) | same | — | activation_9 |
| | batch_normalization_11 | (BatchNormalization) | (None, 10, 52, 128) | 512 | — | — | — | — | conv2d_10 |
| | activation_10 | (Activation) | (None, 10, 52, 128) | 0 | — | — | — | relu | batch_normalization_11 |
| 11 | conv2d_11 | (Conv2D) | (None, 10, 52, 128) | 147584 | (3, 3) | (1, 1) | same | — | activation_10 |
| | add_5 | (Add) | (None, 10, 52, 128) | 0 | — | — | — | — | add_4<br>conv2d_11 |
| | batch_normalization_12 | (BatchNormalization) | (None, 10, 52, 128) | 512 | — | — | — | — | add_5 |
| | activation_11 | (Activation) | (None, 10, 52, 128) | 0 | — | — | — | relu | batch_normalization_12 |
| 12 | conv2d_12 | (Conv2D) | (None, 10, 52, 128) | 147584 | (3, 3) | (1, 1) | same | — | activation_11 |
| | batch_normalization_13 | (BatchNormalization) | (None, 10, 52, 128) | 512 | — | — | — | — | conv2d_12 |
| | activation_12 | (Activation) | (None, 10, 52, 128) | 0 | — | — | — | relu | batch_normalization_13 |
| 13 | conv2d_13 | (Conv2D) | (None, 10, 52, 128) | 147584 | (3, 3) | (1, 1) | same | — | activation_12 |
| | add_6 | (Add) | (None, 10, 52, 128) | 0 | — | — | — | — | add_5<br>conv2d_13 |
| | batch_normalization_14 | (BatchNormalization) | (None, 10, 52, 128) | 512 | — | — | — | — | add_6 |
| | activation_13 | (Activation) | (None, 10, 52, 128) | 0 | — | — | — | relu | batch_normalization_14 |
| 14 | conv2d_14 | (Conv2D) | (None, 10, 52, 128) | 147584 | (3, 3) | (1, 1) | same | — | activation_13 |
| | batch_normalization_15 | (BatchNormalization) | (None, 10, 52, 128) | 512 | — | — | — | — | conv2d_14 |
| | activation_14 | (Activation) | (None, 10, 52, 128) | 0 | — | — | — | relu | batch_normalization_15 |
| 15 | conv2d_15 | (Conv2D) | (None, 10, 52, 128) | 147584 | (3, 3) | (1, 1) | same | — | activation_14 |
| | add_7 | (Add) | (None, 10, 52, 128) | 0 | — | — | — | — | add_6<br>conv2d_15 |
| | batch_normalization_16 | (BatchNormalization) | (None, 10, 52, 128) | 512 | — | — | — | — | add_7 |
| | activation_15 | (Activation) | (None, 10, 52, 128) | 0 | — | — | — | relu | batch_normalization_16 |
| 16 | conv2d_16 | (Conv2D) | (None, 5, 26, 256) | 295168 | (3, 3) | (1, 1) | same | — | activation_15 |
| | batch_normalization_17 | (BatchNormalization) | (None, 5, 26, 256) | 1024 | — | — | — | — | conv2d_16 |
| | conv2d_18 | (Conv2D) | (None, 5, 26, 256) | 33024 | (1, 1) | | valid | — | add_7 |
| | activation_16 | (Activation) | (None, 5, 26, 256) | 0 | — | — | — | relu | batch_normalization_17 |
| | batch_normalization_18 | (BatchNormalization) | (None, 5, 26, 256) | 1024 | — | — | — | — | conv2d_18 |
| 17 | conv2d_17 | (Conv2D) | (None, 5, 26, 256) | 590080 | (3, 3) | (1, 1) | same | — | activation_16 |
| | add_8 | (Add) | (None, 5, 26, 256) | 0 | — | — | — | — | batch_normalization_18<br>conv2d_17 |

| | | | | | | | | | |
|---|---|---|---|---|---|---|---|---|---|
| | batch_normalization_19 | (BatchNormalization) | (None, 5, 26, 256) | 1024 | — | — | — | — | add_8 |
| | activation_17 | (Activation) | (None, 5, 26, 256) | 0 | — | — | — | relu | batch_normalization_19 |
| 18 | conv2d_19 | (Conv2D) | (None, 5, 26, 256) | 590080 | (3, 3) | (1, 1) | same | — | activation_17 |
| | batch_normalization_20 | (BatchNormalization) | (None, 5, 26, 256) | 1024 | — | — | — | — | conv2d_19 |
| | activation_18 | (Activation) | (None, 5, 26, 256) | 0 | — | — | — | relu | batch_normalization_20 |
| 19 | conv2d_20 | (Conv2D) | (None, 5, 26, 256) | 590080 | (3, 3) | (1, 1) | same | — | activation_18 |
| | add_9 | (Add) | (None, 5, 26, 256) | 0 | — | — | — | — | add_8<br>conv2d_20 |
| | batch_normalization_21 | (BatchNormalization) | (None, 5, 26, 256) | 1024 | — | — | — | — | add_9 |
| | activation_19 | (Activation) | (None, 5, 26, 256) | 0 | — | — | — | relu | batch_normalization_21 |
| 20 | conv2d_21 | (Conv2D) | (None, 5, 26, 256) | 590080 | (3, 3) | (1, 1) | same | — | activation_19 |
| | batch_normalization_22 | (BatchNormalization) | (None, 5, 26, 256) | 1024 | — | — | — | — | conv2d_21 |
| | activation_20 | (Activation) | (None, 5, 26, 256) | 0 | — | — | — | relu | batch_normalization_22 |
| 21 | conv2d_22 | (Conv2D) | (None, 5, 26, 256) | 590080 | (3, 3) | (1, 1) | same | — | activation_20 |
| | add_10 | (Add) | (None, 5, 26, 256) | 0 | — | — | — | — | add_9<br>conv2d_22 |
| | batch_normalization_23 | (BatchNormalization) | (None, 5, 26, 256) | 1024 | — | — | — | — | add_10 |
| | activation_21 | (Activation) | (None, 5, 26, 256) | 0 | — | — | — | relu | batch_normalization_23 |
| 22 | conv2d_23 | (Conv2D) | (None, 5, 26, 256) | 590080 | (3, 3) | (1, 1) | same | — | activation_21 |
| | batch_normalization_24 | (BatchNormalization) | (None, 5, 26, 256) | 1024 | — | — | — | — | conv2d_23 |
| | activation_22 | (Activation) | (None, 5, 26, 256) | 0 | — | — | — | relu | batch_normalization_24 |
| 23 | conv2d_24 | (Conv2D) | (None, 5, 26, 256) | 590080 | (3, 3) | (1, 1) | same | — | activation_22 |
| | add_11 | (Add) | (None, 5, 26, 256) | 0 | — | — | — | — | add_10<br>conv2d_24 |
| | batch_normalization_25 | (BatchNormalization) | (None, 5, 26, 256) | 1024 | — | — | — | — | add_11 |
| | activation_23 | (Activation) | (None, 5, 26, 256) | 0 | — | — | — | relu | batch_normalization_25 |
| 24 | conv2d_25 | (Conv2D) | (None, 5, 26, 256) | 590080 | (3, 3) | (1, 1) | same | — | activation_23 |
| | batch_normalization_26 | (BatchNormalization) | (None, 5, 26, 256) | 1024 | — | — | — | — | conv2d_25 |
| | activation_24 | (Activation) | (None, 5, 26, 256) | 0 | — | — | — | relu | batch_normalization_26 |
| 25 | conv2d_26 | (Conv2D) | (None, 5, 26, 256) | 590080 | (3, 3) | (1, 1) | same | — | activation_24 |
| | add_12 | (Add) | (None, 5, 26, 256) | 0 | — | — | — | — | add_11<br>conv2d_26 |
| | batch_normalization_27 | (BatchNormalization) | (None, 5, 26, 256) | 1024 | — | — | — | — | add_12 |
| | activation_25 | (Activation) | (None, 5, 26, 256) | 0 | — | — | — | relu | batch_normalization_27 |
| 26 | conv2d_27 | (Conv2D) | (None, 5, 26, 256) | 590080 | (3, 3) | (1, 1) | same | — | activation_25 |
| | batch_normalization_28 | (BatchNormalization) | (None, 5, 26, 256) | 1024 | — | — | — | — | conv2d_27 |
| | activation_26 | (Activation) | (None, 5, 26, 256) | 0 | — | — | — | relu | batch_normalization_28 |
| 27 | conv2d_28 | (Conv2D) | (None, 5, 26, 256) | 590080 | (3, 3) | (1, 1) | same | — | activation_26 |
| | add_13 | (Add) | (None, 5, 26, 256) | 0 | — | — | — | — | add_12<br>conv2d_28 |
| | batch_normalization_29 | (BatchNormalization) | (None, 5, 26, 256) | 1024 | — | — | — | — | add_13 |
| | activation_27 | (Activation) | (None, 5, 26, 256) | 0 | — | — | — | relu | batch_normalization_29 |
| 28 | conv2d_29 | (Conv2D) | (None, 3, 13, 512) | 1180160 | (3, 3) | (1, 1) | same | — | activation_27 |
| | batch_normalization_30 | (BatchNormalization) | (None, 3, 13, 512) | 2048 | — | — | — | — | conv2d_29 |
| | conv2d_31 | (Conv2D) | (None, 3, 13, 512) | 131584 | (1, 1) | | valid | — | add_13 |
| | activation_28 | (Activation) | (None, 3, 13, 512) | 0 | — | — | — | relu | batch_normalization_30 |
| | batch_normalization_31 | (BatchNormalization) | (None, 3, 13, 512) | 2048 | — | — | — | — | conv2d_31 |
| 29 | conv2d_30 | (Conv2D) | (None, 3, 13, 512) | 2359808 | (3, 3) | (1, 1) | same | — | activation_28 |
| | add_14 | (Add) | (None, 3, 13, 512) | 0 | — | — | — | — | batch_normalization_31<br>conv2d_30 |
| | batch_normalization_32 | (BatchNormalization) | (None, 3, 13, 512) | 2048 | — | — | — | — | add_14 |
| | activation_29 | (Activation) | (None, 3, 13, 512) | 0 | — | — | — | relu | batch_normalization_32 |
| 30 | conv2d_32 | (Conv2D) | (None, 3, 13, 512) | 2359808 | (3, 3) | (1, 1) | same | — | activation_29 |
| | batch_normalization_33 | (BatchNormalization) | (None, 3, 13, 512) | 2048 | — | — | — | — | conv2d_32 |
| | activation_30 | (Activation) | (None, 3, 13, 512) | 0 | — | — | — | relu | batch_normalization_33 |
| 31 | conv2d_33 | (Conv2D) | (None, 3, 13, 512) | 2359808 | (3, 3) | (1, 1) | same | — | activation_30 |
| | add_15 | (Add) | (None, 3, 13, 512) | 0 | — | — | — | — | add_14<br>conv2d_33 |
| | batch_normalization_34 | (BatchNormalization) | (None, 3, 13, 512) | 2048 | — | — | — | — | add_15 |
| | activation_31 | (Activation) | (None, 3, 13, 512) | 0 | — | — | — | relu | batch_normalization_34 |
| 32 | conv2d_34 | (Conv2D) | (None, 3, 13, 512) | 2359808 | (3, 3) | (1, 1) | same | — | activation_31 |
| | batch_normalization_35 | (BatchNormalization) | (None, 3, 13, 512) | 2048 | — | — | — | — | conv2d_34 |
| | activation_32 | (Activation) | (None, 3, 13, 512) | 0 | — | — | — | relu | batch_normalization_35 |
| 33 | conv2d_35 | (Conv2D) | (None, 3, 13, 512) | 2359808 | (3, 3) | (1, 1) | same | — | activation_32 |
| | add_16 | (Add) | (None, 3, 13, 512) | 0 | | — | — | — | add_15<br>conv2d_35 |
| | batch_normalization_36 | (BatchNormalization) | (None, 3, 13, 512) | 2048 | | — | — | — | add_16 |
| | activation_33 | (Activation) | (None, 3, 13, 512) | 0 | | — | — | relu | batch_normalization_36 |
| | global_average_pooling2d_1 | (GlogalAveragePooling2D) | (None, 512) | 0 | | — | — | — | activation_33 |
| 34 | dense_1 | (Dense) | (None, 31) | 15903 | | — | — | softmax | global_average_pooling2d_1 |

| | |
|---|---|
| **Total parameters:** | **21,319,839** |
| **Trainable parameters:** | **21,302,815** |
| **Non-trainable parameters:** | **17024** |

# 3 VGG-8-1D model – Results

Supplementary Table 3.1: Results of the testing clinical sample analysis with the CNN-based system with VGG-8-1D model. Results evaluated per each target VOC.

*Label* - the class label of VOC. *TP* - number of true positives detected per VOC. *TTP* - number of tentative true positives detected per VOC. *FP* - number of false positives detected per VOC. *TTN* - number of tentative true negatives detected per VOC. *FN* - number of false negatives detected per VOC. *TN* - number of true negatives detected per VOC (evaluation excluding *RT* position). *FP** - number of false positives detected per VOC (evaluation excluding *RT* position). *TTP** - number of tentative true positives detected per VOC (evaluation excluding *RT* position). *Sensitivity (expert)* - Sensitivity per VOC in relation to expert-derived ground truth benchmark; tentative true positives (TTP) are considered FP, tentative true negatives (TTN) are considered FN; sensitivity = TP/(TP+FN+TTN). *Sensitivity (system)* - Sensitivity per VOC in relation to system-derived correction benchmark; tentative true positives (TTP) are considered TP, tentative true negatives (TTN) are considered TN; sensitivity=(TP+TTP)/(TP+TTP+FN). *Specificity (expert)* - Specificity per VOC in relation to expert-derived ground truth benchmark; tentative true positives (TTP*) are considered FP*; specificity=TN/TN+FP*+TTP*. *Specificity (system)* - Specificity per VOC in relation to system-derived correction benchmark; tentative true positives (TTP*) are considered TP; specificity=TN/TN+FP*. *AP (expert)* - Average precision per VOC in relation to expert-derived ground truth benchmark. *AP (system)* - Average precision per VOC in relation to system-derived correction benchmark.

| Label | TP | TTP | FP | TTN | FN | TN | FP* | TTP* | Sensitivity (expert) | Sensitivity (system) | Specificity (expert) | Specificity (system) | AP (expert) | AP (system) |
|---|---|---|---|---|---|---|---|---|---|---|---|---|---|---|
| 1 | 20 | 18 | 0 | 0 | 0 | 0 | 0 | 18 | 1 | 1 | 0 | - | 0.8282 | 1 |
| 2 | 29 | 7 | 0 | 0 | 0 | 2 | 0 | 7 | 1 | 1 | 0.2222 | 1 | 0.9706 | 1 |
| 3 | 30 | 8 | 0 | 0 | 0 | 0 | 0 | 8 | 1 | 1 | 0 | - | 0.9989 | 1 |
| 4 | 38 | 0 | 0 | 0 | 0 | 0 | 0 | 0 | 1 | 1 | - | - | 1 | 1 |
| 5 | 35 | 3 | 0 | 1 | 0 | 0 | 0 | 2 | 0.9722 | 1 | 0 | - | 0.9393 | 1 |
| 6 | 10 | 27 | 0 | 1 | 0 | 1 | 0 | 26 | 0.9091 | 1 | 0.037 | 1 | 0.6951 | 1 |
| 7 | 23 | 7 | 0 | 0 | 0 | 8 | 0 | 7 | 1 | 1 | 0.5333 | 1 | 0.9917 | 1 |
| 8 | 37 | 1 | 0 | 0 | 0 | 0 | 0 | 1 | 1 | 1 | 0 | - | 0.9915 | 1 |
| 9 | 38 | 0 | 0 | 0 | 0 | 0 | 0 | 0 | 1 | 1 | - | - | 1 | 1 |
| 10 | 29 | 5 | 0 | 1 | 0 | 4 | 0 | 4 | 0.9667 | 1 | 0.5 | 1 | 0.9622 | 1 |
| 11 | 13 | 20 | 0 | 6 | 0 | 5 | 0 | 14 | 0.6842 | 1 | 0.2632 | 1 | 0.4153 | 1 |
| 12 | 24 | 10 | 0 | 1 | 0 | 4 | 0 | 9 | 0.96 | 1 | 0.3077 | 1 | 0.8974 | 1 |
| 13 | 32 | 4 | 0 | 1 | 0 | 2 | 0 | 3 | 0.9697 | 1 | 0.4 | 1 | 0.926 | 1 |
| 14 | 32 | 2 | 0 | 0 | 1 | 3 | 0 | 2 | 0.9697 | 0.9714 | 0.6 | 1 | 0.9642 | 0.9714 |
| 15 | 22 | 15 | 0 | 1 | 0 | 1 | 0 | 14 | 0.9565 | 1 | 0.0667 | 1 | 0.8076 | 1 |
| 16 | 19 | 11 | 2 | 1 | 3 | 4 | 1 | 10 | 0.8261 | 0.9091 | 0.2667 | 0.8 | 0.8086 | 0.8965 |
| 17 | 38 | 0 | 0 | 0 | 0 | 0 | 0 | 0 | 1 | 1 | - | - | 1 | 1 |
| 18 | 32 | 2 | 0 | 0 | 4 | 0 | 0 | 2 | 0.8889 | 0.8947 | 0 | - | 0.8676 | 0.8947 |
| 19 | 26 | 11 | 0 | 0 | 0 | 1 | 0 | 11 | 1 | 1 | 0.0833 | 1 | 0.8144 | 1 |
| 20 | 36 | 0 | 0 | 0 | 1 | 1 | 0 | 0 | 0.973 | 0.973 | 1 | 1 | 0.973 | 0.973 |
| 21 | 21 | 15 | 0 | 4 | 2 | 0 | 0 | 11 | 0.7778 | 0.9474 | 0 | - | 0.745 | 0.9474 |
| 22 | 32 | 6 | 0 | 0 | 0 | 0 | 0 | 6 | 1 | 1 | 0 | - | 0.9879 | 1 |
| 23 | 36 | 0 | 0 | 0 | 0 | 2 | 0 | 0 | 1 | 1 | 1 | 1 | 1 | 1 |
| 24 | 24 | 13 | 0 | 0 | 0 | 1 | 0 | 13 | 1 | 1 | 0.0714 | 1 | 0.9208 | 1 |
| 25 | 7 | 5 | 0 | 0 | 0 | 26 | 0 | 5 | 1 | 1 | 0.8387 | 1 | 0.8052 | 1 |
| 26 | 21 | 16 | 0 | 1 | 0 | 1 | 0 | 15 | 0.9545 | 1 | 0.0625 | 1 | 0.9313 | 1 |
| 27 | 32 | 4 | 0 | 0 | 0 | 2 | 0 | 4 | 1 | 1 | 0.3333 | 1 | 0.9789 | 1 |
| 28 | 17 | 6 | 0 | 0 | 0 | 15 | 0 | 6 | 1 | 1 | 0.7143 | 1 | 0.8823 | 1 |
| 29 | 31 | 7 | 0 | 0 | 0 | 0 | 0 | 7 | 1 | 1 | 0 | - | 0.957 | 1 |
| 30 | 32 | 3 | 0 | 0 | 0 | 3 | 0 | 3 | 1 | 1 | 0.5 | 1 | 0.9962 | 1 |
| **TOTAL** | **816** | **226** | **2** | **18** | **11** | **86** | **1** | **208** | **0.9657** | **0.9896** | **0.2915** | **0.9885** | **mAP** | |
| | | | | | | | | | | | | | **0.9019** | **0.9894** |

Supplementary Figures 3.1-3.8: Precision against recall graphs for VOCs 1-8.

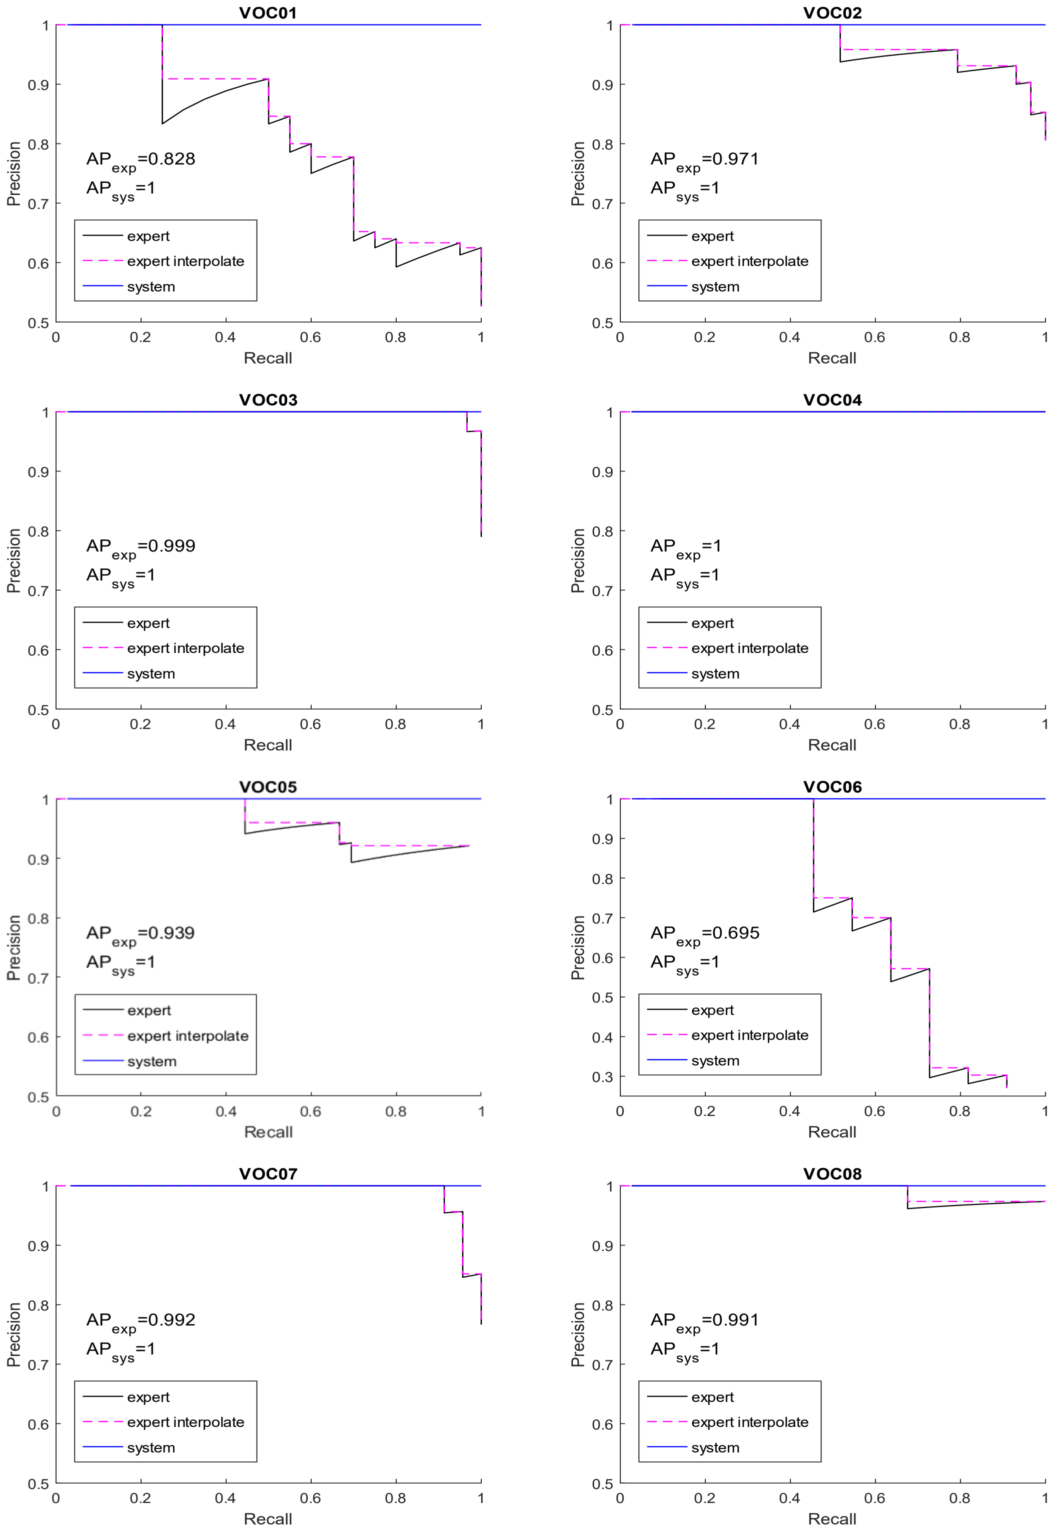

Supplementary Figures 3.9-3.16: Precision against recall graphs for VOCs 9-16.

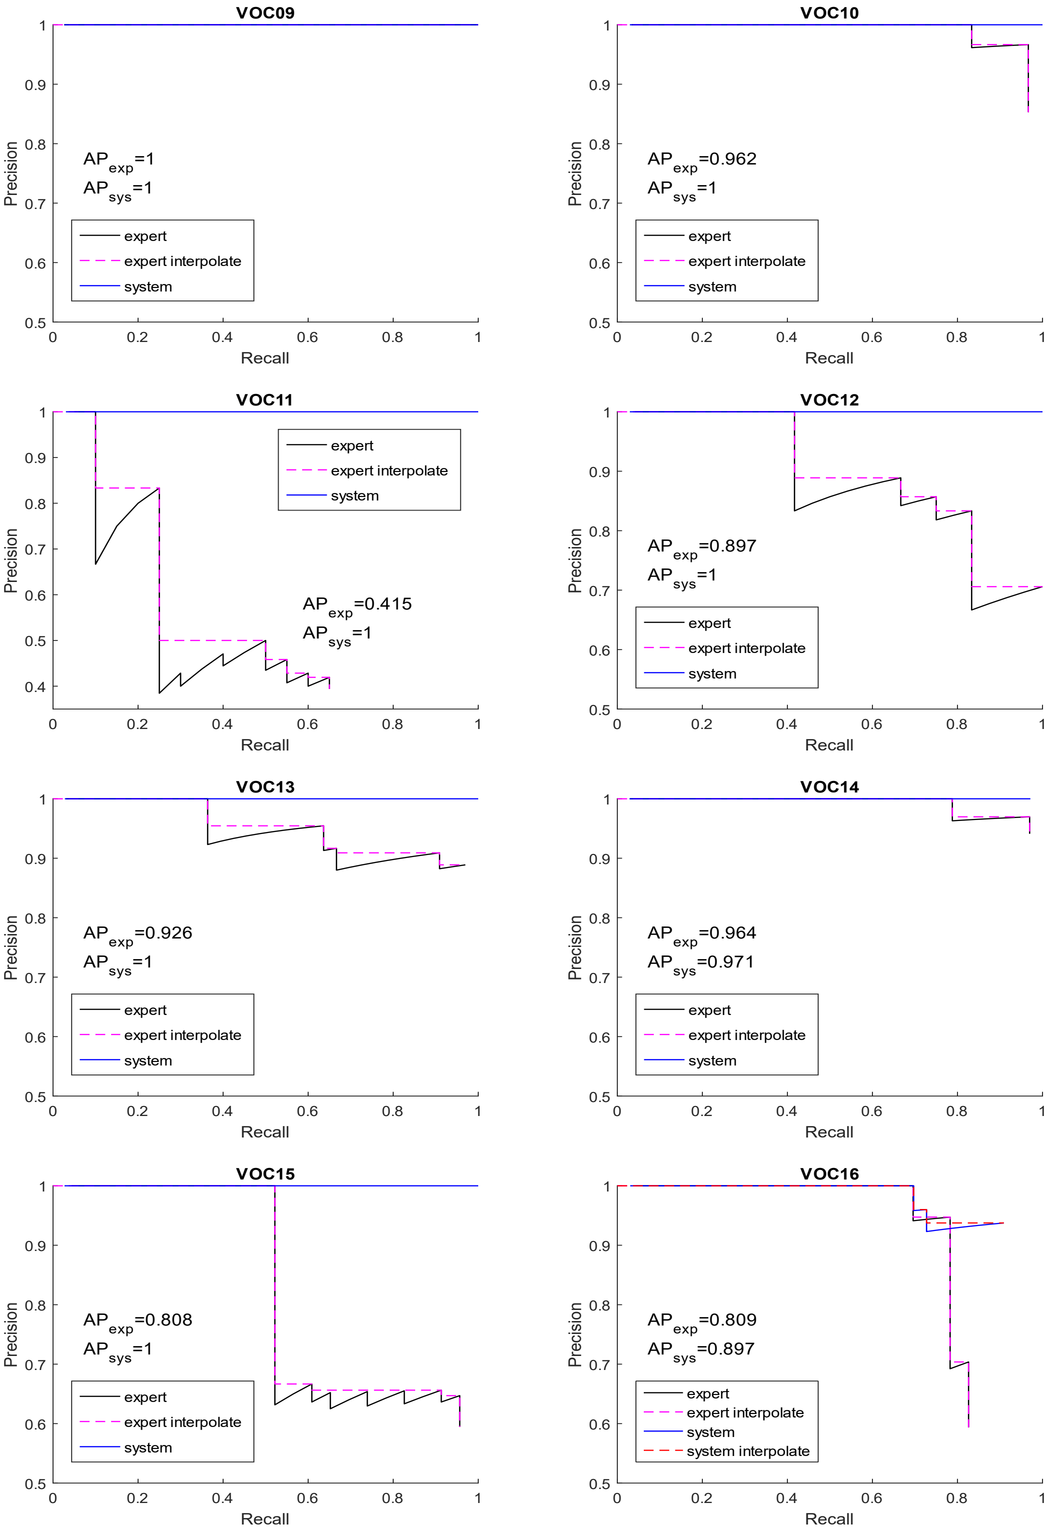

Supplementary Figures 3.17-3.24: Precision against recall graphs for VOCs 17-24.

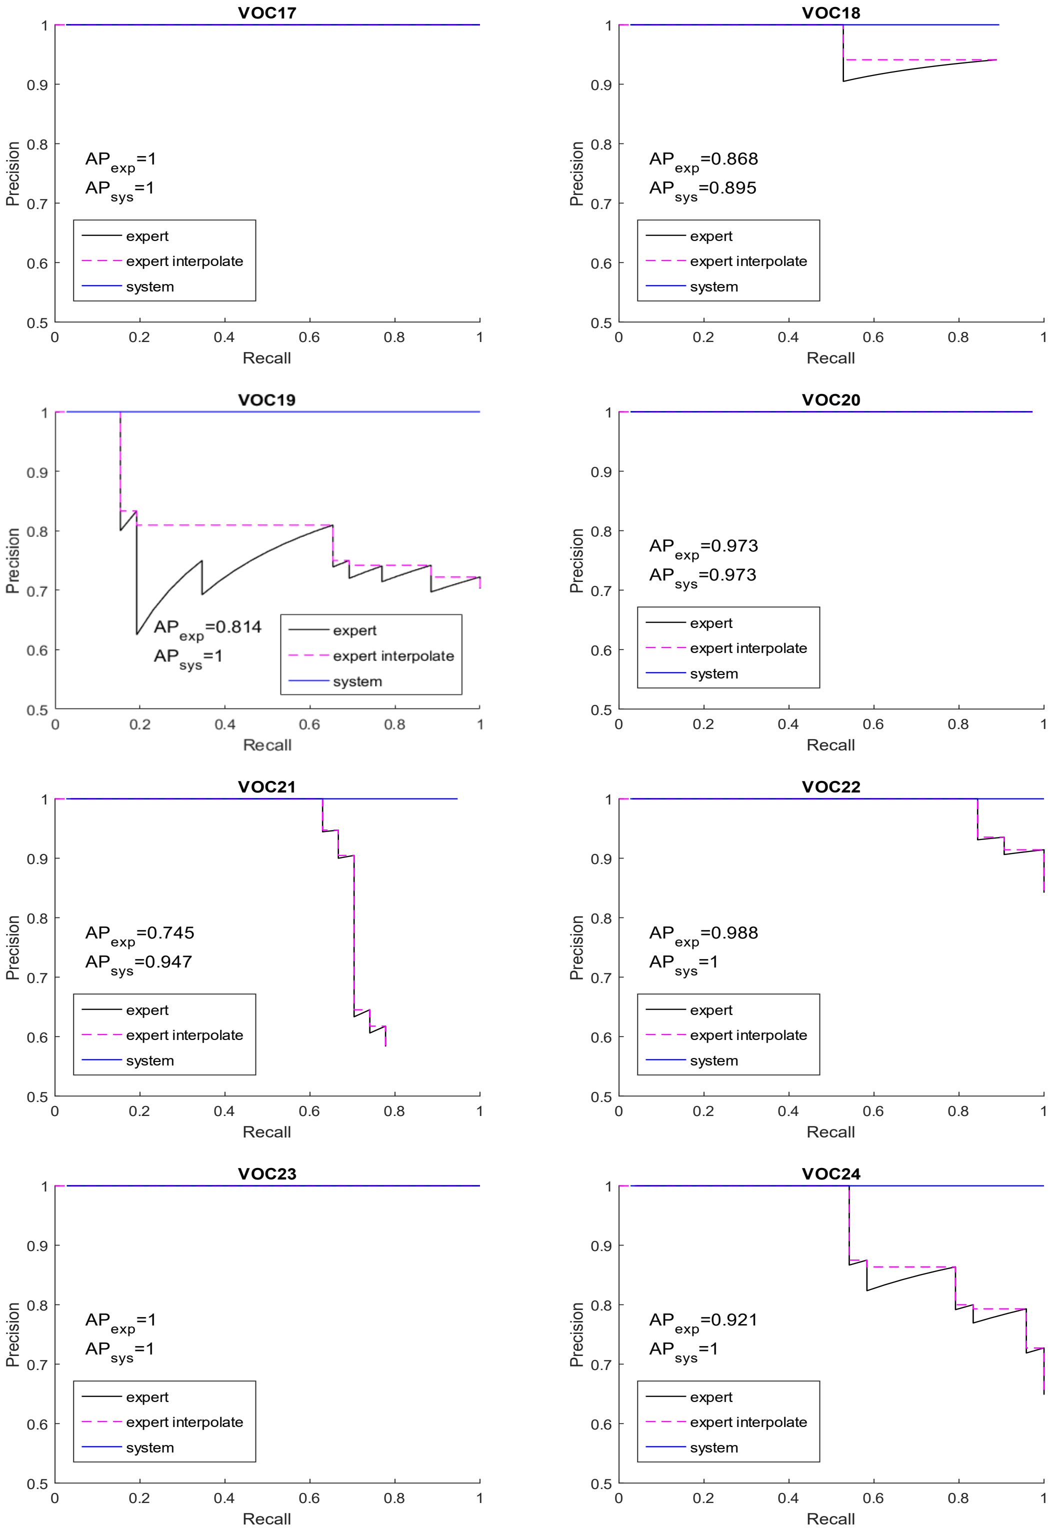

Supplementary Figures 3.25-3.30: Precision against recall graphs for VOCs 25-30.

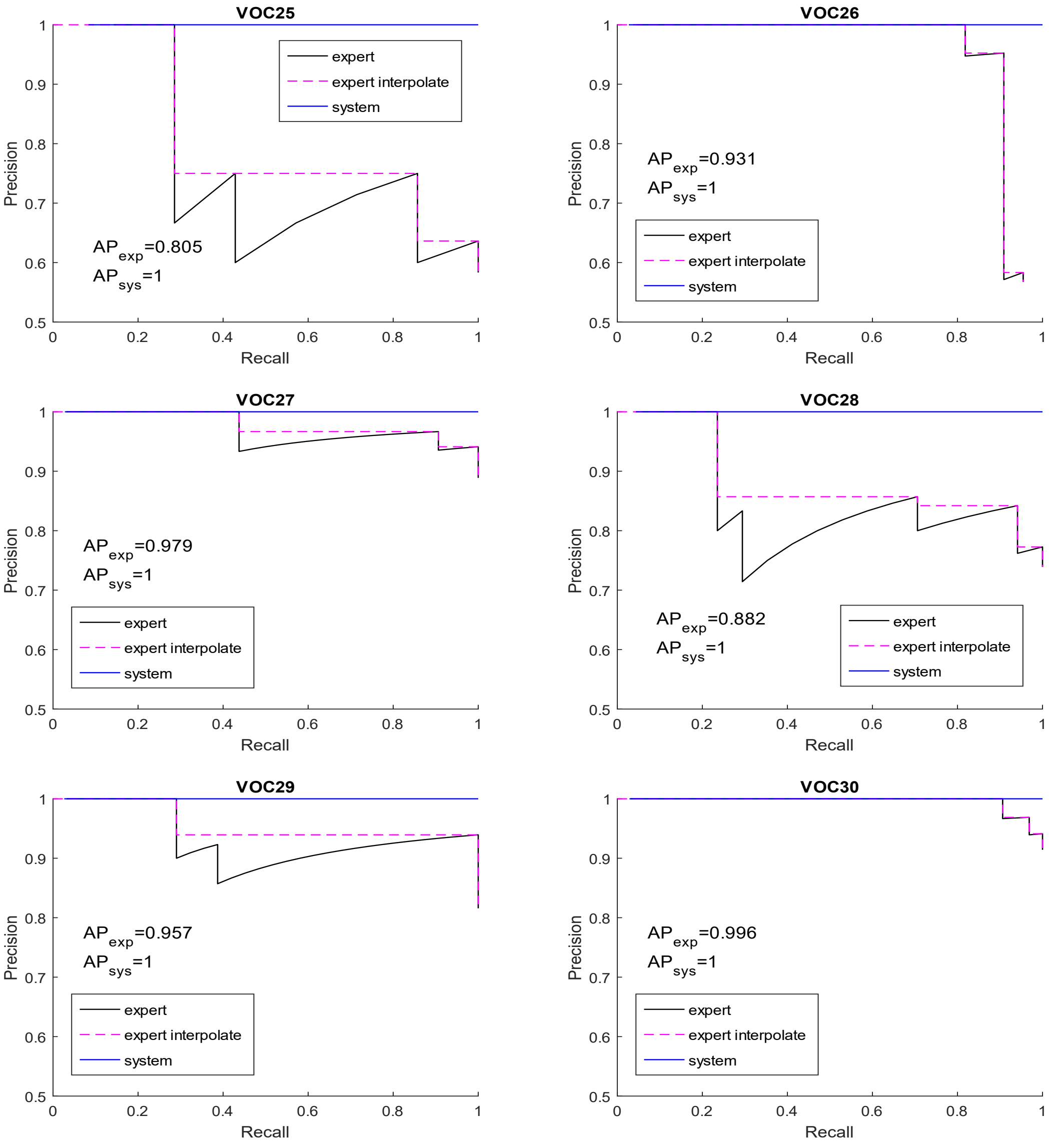

Supplementary Table 3.2: Results of the testing clinical sample analysis with the CNN-based system with VGG-8-1D model. Results evaluated per each testing sample.

Sample ID - number of a sample. TP - number of true positives detected per sample. TTP - number of tentative true positives detected per sample. FP - number of false positives detected per sample. TTN - number of tentative true negatives detected per sample. FN - number of false negatives detected per sample. TN - number of true negatives detected per sample (evaluation excluding *RT* position). FP* - number of false positives detected per sample (evaluation excluding *RT* position). TTP* - number of tentative true positives detected per sample (evaluation excluding *RT* position). *Sensitivity (expert)* - Sensitivity per sample in relation to expert-derived ground truth benchmark; tentative true positives (TTP) are considered FP, tentative true negatives (TTN) are considered FN; sensitivity = TP/(TP+FN+TTN). *Sensitivity (system)* - Sensitivity per sample in relation to system-derived correction benchmark; tentative true positives (TTP) are considered TP, tentative true negatives (TTN) are considered TN; sensitivity=(TP+TTP)/(TP+TTP+FN). *Specificity (expert)* - Specificity per sample in relation to expert-derived ground truth benchmark; tentative true positives (TTP*) are considered FP*; specificity=TN/TN+FP*+TTP*. *Specificity (system)* - Specificity per sample in relation to system-derived correction benchmark; tentative true positives (TTP*) are considered TP; specificity=TN/TN+FP*.

| Sample ID | TP | TTP | FP | TTN | FN | TN | FP* | TTP* | Sensitivity (expert) | Sensitivity (system) | Specificity (expert) | Specificity (system) |
|---|---|---|---|---|---|---|---|---|---|---|---|---|
| 1 | 26 | 2 | 0 | 0 | 1 | 1 | 0 | 2 | 0.963 | 0.9655 | 0.3333 | 1 |
| 2 | 24 | 4 | 0 | 0 | 1 | 1 | 0 | 4 | 0.96 | 0.9655 | 0.2 | 1 |
| 3 | 26 | 3 | 0 | 2 | 0 | 1 | 0 | 1 | 0.9286 | 1 | 0.5 | 1 |
| 4 | 27 | 2 | 0 | 0 | 0 | 1 | 0 | 2 | 1 | 1 | 0.3333 | 1 |
| 5 | 16 | 6 | 0 | 0 | 0 | 8 | 0 | 6 | 1 | 1 | 0.5714 | 1 |
| 6 | 24 | 4 | 0 | 1 | 0 | 2 | 0 | 3 | 0.96 | 1 | 0.4 | 1 |
| 7 | 26 | 2 | 0 | 0 | 1 | 1 | 0 | 2 | 0.963 | 0.9655 | 0.3333 | 1 |
| 8 | 24 | 3 | 0 | 0 | 1 | 2 | 0 | 3 | 0.96 | 0.9643 | 0.4 | 1 |
| 9 | 26 | 2 | 0 | 0 | 0 | 2 | 0 | 2 | 1 | 1 | 0.5 | 1 |
| 10 | 10 | 9 | 0 | 0 | 1 | 10 | 0 | 9 | 0.9091 | 0.95 | 0.5263 | 1 |
| 11 | 24 | 5 | 0 | 0 | 0 | 1 | 0 | 5 | 1 | 1 | 0.1667 | 1 |
| 12 | 24 | 5 | 0 | 1 | 0 | 1 | 0 | 4 | 0.96 | 1 | 0.2 | 1 |
| 13 | 22 | 6 | 1 | 0 | 0 | 1 | 1 | 6 | 1 | 1 | 0.125 | 0.5 |
| 14 | 25 | 4 | 0 | 0 | 0 | 1 | 0 | 4 | 1 | 1 | 0.2 | 1 |
| 15 | 24 | 3 | 1 | 0 | 1 | 2 | 0 | 3 | 0.96 | 0.9643 | 0.4 | 1 |
| 16 | 20 | 7 | 0 | 3 | 2 | 1 | 0 | 4 | 0.8 | 0.931 | 0.2 | 1 |
| 17 | 21 | 6 | 0 | 2 | 1 | 2 | 0 | 4 | 0.875 | 0.9643 | 0.3333 | 1 |
| 18 | 24 | 4 | 0 | 1 | 1 | 1 | 0 | 3 | 0.9231 | 0.9655 | 0.25 | 1 |
| 19 | 22 | 5 | 0 | 1 | 1 | 2 | 0 | 4 | 0.9167 | 0.9643 | 0.3333 | 1 |
| 20 | 24 | 3 | 0 | 0 | 0 | 3 | 0 | 3 | 1 | 1 | 0.5 | 1 |
| 21 | 18 | 9 | 0 | 0 | 0 | 3 | 0 | 9 | 1 | 1 | 0.25 | 1 |
| 22 | 25 | 5 | 0 | 0 | 0 | 0 | 0 | 5 | 1 | 1 | 0 | - |
| 23 | 21 | 7 | 0 | 1 | 0 | 2 | 0 | 6 | 0.9545 | 1 | 0.25 | 1 |
| 24 | 17 | 10 | 0 | 0 | 0 | 3 | 0 | 10 | 1 | 1 | 0.2308 | 1 |
| 25 | 22 | 5 | 0 | 0 | 0 | 3 | 0 | 5 | 1 | 1 | 0.375 | 1 |
| 26 | 16 | 10 | 0 | 0 | 0 | 4 | 0 | 10 | 1 | 1 | 0.2857 | 1 |
| 27 | 19 | 10 | 0 | 1 | 0 | 1 | 0 | 9 | 0.95 | 1 | 0.1 | 1 |
| 28 | 16 | 12 | 0 | 0 | 0 | 2 | 0 | 12 | 1 | 1 | 0.1429 | 1 |
| 29 | 16 | 11 | 0 | 1 | 0 | 3 | 0 | 10 | 0.9412 | 1 | 0.2308 | 1 |
| 30 | 11 | 15 | 0 | 0 | 0 | 4 | 0 | 15 | 1 | 1 | 0.2105 | 1 |
| 31 | 19 | 9 | 0 | 0 | 0 | 2 | 0 | 9 | 1 | 1 | 0.1818 | 1 |
| 32 | 21 | 8 | 0 | 0 | 0 | 1 | 0 | 8 | 1 | 1 | 0.1111 | 1 |
| 33 | 25 | 4 | 0 | 1 | 0 | 1 | 0 | 3 | 0.9615 | 1 | 0.25 | 1 |
| 34 | 24 | 6 | 0 | 1 | 0 | 0 | 0 | 5 | 0.96 | 1 | 0 | - |
| 35 | 24 | 3 | 0 | 0 | 0 | 3 | 0 | 3 | 1 | 1 | 0.5 | 1 |
| 36 | 20 | 6 | 0 | 1 | 0 | 4 | 0 | 5 | 0.9524 | 1 | 0.4444 | 1 |
| 37 | 22 | 6 | 0 | 1 | 0 | 2 | 0 | 5 | 0.9565 | 1 | 0.2857 | 1 |
| 38 | 21 | 5 | 0 | 0 | 0 | 4 | 0 | 5 | 1 | 1 | 0.4444 | 1 |
| **TOTAL** | **816** | **226** | **2** | **18** | **11** | **86** | **1** | **208** | **0.9657** | **0.9896** | **0.2915** | **0.9885** |

Supplementary Table 3.2.1: Detailed evaluation of the results of the CNN-based system with VGG-8-1D analysis (Stage 2) of the testing clinical sample Test-01-BS01.

**Test_01_BS01** (Sample ID 1)

| VOC Label | Start detection $\mathcal{sRT}$ | End detection $\mathcal{eRT}$ | Confidence $\mathcal{T}$ |
|---|---|---|---|
| 1 | 2.892 | 2.985 | 1.0000 |
| 2 | 3.033 | 3.134 | 1.0000 |
| 3 | 3.392 | 3.480 | 1.0000 |
| 4 | 3.482 | 3.589 | 1.0000 |
| 5 | 3.756 | 3.862 | 1.0000 |
| 6 | 3.891 | 4.027 | 0.9994 |
| 7 | 4.686 | 4.808 | 1.0000 |
| 8 | 4.935 | 5.025 | 1.0000 |
| 9 | 5.028 | 5.121 | 1.0000 |
| 10 | 5.216 | 5.341 | 1.0000 |
| 11 | 5.455 | 5.553 | 1.0000 |
| 12 | 5.556 | 5.670 | 0.9998 |
| 13 | 5.861 | 5.944 | 0.9998 |
| 14 | 6.275 | 6.371 | 1.0000 |
| 15 | 7.411 | 7.501 | 1.0000 |
| 16 | 7.838 | 7.914 | 0.9999 |
| 17 | 9.588 | 9.712 | 1.0000 |
| 18 | 10.243 | 10.359 | 1.0000 |
| 19 | 10.638 | 10.715 | 0.9974 |
| 20 | 11.364 | 11.447 | 1.0000 |
| 22 | 13.594 | 13.684 | 1.0000 |
| 23 | 16.248 | 16.325 | 1.0000 |
| 24 | 16.545 | 16.635 | 1.0000 |
| 26 | 19.712 | 19.837 | 1.0000 |
| 27 | 21.700 | 21.777 | 1.0000 |
| 28 | 22.808 | 22.896 | 1.0000 |
| 29 | 27.590 | 27.704 | 1.0000 |
| 30 | 41.972 | 42.084 | 1.0000 |

| | |
|---|---|
| (green) | **TP** |
| (yellow) | **TTP** |
| (red) | **FP** |

| | TN | TTN | FN |
|---|---|---|---|
| **VOC Label** | 25 | - | 21 |

Supplementary Table 3.2.2: Detailed evaluation of the results of the CNN-based system with VGG-8-1D analysis (Stage 2) of the testing clinical sample Test-01-BS02.

**Test_01_BS02** (Sample ID 2)

| VOC Label | Start detection $s\mathcal{RT}$ | End detection $e\mathcal{RT}$ | Confidence $\mathcal{T}$ |
|---|---|---|---|
| 1 | 2.894 | 2.984 | 1.0000 |
| 2 | 3.040 | 3.130 | 1.0000 |
| 3 | 3.396 | 3.481 | 1.0000 |
| 4 | 3.483 | 3.587 | 1.0000 |
| 5 | 3.759 | 3.863 | 1.0000 |
| 6 | 3.895 | 4.025 | 0.9994 |
| 7 | 4.691 | 4.808 | 1.0000 |
| 8 | 4.935 | 5.026 | 1.0000 |
| 9 | 5.028 | 5.121 | 1.0000 |
| 10 | 5.219 | 5.341 | 1.0000 |
| 11 | 5.458 | 5.556 | 1.0000 |
| 12 | 5.559 | 5.670 | 0.9998 |
| 13 | 5.862 | 5.949 | 1.0000 |
| 14 | 6.278 | 6.371 | 1.0000 |
| 15 | 7.414 | 7.501 | 1.0000 |
| 16 | 7.841 | 7.918 | 1.0000 |
| 17 | 9.589 | 9.713 | 1.0000 |
| 18 | 10.246 | 10.358 | 1.0000 |
| 19 | 10.633 | 10.713 | 0.9995 |
| 20 | 11.368 | 11.450 | 1.0000 |
| 22 | 13.600 | 13.687 | 1.0000 |
| 23 | 16.251 | 16.328 | 1.0000 |
| 24 | 16.545 | 16.638 | 1.0000 |
| 26 | 19.716 | 19.838 | 1.0000 |
| 27 | 21.701 | 21.781 | 1.0000 |
| 28 | 22.815 | 22.899 | 1.0000 |
| 29 | 27.599 | 27.710 | 1.0000 |
| 30 | 41.970 | 42.082 | 1.0000 |

| | |
|---|---|
| | **TP** |
| | **TTP** |
| | **FP** |

| | TN | TTN | FN |
|---|---|---|---|
| **VOC Label** | 25 | - | 21 |

Supplementary Table 3.2.3: Detailed evaluation of the results of the CNN-based system with VGG-8-1D analysis (Stage 2) of the testing clinical sample Test-01-BS03.

**Test_01_BS03** (Sample ID 3)

| VOC Label | Start detection $s\mathcal{RT}$ | End detection $e\mathcal{RT}$ | Confidence $\mathcal{T}$ |
|---|---|---|---|
| 1 | 2.891 | 2.984 | 1.0000 |
| 2 | 3.034 | 3.130 | 1.0000 |
| 3 | 3.390 | 3.475 | 1.0000 |
| 4 | 3.478 | 3.584 | 1.0000 |
| 5 | 3.754 | 3.858 | 1.0000 |
| 6 | 3.884 | 4.038 | 0.9994 |
| 7 | 4.686 | 4.800 | 1.0000 |
| 8 | 4.930 | 5.021 | 1.0000 |
| 9 | 5.023 | 5.116 | 1.0000 |
| 10 | 5.217 | 5.336 | 1.0000 |
| 11 | 5.451 | 5.551 | 1.0000 |
| 12 | 5.554 | 5.665 | 0.9998 |
| 13 | 5.859 | 5.944 | 1.0000 |
| 14 | 6.273 | 6.366 | 1.0000 |
| 15 | 7.403 | 7.499 | 1.0000 |
| 16 | 7.830 | 7.917 | 1.0000 |
| 17 | 9.582 | 9.710 | 1.0000 |
| 18 | 10.237 | 10.354 | 1.0000 |
| 19 | 10.622 | 10.709 | 1.0000 |
| 20 | 11.359 | 11.444 | 1.0000 |
| 21 | 11.756 | 11.812 | 0.9544 |
| 22 | 13.588 | 13.681 | 1.0000 |
| 23 | 16.242 | 16.321 | 1.0000 |
| 24 | 16.536 | 16.629 | 1.0000 |
| 26 | 19.711 | 19.830 | 1.0000 |
| 27 | 21.690 | 21.773 | 1.0000 |
| 28 | 22.804 | 22.891 | 1.0000 |
| 29 | 27.590 | 27.704 | 1.0000 |
| 30 | 41.957 | 42.066 | 1.0000 |

| Colour | Class |
|---|---|
| (green) | **TP** |
| (yellow) | **TTP** |
| (red) | **FP** |

| | TN | TTN | FN |
|---|---|---|---|
| **VOC Label** | 25 | 6, 21 | - |

Supplementary Table 3.2.4: Detailed evaluation of the results of the CNN-based system with VGG-8-1D analysis (Stage 2) of the testing clinical sample Test-01-BS04.

**Test_01_BS04** (Sample ID 4)

| VOC Label | Start detection $sRT$ | End detection $eRT$ | Confidence $T$ |
|---|---|---|---|
| 1 | 2.894 | 2.989 | 1.0000 |
| 2 | 3.035 | 3.138 | 1.0000 |
| 3 | 3.393 | 3.481 | 1.0000 |
| 4 | 3.484 | 3.590 | 1.0000 |
| 5 | 3.757 | 3.858 | 1.0000 |
| 6 | 3.882 | 4.023 | 0.9995 |
| 7 | 4.691 | 4.805 | 1.0000 |
| 8 | 4.933 | 5.026 | 1.0000 |
| 9 | 5.028 | 5.121 | 1.0000 |
| 10 | 5.219 | 5.341 | 1.0000 |
| 11 | 5.456 | 5.556 | 1.0000 |
| 12 | 5.559 | 5.670 | 0.9999 |
| 13 | 5.864 | 5.946 | 0.9994 |
| 14 | 6.281 | 6.365 | 1.0000 |
| 15 | 7.411 | 7.501 | 1.0000 |
| 16 | 7.835 | 7.923 | 1.0000 |
| 17 | 9.589 | 9.716 | 1.0000 |
| 18 | 10.246 | 10.358 | 1.0000 |
| 19 | 10.628 | 10.713 | 1.0000 |
| 20 | 11.365 | 11.450 | 1.0000 |
| 21 | 11.763 | 11.818 | 0.9576 |
| 22 | 13.595 | 13.688 | 1.0000 |
| 23 | 16.249 | 16.328 | 1.0000 |
| 24 | 16.543 | 16.636 | 1.0000 |
| 26 | 19.722 | 19.836 | 1.0000 |
| 27 | 21.700 | 21.779 | 1.0000 |
| 28 | 22.810 | 22.901 | 1.0000 |
| 29 | 27.592 | 27.711 | 1.0000 |
| 30 | 41.969 | 42.078 | 1.0000 |

| Colour | Meaning |
|---|---|
| (green) | TP |
| (yellow) | TTP |
| (red) | FP |

| | TN | TTN | FN |
|---|---|---|---|
| **VOC Label** | 25 | - | - |

Supplementary Table 3.2.5: Detailed evaluation of the results of the CNN-based system with VGG-8-1D analysis (Stage 2) of the testing clinical sample Test-01-ES.

**Test_01_ES** (Sample ID 5)

| VOC Label | Start detection $s\mathcal{RT}$ | End detection $e\mathcal{RT}$ | Confidence $\mathcal{T}$ |
|---|---|---|---|
| 1 | 2.915 | 2.992 | 0.9973 |
| 2 | 3.056 | 3.109 | 0.9474 |
| 3 | 3.420 | 3.473 | 0.9933 |
| 4 | 3.475 | 3.597 | 1.0000 |
| 5 | 3.746 | 3.862 | 1.0000 |
| 6 | 3.865 | 3.966 | 0.9991 |
| 8 | 4.917 | 5.015 | 1.0000 |
| 9 | 5.018 | 5.103 | 1.0000 |
| 11 | 5.466 | 5.537 | 0.9980 |
| 12 | 5.553 | 5.657 | 1.0000 |
| 15 | 7.421 | 7.474 | 0.9243 |
| 16 | 7.840 | 7.928 | 1.0000 |
| 17 | 9.583 | 9.703 | 1.0000 |
| 18 | 10.230 | 10.341 | 1.0000 |
| 19 | 10.600 | 10.709 | 1.0000 |
| 21 | 11.331 | 11.419 | 0.9986 |
| 22 | 13.587 | 13.680 | 1.0000 |
| 24 | 16.537 | 16.627 | 1.0000 |
| 26 | 19.705 | 19.829 | 1.0000 |
| 28 | 22.803 | 22.885 | 1.0000 |
| 29 | 27.586 | 27.702 | 1.0000 |
| 30 | 41.957 | 42.048 | 1.0000 |

| | |
|---|---|
| (green) | **TP** |
| (yellow) | **TTP** |
| (pink) | **FP** |

| | TN | TTN | FN |
|---|---|---|---|
| **VOC Label** | 7, 10, 13, 14, 20, 23, 25, 27 | - | - |

Supplementary Table 3.2.6: Detailed evaluation of the results of the CNN-based system with VGG-8-1D analysis (Stage 2) of the testing clinical sample Test-02-BS01.

**Test_02_BS01** (Sample ID 6)

| VOC Label | Start detection $sRT$ | End detection $eRT$ | Confidence $T$ |
|---|---|---|---|
| 1 | 2.881 | 2.982 | 1.0000 |
| 2 | 3.030 | 3.129 | 1.0000 |
| 3 | 3.370 | 3.477 | 1.0000 |
| 4 | 3.479 | 3.575 | 1.0000 |
| 5 | 3.745 | 3.856 | 1.0000 |
| 6 | 3.859 | 4.024 | 0.9995 |
| 7 | 4.693 | 4.781 | 1.0000 |
| 8 | 4.927 | 5.006 | 1.0000 |
| 9 | 5.009 | 5.110 | 1.0000 |
| 10 | 5.221 | 5.325 | 1.0000 |
| 11 | 5.447 | 5.532 | 0.9995 |
| 12 | 5.558 | 5.654 | 0.9996 |
| 13 | 5.853 | 5.927 | 1.0000 |
| 14 | 6.262 | 6.347 | 1.0000 |
| 15 | 7.389 | 7.464 | 0.9995 |
| 17 | 9.567 | 9.708 | 1.0000 |
| 18 | 10.226 | 10.321 | 1.0000 |
| 19 | 10.605 | 10.687 | 1.0000 |
| 20 | 11.347 | 11.432 | 1.0000 |
| 21 | 11.732 | 11.790 | 0.9656 |
| 22 | 13.563 | 13.659 | 1.0000 |
| 23 | 16.220 | 16.297 | 1.0000 |
| 24 | 16.516 | 16.601 | 1.0000 |
| 26 | 19.695 | 19.801 | 1.0000 |
| 27 | 21.669 | 21.746 | 1.0000 |
| 28 | 22.777 | 22.872 | 1.0000 |
| 29 | 27.565 | 27.684 | 1.0000 |
| 30 | 41.940 | 42.015 | 0.9917 |

| Colour | Meaning |
|---|---|
| (green) | TP |
| (yellow) | TTP |
| (red) | FP |

| | TN | TTN | FN |
|---|---|---|---|
| VOC Label | 16, 25 | 5 | - |

Supplementary Table 3.2.7: Detailed evaluation of the results of the CNN-based system with VGG-8-1D analysis (Stage 2) of the testing clinical sample Test-02-BS02.

**Test_02_BS02** (Sample ID 7)

| VOC Label | Start detection $s\mathcal{RT}$ | End detection $e\mathcal{RT}$ | Confidence $\mathcal{T}$ |
|---|---|---|---|
| 1 | 2.881 | 2.982 | 1.0000 |
| 2 | 3.033 | 3.128 | 1.0000 |
| 3 | 3.367 | 3.476 | 1.0000 |
| 4 | 3.479 | 3.580 | 1.0000 |
| 5 | 3.747 | 3.850 | 1.0000 |
| 6 | 3.874 | 4.020 | 0.9997 |
| 7 | 4.691 | 4.784 | 1.0000 |
| 8 | 4.922 | 5.007 | 1.0000 |
| 9 | 5.009 | 5.110 | 1.0000 |
| 10 | 5.216 | 5.320 | 1.0000 |
| 11 | 5.453 | 5.527 | 0.9886 |
| 12 | 5.553 | 5.652 | 0.9996 |
| 13 | 5.856 | 5.928 | 1.0000 |
| 14 | 6.264 | 6.344 | 1.0000 |
| 15 | 7.394 | 7.463 | 0.9988 |
| 17 | 9.568 | 9.709 | 1.0000 |
| 18 | 10.224 | 10.324 | 1.0000 |
| 19 | 10.613 | 10.687 | 0.9998 |
| 20 | 11.342 | 11.432 | 1.0000 |
| 21 | 11.732 | 11.790 | 0.9567 |
| 22 | 13.568 | 13.659 | 1.0000 |
| 23 | 16.219 | 16.299 | 1.0000 |
| 24 | 16.521 | 16.598 | 1.0000 |
| 26 | 19.710 | 19.797 | 0.9999 |
| 27 | 21.671 | 21.747 | 1.0000 |
| 28 | 22.786 | 22.868 | 1.0000 |
| 29 | 27.564 | 27.676 | 1.0000 |
| 30 | 41.931 | 42.029 | 1.0000 |

| Legend | |
|---|---|
| (green) | **TP** |
| (yellow) | **TTP** |
| (red) | **FP** |

| | TN | TTN | FN |
|---|---|---|---|
| **VOC Label** | 25 | - | 16 |

Supplementary Table 3.2.8: Detailed evaluation of the results of the CNN-based system with VGG-8-1D analysis (Stage 2) of the testing clinical sample Test-02-BS03.

**Test_02_BS03** (Sample ID 8)

| VOC Label | Start detection $sRT$ | End detection $eRT$ | Confidence $\mathcal{T}$ |
|---|---|---|---|
| 1 | 2.885 | 2.981 | 1.0000 |
| 2 | 3.034 | 3.132 | 1.0000 |
| 3 | 3.371 | 3.477 | 1.0000 |
| 4 | 3.480 | 3.581 | 1.0000 |
| 5 | 3.748 | 3.851 | 1.0000 |
| 6 | 3.872 | 4.037 | 1.0000 |
| 7 | 4.698 | 4.782 | 1.0000 |
| 8 | 4.923 | 5.008 | 1.0000 |
| 9 | 5.011 | 5.111 | 1.0000 |
| 10 | 5.220 | 5.321 | 1.0000 |
| 11 | 5.448 | 5.533 | 0.9993 |
| 12 | 5.555 | 5.653 | 0.9993 |
| 13 | 5.860 | 5.926 | 0.9999 |
| 14 | 6.271 | 6.343 | 1.0000 |
| 15 | 7.390 | 7.465 | 0.9994 |
| 17 | 9.570 | 9.707 | 1.0000 |
| 18 | 10.225 | 10.323 | 1.0000 |
| 19 | 10.617 | 10.691 | 1.0000 |
| 21 | 11.290 | 11.343 | 0.9795 |
| 20 | 11.346 | 11.433 | 1.0000 |
| 22 | 13.568 | 13.658 | 1.0000 |
| 23 | 16.222 | 16.299 | 1.0000 |
| 24 | 16.524 | 16.598 | 0.9999 |
| 26 | 19.702 | 19.800 | 1.0000 |
| 27 | 21.673 | 21.747 | 1.0000 |
| 28 | 22.783 | 22.868 | 1.0000 |
| 29 | 27.567 | 27.684 | 1.0000 |

| | |
|---|---|
| (green) | **TP** |
| (yellow) | **TTP** |
| (red) | **FP** |

| | TN | TTN | FN |
|---|---|---|---|
| **VOC Label** | 25, 30 | - | 16 |

Supplementary Table 3.2.9: Detailed evaluation of the results of the CNN-based system with VGG-8-1D analysis (Stage 2) of the testing clinical sample Test-02-BS04.

**Test_02_BS04** (Sample ID 9)

| VOC Label | Start detection $\mathcal{sRT}$ | End detection $\mathcal{eRT}$ | Confidence $\mathcal{T}$ |
|---|---|---|---|
| 1 | 2.886 | 2.979 | 1.0000 |
| 2 | 3.035 | 3.133 | 1.0000 |
| 3 | 3.382 | 3.478 | 1.0000 |
| 4 | 3.481 | 3.584 | 1.0000 |
| 5 | 3.748 | 3.852 | 1.0000 |
| 6 | 3.873 | 4.075 | 1.0000 |
| 7 | 4.695 | 4.785 | 1.0000 |
| 8 | 4.923 | 5.008 | 1.0000 |
| 9 | 5.011 | 5.114 | 1.0000 |
| 10 | 5.218 | 5.324 | 1.0000 |
| 11 | 5.448 | 5.533 | 0.9995 |
| 12 | 5.555 | 5.655 | 0.9996 |
| 13 | 5.857 | 5.923 | 0.9985 |
| 14 | 6.273 | 6.342 | 1.0000 |
| 15 | 7.390 | 7.472 | 1.0000 |
| 17 | 9.569 | 9.707 | 1.0000 |
| 18 | 10.224 | 10.325 | 1.0000 |
| 19 | 10.611 | 10.688 | 1.0000 |
| 20 | 11.343 | 11.435 | 1.0000 |
| 21 | 11.732 | 11.790 | 0.9659 |
| 22 | 13.569 | 13.662 | 1.0000 |
| 23 | 16.220 | 16.299 | 1.0000 |
| 24 | 16.522 | 16.599 | 0.9999 |
| 26 | 19.711 | 19.798 | 1.0000 |
| 27 | 21.668 | 21.748 | 1.0000 |
| 28 | 22.784 | 22.869 | 1.0000 |
| 29 | 27.564 | 27.683 | 1.0000 |
| 30 | 41.926 | 42.029 | 1.0000 |

| | |
|---|---|
| | **TP** |
| | **TTP** |
| | **FP** |

| | **TN** | **TTN** | **FN** |
|---|---|---|---|
| **VOC Label** | 16, 25 | - | - |

Supplementary Table 3.2.10: Detailed evaluation of the results of the CNN-based system with VGG-8-1D analysis (Stage 2) of the testing clinical sample Test-02-ES.

**Test_02_ES** (Sample ID 10)

| VOC Label | Start detection $s\mathcal{RT}$ | End detection $e\mathcal{RT}$ | Confidence $\mathcal{T}$ |
|---|---|---|---|
| 1 | 2.897 | 2.996 | 1.0000 |
| 3 | 3.415 | 3.468 | 0.9900 |
| 4 | 3.471 | 3.590 | 1.0000 |
| 5 | 3.741 | 3.858 | 1.0000 |
| 6 | 3.861 | 3.927 | 0.9802 |
| 8 | 4.911 | 5.009 | 1.0000 |
| 9 | 5.012 | 5.094 | 1.0000 |
| 10 | 5.216 | 5.303 | 0.9872 |
| 12 | 5.569 | 5.648 | 0.9921 |
| 15 | 7.418 | 7.469 | 0.7724 |
| 16 | 7.840 | 7.890 | 0.8811 |
| 17 | 9.572 | 9.694 | 1.0000 |
| 18 | 10.223 | 10.329 | 1.0000 |
| 19 | 10.615 | 10.689 | 0.9947 |
| 21 | 11.333 | 11.402 | 0.9218 |
| 22 | 13.600 | 13.669 | 0.9975 |
| 26 | 19.720 | 19.802 | 0.9996 |
| 28 | 22.804 | 22.873 | 0.9980 |
| 29 | 27.570 | 27.676 | 0.9999 |

| | |
|---|---|
| | **TP** |
| | **TTP** |
| | **FP** |

| | TN | TTN | FN |
|---|---|---|---|
| **VOC Label** | 2, 7, 11, 13, 14, 23, 24, 25, 27, 30 | - | 20 |

Supplementary Table 3.2.11: Detailed evaluation of the results of the CNN-based system with VGG-8-1D analysis (Stage 2) of the testing clinical sample Test-03-BS01.

**Test_03_BS01** (Sample ID 11)

| VOC Label | Start detection $s\mathcal{RT}$ | End detection $e\mathcal{RT}$ | Confidence $\mathcal{T}$ |
|---|---|---|---|
| 1 | 2.869 | 2.954 | 1.0000 |
| 2 | 3.005 | 3.087 | 1.0000 |
| 3 | 3.351 | 3.425 | 1.0000 |
| 4 | 3.428 | 3.539 | 1.0000 |
| 5 | 3.680 | 3.792 | 1.0000 |
| 6 | 3.805 | 3.959 | 0.9992 |
| 7 | 4.621 | 4.674 | 0.9886 |
| 8 | 4.829 | 4.906 | 1.0000 |
| 9 | 4.908 | 4.996 | 1.0000 |
| 10 | 5.126 | 5.230 | 1.0000 |
| 11 | 5.232 | 5.424 | 1.0000 |
| 12 | 5.426 | 5.530 | 0.9998 |
| 13 | 5.724 | 5.801 | 1.0000 |
| 14 | 6.122 | 6.210 | 1.0000 |
| 15 | 7.238 | 7.325 | 1.0000 |
| 16 | 7.662 | 7.745 | 1.0000 |
| 17 | 9.393 | 9.499 | 0.9999 |
| 18 | 10.035 | 10.150 | 1.0000 |
| 19 | 10.404 | 10.495 | 1.0000 |
| 20 | 11.129 | 11.222 | 1.0000 |
| 21 | 11.514 | 11.569 | 0.9034 |
| 22 | 13.355 | 13.445 | 1.0000 |
| 23 | 15.987 | 16.067 | 1.0000 |
| 24 | 16.295 | 16.383 | 1.0000 |
| 26 | 19.493 | 19.594 | 1.0000 |
| 27 | 21.435 | 21.509 | 1.0000 |
| 28 | 22.578 | 22.652 | 0.9973 |
| 29 | 27.334 | 27.448 | 1.0000 |
| 30 | 41.686 | 41.763 | 0.9923 |

| | |
|---|---|
| (green) | **TP** |
| (yellow) | **TTP** |
| (red) | **FP** |

| | TN | TTN | FN |
|---|---|---|---|
| **VOC Label** | 25 | - | - |

Supplementary Table 3.2.12: Detailed evaluation of the results of the CNN-based system with VGG-8-1D analysis (Stage 2) of the testing clinical sample Test-03-BS02.

**Test_03_BS02** (Sample ID 12)

| VOC Label | Start detection $sRT$ | End detection $eRT$ | Confidence $T$ |
|---|---|---|---|
| 1 | 2.865 | 2.947 | 1.0000 |
| 2 | 3.003 | 3.082 | 1.0000 |
| 3 | 3.340 | 3.423 | 1.0000 |
| 4 | 3.425 | 3.539 | 1.0000 |
| 5 | 3.678 | 3.781 | 1.0000 |
| 6 | 3.813 | 3.949 | 0.9992 |
| 7 | 4.615 | 4.665 | 0.9573 |
| 8 | 4.820 | 4.905 | 1.0000 |
| 9 | 4.907 | 4.992 | 1.0000 |
| 10 | 5.112 | 5.226 | 1.0000 |
| 11 | 5.228 | 5.420 | 1.0000 |
| 12 | 5.422 | 5.523 | 0.9998 |
| 13 | 5.712 | 5.794 | 1.0000 |
| 14 | 6.110 | 6.205 | 1.0000 |
| 15 | 7.232 | 7.325 | 1.0000 |
| 16 | 7.662 | 7.739 | 1.0000 |
| 17 | 9.386 | 9.495 | 1.0000 |
| 18 | 10.031 | 10.143 | 1.0000 |
| 19 | 10.403 | 10.487 | 1.0000 |
| 20 | 11.121 | 11.217 | 1.0000 |
| 21 | 11.501 | 11.559 | 0.8859 |
| 22 | 13.349 | 13.440 | 1.0000 |
| 23 | 15.981 | 16.060 | 1.0000 |
| 24 | 16.294 | 16.371 | 1.0000 |
| 26 | 19.474 | 19.591 | 1.0000 |
| 27 | 21.421 | 21.503 | 1.0000 |
| 28 | 22.561 | 22.641 | 0.9997 |
| 29 | 27.328 | 27.432 | 1.0000 |
| 30 | 41.679 | 41.775 | 1.0000 |

| Colour | Category |
|---|---|
| (green) | TP |
| (yellow) | TTP |
| (red) | FP |

| | TN | TTN | FN |
|---|---|---|---|
| VOC Label | 25 | 15 | - |

Supplementary Table 3.2.13: Detailed evaluation of the results of the CNN-based system with VGG-8-1D analysis (Stage 2) of the testing clinical sample Test-03-BS03.

**Test_03_BS03** (Sample ID 13)

| VOC Label | Start detection $s\mathcal{RT}$ | End detection $e\mathcal{RT}$ | Confidence $\mathcal{T}$ |
|---|---|---|---|
| 1 | 2.865 | 2.952 | 1.0000 |
| 2 | 3.005 | 3.088 | 1.0000 |
| 3 | 3.343 | 3.425 | 1.0000 |
| 4 | 3.428 | 3.542 | 1.0000 |
| 5 | 3.683 | 3.784 | 1.0000 |
| 6 | 3.813 | 3.954 | 0.9993 |
| 7 | 4.623 | 4.673 | 0.9360 |
| 8 | 4.819 | 4.907 | 1.0000 |
| 9 | 4.910 | 4.997 | 1.0000 |
| 10 | 5.111 | 5.218 | 1.0000 |
| 11 | 5.321 | 5.422 | 1.0000 |
| 12 | 5.425 | 5.528 | 0.9999 |
| 13 | 5.717 | 5.799 | 1.0000 |
| 14 | 6.117 | 6.208 | 1.0000 |
| 15 | 7.237 | 7.312 | 0.9999 |
| 16 | 7.540 | 7.612 | 0.9951 |
| 17 | 9.384 | 9.498 | 1.0000 |
| 18 | 10.034 | 10.148 | 1.0000 |
| 19 | 10.402 | 10.490 | 1.0000 |
| 20 | 11.126 | 11.219 | 1.0000 |
| 21 | 11.511 | 11.567 | 0.9277 |
| 22 | 13.352 | 13.444 | 1.0000 |
| 23 | 15.985 | 16.062 | 1.0000 |
| 24 | 16.296 | 16.378 | 1.0000 |
| 26 | 19.465 | 19.590 | 1.0000 |
| 27 | 21.425 | 21.502 | 1.0000 |
| 28 | 22.573 | 22.642 | 0.9964 |
| 29 | 27.327 | 27.436 | 1.0000 |
| 30 | 41.672 | 41.781 | 1.0000 |

| | |
|---|---|
| (green) | TP |
| (yellow) | TTP |
| (red) | FP |

| | TN | TTN | FN |
|---|---|---|---|
| VOC Label | 25 | - | - |

Supplementary Table 3.2.14: Detailed evaluation of the results of the CNN-based system with VGG-8-1D analysis (Stage 2) of the testing clinical sample Test-03-BS04.

**Test_03_BS04** (Sample ID 14)

| VOC Label | Start detection $sRT$ | End detection $eRT$ | Confidence $T$ |
|---|---|---|---|
| 1 | 2.861 | 2.949 | 1.0000 |
| 2 | 3.010 | 3.093 | 1.0000 |
| 3 | 3.340 | 3.425 | 1.0000 |
| 4 | 3.427 | 3.542 | 1.0000 |
| 5 | 3.680 | 3.781 | 1.0000 |
| 6 | 3.810 | 3.953 | 0.9994 |
| 7 | 4.585 | 4.686 | 1.0000 |
| 8 | 4.816 | 4.901 | 1.0000 |
| 9 | 4.903 | 4.996 | 1.0000 |
| 10 | 5.094 | 5.214 | 1.0000 |
| 11 | 5.320 | 5.418 | 1.0000 |
| 12 | 5.421 | 5.522 | 0.9998 |
| 13 | 5.710 | 5.795 | 1.0000 |
| 14 | 6.113 | 6.204 | 1.0000 |
| 15 | 7.230 | 7.313 | 1.0000 |
| 16 | 7.657 | 7.716 | 0.9924 |
| 17 | 9.381 | 9.493 | 1.0000 |
| 18 | 10.026 | 10.148 | 1.0000 |
| 19 | 10.405 | 10.484 | 1.0000 |
| 20 | 11.121 | 11.216 | 1.0000 |
| 21 | 11.500 | 11.561 | 0.9249 |
| 22 | 13.356 | 13.435 | 1.0000 |
| 23 | 15.978 | 16.058 | 1.0000 |
| 24 | 16.299 | 16.368 | 0.9996 |
| 26 | 19.462 | 19.587 | 1.0000 |
| 27 | 21.421 | 21.504 | 1.0000 |
| 28 | 22.559 | 22.643 | 1.0000 |
| 29 | 27.322 | 27.439 | 1.0000 |
| 30 | 41.671 | 41.772 | 1.0000 |

| Colour | Class |
|---|---|
| (green) | TP |
| (yellow) | TTP |
| (red) | FP |

| | TN | TTN | FN |
|---|---|---|---|
| VOC Label | 25 | - | - |

Supplementary Table 3.2.15: Detailed evaluation of the results of the CNN-based system with VGG-8-1D analysis (Stage 2) of the testing clinical sample Test-03-ES.

**Test_03_ES** (Sample ID 15)

| VOC Label | Start detection $sRT$ | End detection $eRT$ | Confidence $T$ |
|---|---|---|---|
| 1 | 2.856 | 2.976 | 1.0000 |
| 2 | 3.034 | 3.090 | 0.9810 |
| 3 | 3.377 | 3.430 | 0.9750 |
| 4 | 3.432 | 3.539 | 1.0000 |
| 5 | 3.685 | 3.796 | 1.0000 |
| 6 | 3.799 | 3.953 | 1.0000 |
| 8 | 4.815 | 4.913 | 1.0000 |
| 9 | 4.916 | 5.003 | 1.0000 |
| 10 | 5.102 | 5.192 | 0.9998 |
| 11 | 5.340 | 5.420 | 0.9986 |
| 12 | 5.430 | 5.531 | 1.0000 |
| 13 | 5.730 | 5.804 | 1.0000 |
| 15 | 7.245 | 7.319 | 1.0000 |
| 16 | 7.552 | 7.616 | 0.9934 |
| 17 | 9.398 | 9.498 | 1.0000 |
| 18 | 10.053 | 10.132 | 1.0000 |
| 19 | 10.405 | 10.493 | 1.0000 |
| 21 | 11.081 | 11.163 | 0.9997 |
| 20 | 11.166 | 11.232 | 0.9673 |
| 22 | 13.356 | 13.451 | 1.0000 |
| 23 | 15.991 | 16.073 | 1.0000 |
| 24 | 16.296 | 16.389 | 1.0000 |
| 25 | 16.786 | 16.895 | 1.0000 |
| 26 | 19.483 | 19.598 | 1.0000 |
| 27 | 21.427 | 21.512 | 1.0000 |
| 28 | 22.563 | 22.655 | 1.0000 |
| 29 | 27.338 | 27.447 | 1.0000 |
| 30 | 41.681 | 41.788 | 1.0000 |

| Colour | Class |
|---|---|
| (green) | **TP** |
| (yellow) | **TTP** |
| (red) | **FP** |

| | TN | TTN | FN |
|---|---|---|---|
| **VOC Label** | 7, 14 | - | 16 |

Supplementary Table 3.2.16: Detailed evaluation of the results of the CNN-based system with VGG-8-1D analysis (Stage 2) of the testing clinical sample Test-04-BS01.

**Test_04_BS01** (Sample ID 16)

| VOC Label | Start detection $s\mathcal{RT}$ | End detection $e\mathcal{RT}$ | Confidence $\mathcal{T}$ |
|---|---|---|---|
| 1 | 3.146 | 3.306 | 1.0000 |
| 2 | 3.373 | 3.509 | 1.0000 |
| 3 | 4.005 | 4.088 | 1.0000 |
| 4 | 4.090 | 4.176 | 1.0000 |
| 5 | 4.576 | 4.683 | 1.0000 |
| 6 | 4.827 | 4.920 | 0.9980 |
| 7 | 5.914 | 6.023 | 1.0000 |
| 8 | 6.258 | 6.351 | 1.0000 |
| 9 | 6.354 | 6.453 | 1.0000 |
| 10 | 6.621 | 6.728 | 1.0000 |
| 11 | 6.968 | 7.048 | 0.9989 |
| 12 | 7.051 | 7.123 | 1.0000 |
| 13 | 7.521 | 7.601 | 1.0000 |
| 15 | 9.341 | 9.419 | 0.9990 |
| 16 | 9.743 | 9.844 | 1.0000 |
| 17 | 11.633 | 11.734 | 1.0000 |
| 19 | 12.815 | 12.900 | 1.0000 |
| 21 | 13.609 | 13.691 | 0.9686 |
| 20 | 13.694 | 13.776 | 1.0000 |
| 22 | 15.903 | 15.985 | 1.0000 |
| 23 | 18.679 | 18.753 | 1.0000 |
| 24 | 18.918 | 18.995 | 1.0000 |
| 26 | 22.177 | 22.241 | 0.9718 |
| 27 | 24.161 | 24.243 | 1.0000 |
| 28 | 25.393 | 25.456 | 0.9490 |
| 29 | 30.186 | 30.303 | 1.0000 |
| 30 | 44.662 | 44.793 | 1.0000 |

| | |
|---|---|
| | TP |
| | TTP |
| | FP |

| | TN | TTN | FN |
|---|---|---|---|
| VOC Label | 25 | 10, 16, 21 | 14, 18 |

Supplementary Table 3.2.17: Detailed evaluation of the results of the CNN-based system with VGG-8-1D analysis (Stage 2) of the testing clinical sample Test-04-BS02.

**Test_04_BS02** (Sample ID 17)

| VOC Label | Start detection $s\mathcal{RT}$ | End detection $e\mathcal{RT}$ | Confidence $\mathcal{T}$ |
|---|---|---|---|
| 1 | 3.138 | 3.303 | 1.0000 |
| 2 | 3.370 | 3.519 | 1.0000 |
| 3 | 3.994 | 4.085 | 1.0000 |
| 4 | 4.087 | 4.181 | 1.0000 |
| 5 | 4.573 | 4.792 | 1.0000 |
| 6 | 4.824 | 4.888 | 0.9978 |
| 7 | 5.915 | 6.030 | 1.0000 |
| 8 | 6.259 | 6.357 | 1.0000 |
| 9 | 6.360 | 6.461 | 1.0000 |
| 10 | 6.629 | 6.738 | 1.0000 |
| 11 | 6.974 | 7.059 | 0.9980 |
| 12 | 7.062 | 7.128 | 1.0000 |
| 13 | 7.535 | 7.612 | 1.0000 |
| 14 | 8.053 | 8.146 | 1.0000 |
| 15 | 9.323 | 9.427 | 1.0000 |
| 16 | 9.748 | 9.846 | 1.0000 |
| 17 | 11.635 | 11.730 | 1.0000 |
| 19 | 12.819 | 12.901 | 1.0000 |
| 21 | 13.634 | 13.700 | 0.9703 |
| 20 | 13.703 | 13.785 | 1.0000 |
| 22 | 15.903 | 15.988 | 1.0000 |
| 23 | 18.682 | 18.759 | 1.0000 |
| 24 | 18.921 | 18.998 | 1.0000 |
| 26 | 22.177 | 22.244 | 0.9728 |
| 27 | 24.164 | 24.247 | 1.0000 |
| 29 | 30.184 | 30.311 | 1.0000 |
| 30 | 44.669 | 44.790 | 1.0000 |

| Colour | Class |
|---|---|
| (green) | **TP** |
| (yellow) | **TTP** |
| (pink) | **FP** |

| | TN | TTN | FN |
|---|---|---|---|
| **VOC Label** | 25, 28 | 13, 21 | 18 |

Supplementary Table 3.2.18: Detailed evaluation of the results of the CNN-based system with VGG-8-1D analysis (Stage 2) of the testing clinical sample Test-04-BS03.

**Test_04_BS03** (Sample ID 18)

| VOC Label | Start detection $sRT$ | End detection $eRT$ | Confidence $T$ |
|---|---|---|---|
| 1 | 3.153 | 3.300 | 1.0000 |
| 2 | 3.372 | 3.521 | 1.0000 |
| 3 | 3.993 | 4.087 | 1.0000 |
| 4 | 4.089 | 4.183 | 1.0000 |
| 5 | 4.575 | 4.794 | 1.0000 |
| 6 | 4.826 | 4.893 | 0.9984 |
| 7 | 5.914 | 6.015 | 0.9996 |
| 8 | 6.273 | 6.364 | 1.0000 |
| 9 | 6.366 | 6.467 | 1.0000 |
| 10 | 6.632 | 6.720 | 1.0000 |
| 11 | 6.980 | 7.065 | 0.9950 |
| 12 | 7.068 | 7.142 | 1.0000 |
| 13 | 7.541 | 7.615 | 1.0000 |
| 14 | 8.058 | 8.151 | 1.0000 |
| 15 | 9.326 | 9.432 | 1.0000 |
| 16 | 9.753 | 9.849 | 1.0000 |
| 17 | 11.638 | 11.736 | 1.0000 |
| 19 | 12.822 | 12.906 | 1.0000 |
| 21 | 13.618 | 13.705 | 0.9994 |
| 20 | 13.708 | 13.798 | 1.0000 |
| 22 | 15.906 | 15.991 | 1.0000 |
| 23 | 18.685 | 18.762 | 1.0000 |
| 24 | 18.930 | 19.001 | 0.9994 |
| 26 | 22.184 | 22.248 | 0.9743 |
| 27 | 24.172 | 24.251 | 1.0000 |
| 28 | 25.356 | 25.441 | 0.9996 |
| 29 | 30.190 | 30.320 | 1.0000 |
| 30 | 44.679 | 44.789 | 1.0000 |

| Colour | Class |
|---|---|
| (green) | TP |
| (yellow) | TTP |
| (red) | FP |

| | TN | TTN | FN |
|---|---|---|---|
| VOC Label | 25 | 21 | 18 |

Supplementary Table 3.2.19: Detailed evaluation of the results of the CNN-based system with VGG-8-1D analysis (Stage 2) of the testing clinical sample Test-04-BS04.

**Test_04_BS04** (Sample ID 19)

| VOC Label | Start detection $sRT$ | End detection $eRT$ | Confidence $T$ |
|---|---|---|---|
| 1 | 3.139 | 3.301 | 1.0000 |
| 2 | 3.368 | 3.517 | 1.0000 |
| 3 | 3.995 | 4.085 | 1.0000 |
| 4 | 4.088 | 4.179 | 1.0000 |
| 5 | 4.571 | 4.784 | 1.0000 |
| 6 | 4.825 | 4.881 | 0.9816 |
| 7 | 5.927 | 6.002 | 0.9567 |
| 8 | 6.258 | 6.357 | 1.0000 |
| 9 | 6.359 | 6.458 | 1.0000 |
| 10 | 6.626 | 6.733 | 1.0000 |
| 11 | 6.773 | 6.837 | 0.9674 |
| 12 | 7.056 | 7.130 | 1.0000 |
| 13 | 7.532 | 7.609 | 1.0000 |
| 14 | 8.053 | 8.143 | 1.0000 |
| 15 | 9.332 | 9.428 | 1.0000 |
| 16 | 9.755 | 9.848 | 1.0000 |
| 17 | 11.640 | 11.740 | 1.0000 |
| 19 | 12.821 | 12.909 | 1.0000 |
| 21 | 13.602 | 13.702 | 0.9953 |
| 20 | 13.705 | 13.790 | 1.0000 |
| 22 | 15.908 | 15.993 | 1.0000 |
| 23 | 18.687 | 18.764 | 1.0000 |
| 24 | 18.924 | 19.003 | 1.0000 |
| 26 | 22.183 | 22.247 | 0.9715 |
| 27 | 24.171 | 24.253 | 1.0000 |
| 29 | 30.191 | 30.321 | 1.0000 |
| 30 | 44.678 | 44.795 | 1.0000 |

| Legend |
|---|
| TP |
| TTP |
| FP |

| | TN | TTN | FN |
|---|---|---|---|
| VOC Label | 25, 28 | 11 | 18 |

Supplementary Table 3.2.20: Detailed evaluation of the results of the CNN-based system with VGG-8-1D analysis (Stage 2) of the testing clinical sample Test-04-ES.

**Test_04_ES** (Sample ID 20)

| VOC Label | Start detection $sRT$ | End detection $eRT$ | Confidence $T$ |
|---|---|---|---|
| 1 | 3.129 | 3.336 | 1.0000 |
| 2 | 3.416 | 3.506 | 1.0000 |
| 3 | 4.037 | 4.088 | 0.9765 |
| 4 | 4.090 | 4.196 | 1.0000 |
| 5 | 4.592 | 4.709 | 1.0000 |
| 6 | 4.786 | 4.910 | 1.0000 |
| 8 | 6.277 | 6.378 | 1.0000 |
| 9 | 6.381 | 6.476 | 1.0000 |
| 10 | 6.686 | 6.760 | 0.9926 |
| 12 | 7.039 | 7.140 | 1.0000 |
| 13 | 7.567 | 7.628 | 0.9364 |
| 14 | 8.079 | 8.156 | 0.9999 |
| 15 | 9.323 | 9.429 | 1.0000 |
| 16 | 9.758 | 9.862 | 1.0000 |
| 17 | 11.636 | 11.748 | 1.0000 |
| 18 | 12.369 | 12.464 | 1.0000 |
| 19 | 12.814 | 12.918 | 1.0000 |
| 21 | 13.581 | 13.682 | 1.0000 |
| 20 | 13.706 | 13.799 | 1.0000 |
| 22 | 15.906 | 16.005 | 1.0000 |
| 23 | 18.692 | 18.772 | 1.0000 |
| 24 | 18.923 | 19.016 | 1.0000 |
| 25 | 19.447 | 19.561 | 1.0000 |
| 26 | 22.271 | 22.332 | 0.9467 |
| 27 | 24.179 | 24.261 | 1.0000 |
| 28 | 25.348 | 25.446 | 1.0000 |
| 29 | 30.200 | 30.325 | 1.0000 |

| Colour | Meaning |
|---|---|
| (green) | **TP** |
| (yellow) | **TTP** |
| (red) | **FP** |

| | TN | TTN | FN |
|---|---|---|---|
| **VOC Label** | 7, 11, 30 | - | - |

Supplementary Table 3.2.21: Detailed evaluation of the results of the CNN-based system with VGG-8-1D analysis (Stage 2) of the testing clinical sample Test-05-BS01.

**Test_05_BS01** (Sample ID 21)

| VOC Label | Start detection $s\mathcal{RT}$ | End detection $e\mathcal{RT}$ | Confidence $\mathcal{T}$ |
|---|---|---|---|
| 1 | 3.114 | 3.256 | 0.9961 |
| 2 | 3.382 | 3.513 | 1.0000 |
| 3 | 3.934 | 4.024 | 1.0000 |
| 4 | 4.027 | 4.107 | 1.0000 |
| 5 | 4.480 | 4.589 | 1.0000 |
| 6 | 4.731 | 4.811 | 0.9867 |
| 7 | 5.757 | 5.848 | 0.9994 |
| 8 | 6.093 | 6.181 | 1.0000 |
| 9 | 6.184 | 6.280 | 1.0000 |
| 10 | 6.437 | 6.557 | 1.0000 |
| 11 | 6.589 | 6.744 | 0.9999 |
| 13 | 7.329 | 7.406 | 1.0000 |
| 14 | 7.828 | 7.924 | 1.0000 |
| 15 | 9.071 | 9.162 | 1.0000 |
| 16 | 9.468 | 9.572 | 0.9982 |
| 17 | 11.300 | 11.433 | 1.0000 |
| 18 | 12.033 | 12.129 | 1.0000 |
| 19 | 12.509 | 12.593 | 1.0000 |
| 21 | 13.299 | 13.376 | 0.9279 |
| 20 | 13.389 | 13.487 | 1.0000 |
| 22 | 15.590 | 15.664 | 0.9999 |
| 23 | 18.360 | 18.440 | 1.0000 |
| 24 | 18.588 | 18.663 | 0.9999 |
| 26 | 21.881 | 21.945 | 0.9610 |
| 27 | 23.838 | 23.918 | 1.0000 |
| 29 | 29.791 | 29.903 | 1.0000 |
| 30 | 44.251 | 44.347 | 1.0000 |

| | |
|---|---|
| | **TP** |
| | **TTP** |
| | **FP** |

| | TN | TTN | FN |
|---|---|---|---|
| **VOC Label** | 12, 25, 28 | - | - |

Supplementary Table 3.2.22: Detailed evaluation of the results of the CNN-based system with VGG-8-1D analysis (Stage 2) of the testing clinical sample Test-05-BS02.

**Test_05_BS02** (Sample ID 22)

| VOC Label | Start detection $sRT$ | End detection $eRT$ | Confidence $\mathcal{T}$ |
|---|---|---|---|
| 1 | 3.117 | 3.271 | 1.0000 |
| 2 | 3.338 | 3.492 | 1.0000 |
| 3 | 3.930 | 4.025 | 1.0000 |
| 4 | 4.028 | 4.110 | 1.0000 |
| 5 | 4.473 | 4.699 | 1.0000 |
| 6 | 4.723 | 4.784 | 0.9861 |
| 7 | 5.749 | 5.866 | 1.0000 |
| 8 | 6.091 | 6.184 | 1.0000 |
| 9 | 6.187 | 6.280 | 1.0000 |
| 10 | 6.428 | 6.558 | 1.0000 |
| 11 | 6.561 | 6.688 | 0.9988 |
| 12 | 6.855 | 6.924 | 0.9733 |
| 13 | 7.340 | 7.409 | 1.0000 |
| 14 | 7.839 | 7.929 | 1.0000 |
| 15 | 9.056 | 9.154 | 1.0000 |
| 16 | 9.475 | 9.555 | 0.9992 |
| 17 | 11.313 | 11.422 | 1.0000 |
| 18 | 12.037 | 12.146 | 1.0000 |
| 19 | 12.504 | 12.594 | 1.0000 |
| 21 | 13.275 | 13.382 | 1.0000 |
| 20 | 13.384 | 13.485 | 1.0000 |
| 22 | 15.578 | 15.668 | 1.0000 |
| 23 | 18.362 | 18.444 | 1.0000 |
| 24 | 18.582 | 18.667 | 1.0000 |
| 25 | 19.095 | 19.180 | 1.0000 |
| 26 | 21.885 | 21.951 | 0.9832 |
| 27 | 23.839 | 23.921 | 1.0000 |
| 28 | 24.949 | 25.050 | 1.0000 |
| 29 | 29.787 | 29.920 | 1.0000 |
| 30 | 44.246 | 44.371 | 1.0000 |

| Colour | Category |
|---|---|
| (green) | **TP** |
| (yellow) | **TTP** |
| (red) | **FP** |

| | TN | TTN | FN |
|---|---|---|---|
| **VOC Label** | - | - | - |

Supplementary Table 3.2.23: Detailed evaluation of the results of the CNN-based system with VGG-8-1D analysis (Stage 2) of the testing clinical sample Test-05-BS03.

**Test_05_BS03** (Sample ID 23)

| VOC Label | Start detection $s\mathcal{RT}$ | End detection $e\mathcal{RT}$ | Confidence $\mathcal{T}$ |
|---|---|---|---|
| 1 | 3.072 | 3.267 | 1.0000 |
| 2 | 3.331 | 3.485 | 1.0000 |
| 3 | 3.912 | 4.011 | 1.0000 |
| 4 | 4.013 | 4.096 | 1.0000 |
| 5 | 4.461 | 4.680 | 1.0000 |
| 6 | 4.712 | 4.773 | 0.9886 |
| 7 | 5.750 | 5.843 | 0.9889 |
| 8 | 6.080 | 6.174 | 1.0000 |
| 9 | 6.176 | 6.273 | 1.0000 |
| 10 | 6.425 | 6.545 | 1.0000 |
| 11 | 6.587 | 6.750 | 0.9999 |
| 12 | 6.854 | 6.929 | 1.0000 |
| 13 | 7.319 | 7.396 | 1.0000 |
| 14 | 7.824 | 7.920 | 1.0000 |
| 15 | 9.065 | 9.161 | 1.0000 |
| 16 | 9.464 | 9.562 | 0.9989 |
| 17 | 11.319 | 11.428 | 1.0000 |
| 18 | 12.038 | 12.147 | 1.0000 |
| 19 | 12.502 | 12.598 | 1.0000 |
| 21 | 13.282 | 13.383 | 1.0000 |
| 20 | 13.385 | 13.481 | 1.0000 |
| 22 | 15.581 | 15.669 | 1.0000 |
| 23 | 18.362 | 18.441 | 1.0000 |
| 24 | 18.579 | 18.669 | 1.0000 |
| 26 | 21.884 | 21.948 | 0.9723 |
| 27 | 23.837 | 23.920 | 1.0000 |
| 29 | 29.787 | 29.917 | 1.0000 |
| 30 | 44.244 | 44.364 | 1.0000 |

| | |
|---|---|
| (green) | **TP** |
| (yellow) | **TTP** |
| (red) | **FP** |

| | TN | TTN | FN |
|---|---|---|---|
| **VOC Label** | 25, 28 | 11 | - |

Supplementary Table 3.2.24: Detailed evaluation of the results of the CNN-based system with VGG-8-1D analysis (Stage 2) of the testing clinical sample Test-05-BS04.

**Test_05_BS04** (Sample ID 24)

| VOC Label | Start detection $sRT$ | End detection $eRT$ | Confidence $\mathcal{T}$ |
|---|---|---|---|
| 1 | 3.153 | 3.269 | 0.9892 |
| 2 | 3.416 | 3.539 | 1.0000 |
| 3 | 3.984 | 4.069 | 1.0000 |
| 4 | 4.072 | 4.157 | 1.0000 |
| 5 | 4.533 | 4.637 | 1.0000 |
| 6 | 4.778 | 4.842 | 0.8617 |
| 7 | 5.810 | 5.921 | 1.0000 |
| 8 | 6.151 | 6.236 | 1.0000 |
| 9 | 6.239 | 6.329 | 1.0000 |
| 10 | 6.495 | 6.612 | 1.0000 |
| 11 | 6.660 | 6.809 | 0.9987 |
| 13 | 7.379 | 7.464 | 0.9995 |
| 14 | 7.892 | 7.977 | 1.0000 |
| 15 | 9.144 | 9.211 | 0.9907 |
| 16 | 9.522 | 9.621 | 0.9548 |
| 17 | 11.353 | 11.491 | 1.0000 |
| 18 | 12.105 | 12.203 | 0.9999 |
| 19 | 12.578 | 12.658 | 0.9999 |
| 21 | 13.351 | 13.449 | 1.0000 |
| 20 | 13.452 | 13.547 | 1.0000 |
| 22 | 15.648 | 15.736 | 1.0000 |
| 23 | 18.425 | 18.502 | 1.0000 |
| 24 | 18.651 | 18.736 | 1.0000 |
| 26 | 21.942 | 22.003 | 0.9537 |
| 27 | 23.902 | 23.984 | 1.0000 |
| 29 | 29.880 | 29.981 | 0.9998 |
| 30 | 44.327 | 44.458 | 1.0000 |

| Legend | |
|---|---|
| (green) | TP |
| (yellow) | TTP |
| (red) | FP |

| | TN | TTN | FN |
|---|---|---|---|
| VOC Label | 12, 25, 28 | - | - |

Supplementary Table 3.2.25: Detailed evaluation of the results of the CNN-based system with VGG-8-1D analysis (Stage 2) of the testing clinical sample Test-05-ES.

**Test_05_ES** (Sample ID 25)

| VOC Label | Start detection $s\mathcal{RT}$ | End detection $e\mathcal{RT}$ | Confidence $\mathcal{T}$ |
|---|---|---|---|
| 1 | 3.121 | 3.283 | 1.0000 |
| 2 | 3.357 | 3.474 | 1.0000 |
| 3 | 3.941 | 4.005 | 0.9999 |
| 4 | 4.007 | 4.119 | 1.0000 |
| 5 | 4.480 | 4.596 | 1.0000 |
| 6 | 4.599 | 4.779 | 1.0000 |
| 8 | 6.087 | 6.187 | 1.0000 |
| 9 | 6.190 | 6.285 | 1.0000 |
| 12 | 6.816 | 6.925 | 1.0000 |
| 13 | 7.341 | 7.410 | 0.9197 |
| 14 | 7.845 | 7.919 | 0.9998 |
| 15 | 9.046 | 9.155 | 1.0000 |
| 16 | 9.473 | 9.576 | 1.0000 |
| 17 | 11.313 | 11.421 | 1.0000 |
| 18 | 12.039 | 12.143 | 1.0000 |
| 19 | 12.493 | 12.593 | 1.0000 |
| 21 | 13.264 | 13.365 | 1.0000 |
| 20 | 13.381 | 13.468 | 1.0000 |
| 22 | 15.571 | 15.667 | 1.0000 |
| 23 | 18.362 | 18.445 | 1.0000 |
| 24 | 18.575 | 18.668 | 1.0000 |
| 25 | 19.076 | 19.190 | 1.0000 |
| 26 | 21.858 | 21.966 | 1.0000 |
| 27 | 23.835 | 23.920 | 1.0000 |
| 28 | 24.947 | 25.048 | 1.0000 |
| 29 | 29.788 | 29.910 | 1.0000 |
| 30 | 44.239 | 44.364 | 1.0000 |

| | |
|---|---|
| (green) | **TP** |
| (yellow) | **TTP** |
| (red) | **FP** |

| | TN | TTN | FN |
|---|---|---|---|
| **VOC Label** | 7, 10, 11 | - | - |

Supplementary Table 3.2.26: Detailed evaluation of the results of the CNN-based system with VGG-8-1D analysis (Stage 2) of the testing clinical sample Test-06-BS01.

**Test_06_BS01** (Sample ID 26)

| VOC Label | Start detection $s\mathcal{RT}$ | End detection $e\mathcal{RT}$ | Confidence $\mathcal{T}$ |
|---|---|---|---|
| 1 | 3.140 | 3.242 | 0.9999 |
| 2 | 3.386 | 3.468 | 0.9995 |
| 3 | 3.925 | 3.991 | 0.9999 |
| 4 | 3.994 | 4.071 | 0.9999 |
| 5 | 4.437 | 4.530 | 1.0000 |
| 6 | 4.679 | 4.791 | 0.9949 |
| 7 | 5.656 | 5.778 | 1.0000 |
| 8 | 5.997 | 6.072 | 1.0000 |
| 9 | 6.074 | 6.154 | 0.9999 |
| 10 | 6.328 | 6.424 | 1.0000 |
| 11 | 6.496 | 6.741 | 0.9988 |
| 12 | 7.062 | 7.120 | 0.9814 |
| 13 | 7.190 | 7.275 | 1.0000 |
| 14 | 7.679 | 7.775 | 1.0000 |
| 17 | 11.097 | 11.212 | 0.9996 |
| 18 | 11.837 | 11.904 | 0.9946 |
| 21 | 13.089 | 13.171 | 0.9997 |
| 20 | 13.174 | 13.249 | 1.0000 |
| 22 | 15.364 | 15.443 | 1.0000 |
| 23 | 18.133 | 18.210 | 1.0000 |
| 24 | 18.363 | 18.425 | 0.9946 |
| 25 | 19.030 | 19.104 | 0.9975 |
| 26 | 21.665 | 21.729 | 0.9595 |
| 27 | 23.600 | 23.677 | 1.0000 |
| 29 | 29.546 | 29.618 | 0.9659 |
| 30 | 43.939 | 44.056 | 1.0000 |

| | |
|---|---|
| | **TP** |
| | **TTP** |
| | **FP** |

| | TN | TTN | FN |
|---|---|---|---|
| **VOC Label** | 15, 16, 19, 28 | - | - |

Supplementary Table 3.2.27: Detailed evaluation of the results of the CNN-based system with VGG-8-1D analysis (Stage 2) of the testing clinical sample Test-06-BS02.

**Test_06_BS02** (Sample ID 27)

| VOC Label | Start detection $sRT$ | End detection $eRT$ | Confidence $T$ |
|---|---|---|---|
| 1 | 3.084 | 3.238 | 1.0000 |
| 2 | 3.305 | 3.432 | 1.0000 |
| 3 | 3.867 | 3.944 | 1.0000 |
| 4 | 3.947 | 4.037 | 1.0000 |
| 5 | 4.386 | 4.602 | 1.0000 |
| 6 | 4.634 | 4.704 | 0.9990 |
| 7 | 5.624 | 5.741 | 1.0000 |
| 8 | 5.962 | 6.047 | 1.0000 |
| 9 | 6.050 | 6.140 | 1.0000 |
| 10 | 6.298 | 6.407 | 1.0000 |
| 11 | 6.648 | 6.719 | 0.9998 |
| 12 | 7.034 | 7.108 | 0.9991 |
| 13 | 7.180 | 7.257 | 1.0000 |
| 14 | 7.669 | 7.759 | 1.0000 |
| 15 | 8.887 | 8.977 | 1.0000 |
| 16 | 9.306 | 9.372 | 0.9960 |
| 17 | 11.109 | 11.218 | 1.0000 |
| 18 | 11.831 | 11.923 | 1.0000 |
| 19 | 12.299 | 12.368 | 1.0000 |
| 21 | 13.082 | 13.174 | 1.0000 |
| 20 | 13.177 | 13.254 | 1.0000 |
| 22 | 15.366 | 15.443 | 1.0000 |
| 23 | 18.142 | 18.222 | 1.0000 |
| 24 | 18.367 | 18.431 | 0.9993 |
| 25 | 18.930 | 19.026 | 0.9999 |
| 26 | 21.675 | 21.741 | 0.9767 |
| 27 | 23.611 | 23.687 | 1.0000 |
| 29 | 29.551 | 29.625 | 0.9970 |
| 30 | 43.945 | 44.075 | 1.0000 |

| Colour | Legend |
|---|---|
| green | TP |
| yellow | TTP |
| red | FP |

| | TN | TTN | FN |
|---|---|---|---|
| VOC Label | 28 | 12 | - |

Supplementary Table 3.2.28: Detailed evaluation of the results of the CNN-based system with VGG-8-1D analysis (Stage 2) of the testing clinical sample Test-06-BS03.

**Test_06_BS03** (Sample ID 28)

| VOC Label | Start detection $sRT$ | End detection $eRT$ | Confidence $T$ |
|---|---|---|---|
| 1 | 3.085 | 3.237 | 1.0000 |
| 2 | 3.298 | 3.424 | 1.0000 |
| 3 | 3.866 | 3.941 | 1.0000 |
| 4 | 3.943 | 4.028 | 1.0000 |
| 5 | 4.383 | 4.599 | 1.0000 |
| 6 | 4.631 | 4.703 | 0.9978 |
| 7 | 5.621 | 5.733 | 1.0000 |
| 8 | 5.952 | 6.040 | 1.0000 |
| 9 | 6.043 | 6.136 | 1.0000 |
| 10 | 6.285 | 6.400 | 1.0000 |
| 11 | 6.627 | 6.702 | 0.9997 |
| 12 | 6.705 | 6.782 | 1.0000 |
| 13 | 7.164 | 7.244 | 1.0000 |
| 14 | 7.655 | 7.743 | 1.0000 |
| 15 | 8.882 | 8.978 | 1.0000 |
| 16 | 9.305 | 9.371 | 0.9859 |
| 17 | 11.112 | 11.221 | 1.0000 |
| 18 | 11.834 | 11.919 | 1.0000 |
| 19 | 12.292 | 12.372 | 1.0000 |
| 21 | 13.080 | 13.165 | 1.0000 |
| 20 | 13.167 | 13.252 | 1.0000 |
| 22 | 15.364 | 15.441 | 1.0000 |
| 23 | 18.140 | 18.214 | 1.0000 |
| 24 | 18.357 | 18.423 | 1.0000 |
| 26 | 21.672 | 21.736 | 0.9743 |
| 27 | 23.615 | 23.676 | 0.9971 |
| 29 | 29.550 | 29.624 | 0.9974 |
| 30 | 43.944 | 44.069 | 1.0000 |

| | |
|---|---|
| (green) | **TP** |
| (yellow) | **TTP** |
| (red) | **FP** |

| | TN | TTN | FN |
|---|---|---|---|
| **VOC Label** | 25, 28 | - | - |

Supplementary Table 3.2.29: Detailed evaluation of the results of the CNN-based system with VGG-8-1D analysis (Stage 2) of the testing clinical sample Test-06-BS04.

**Test_06_BS04** (Sample ID 29)

| VOC Label | Start detection $s\mathcal{RT}$ | End detection $e\mathcal{RT}$ | Confidence $\mathcal{T}$ |
|---|---|---|---|
| 1 | 3.084 | 3.236 | 1.0000 |
| 2 | 3.300 | 3.433 | 1.0000 |
| 3 | 3.865 | 3.945 | 1.0000 |
| 4 | 3.948 | 4.030 | 1.0000 |
| 5 | 4.382 | 4.601 | 1.0000 |
| 6 | 4.633 | 4.697 | 0.9976 |
| 7 | 5.625 | 5.743 | 1.0000 |
| 8 | 5.953 | 6.047 | 1.0000 |
| 9 | 6.049 | 6.143 | 1.0000 |
| 10 | 6.292 | 6.402 | 1.0000 |
| 11 | 6.479 | 6.534 | 0.9930 |
| 12 | 7.035 | 7.109 | 0.9991 |
| 13 | 7.178 | 7.255 | 1.0000 |
| 14 | 7.670 | 7.758 | 1.0000 |
| 15 | 8.886 | 8.976 | 1.0000 |
| 17 | 11.117 | 11.220 | 1.0000 |
| 18 | 11.833 | 11.931 | 1.0000 |
| 19 | 12.302 | 12.373 | 0.9999 |
| 21 | 13.082 | 13.172 | 1.0000 |
| 20 | 13.174 | 13.259 | 1.0000 |
| 22 | 15.366 | 15.448 | 1.0000 |
| 23 | 18.142 | 18.222 | 1.0000 |
| 24 | 18.370 | 18.423 | 0.9662 |
| 26 | 21.678 | 21.741 | 0.9768 |
| 27 | 23.616 | 23.688 | 1.0000 |
| 29 | 29.546 | 29.625 | 0.9747 |
| 30 | 43.952 | 44.076 | 1.0000 |

| Colour | Legend |
|---|---|
| (green) | TP |
| (yellow) | TTP |
| (red) | FP |

| | TN | TTN | FN |
|---|---|---|---|
| VOC Label | 16, 25, 28 | 11 | - |

Supplementary Table 3.2.30: Detailed evaluation of the results of the CNN-based system with VGG-8-1D analysis (Stage 2) of the testing clinical sample Test-06-ES.

**Test_06_ES** (Sample ID 30)

| VOC Label | Start detection $sRT$ | End detection $eRT$ | Confidence $\mathcal{T}$ |
|---|---|---|---|
| 1 | 3.163 | 3.242 | 0.9999 |
| 3 | 3.882 | 3.938 | 0.9968 |
| 4 | 3.940 | 4.041 | 1.0000 |
| 5 | 4.398 | 4.509 | 1.0000 |
| 8 | 5.971 | 6.055 | 1.0000 |
| 9 | 6.058 | 6.140 | 1.0000 |
| 11 | 6.486 | 6.545 | 0.9931 |
| 12 | 7.044 | 7.110 | 0.9981 |
| 13 | 7.187 | 7.256 | 0.9894 |
| 14 | 7.689 | 7.758 | 1.0000 |
| 15 | 8.879 | 8.963 | 1.0000 |
| 16 | 9.304 | 9.365 | 0.9837 |
| 17 | 11.109 | 11.209 | 1.0000 |
| 18 | 11.828 | 11.923 | 1.0000 |
| 19 | 12.291 | 12.376 | 1.0000 |
| 21 | 13.068 | 13.174 | 1.0000 |
| 20 | 13.179 | 13.240 | 0.9968 |
| 22 | 15.350 | 15.446 | 1.0000 |
| 23 | 18.142 | 18.219 | 1.0000 |
| 24 | 18.351 | 18.433 | 1.0000 |
| 25 | 18.862 | 18.955 | 1.0000 |
| 26 | 21.680 | 21.747 | 0.9903 |
| 27 | 23.613 | 23.682 | 0.9999 |
| 28 | 24.704 | 24.778 | 0.9999 |
| 29 | 29.529 | 29.630 | 1.0000 |
| 30 | 43.953 | 44.065 | 1.0000 |

| | |
|---|---|
| (green) | TP |
| (yellow) | TTP |
| (red) | FP |

| | TN | TTN | FN |
|---|---|---|---|
| **VOC Label** | 2, 6, 7, 10 | - | - |

Supplementary Table 3.2.31: Detailed evaluation of the results of the CNN-based system with VGG-8-1D analysis (Stage 2) of the testing clinical sample Test-07-BS01.

**Test_07_BS01** (Sample ID 31)

| VOC Label | Start detection $sRT$ | End detection $eRT$ | Confidence $T$ |
|---|---|---|---|
| 1 | 3.075 | 3.211 | 1.0000 |
| 2 | 3.283 | 3.445 | 1.0000 |
| 3 | 3.803 | 3.901 | 1.0000 |
| 4 | 3.904 | 3.989 | 1.0000 |
| 5 | 4.312 | 4.416 | 1.0000 |
| 6 | 4.558 | 4.624 | 0.9989 |
| 7 | 5.513 | 5.609 | 0.9943 |
| 8 | 5.825 | 5.912 | 1.0000 |
| 9 | 5.915 | 6.005 | 1.0000 |
| 10 | 6.173 | 6.258 | 1.0000 |
| 11 | 6.260 | 6.430 | 1.0000 |
| 12 | 6.571 | 6.627 | 0.9778 |
| 13 | 7.012 | 7.091 | 1.0000 |
| 14 | 7.489 | 7.585 | 1.0000 |
| 15 | 8.675 | 8.769 | 1.0000 |
| 16 | 9.094 | 9.158 | 0.9159 |
| 17 | 10.861 | 10.970 | 1.0000 |
| 18 | 11.574 | 11.683 | 1.0000 |
| 19 | 12.041 | 12.131 | 1.0000 |
| 21 | 12.821 | 12.919 | 1.0000 |
| 20 | 12.921 | 12.990 | 1.0000 |
| 22 | 15.087 | 15.178 | 1.0000 |
| 23 | 17.875 | 17.949 | 1.0000 |
| 24 | 18.074 | 18.159 | 1.0000 |
| 26 | 21.421 | 21.485 | 0.9711 |
| 27 | 23.328 | 23.408 | 1.0000 |
| 29 | 29.190 | 29.312 | 1.0000 |
| 30 | 43.589 | 43.709 | 1.0000 |

| Colour | Category |
|---|---|
| (green) | TP |
| (yellow) | TTP |
| (red) | FP |

| | TN | TTN | FN |
|---|---|---|---|
| VOC Label | 25, 28 | - | - |

Supplementary Table 3.2.32: Detailed evaluation of the results of the CNN-based system with VGG-8-1D analysis (Stage 2) of the testing clinical sample Test-07-BS02.

**Test_07_BS02** (Sample ID 32)

| VOC Label | Start detection $s\mathcal{RT}$ | End detection $e\mathcal{RT}$ | Confidence $\mathcal{T}$ |
|---|---|---|---|
| 1 | 3.083 | 3.227 | 1.0000 |
| 2 | 3.291 | 3.448 | 1.0000 |
| 3 | 3.811 | 3.907 | 1.0000 |
| 4 | 3.909 | 3.997 | 1.0000 |
| 5 | 4.320 | 4.534 | 1.0000 |
| 6 | 4.566 | 4.622 | 0.9804 |
| 7 | 5.535 | 5.623 | 0.7864 |
| 8 | 5.834 | 5.922 | 1.0000 |
| 9 | 5.924 | 6.013 | 1.0000 |
| 10 | 6.173 | 6.282 | 1.0000 |
| 11 | 6.340 | 6.401 | 0.9814 |
| 12 | 6.590 | 6.646 | 0.9430 |
| 13 | 7.023 | 7.105 | 1.0000 |
| 14 | 7.504 | 7.597 | 1.0000 |
| 15 | 8.690 | 8.789 | 1.0000 |
| 16 | 9.103 | 9.191 | 0.9943 |
| 17 | 10.882 | 10.991 | 1.0000 |
| 18 | 11.595 | 11.707 | 1.0000 |
| 19 | 12.057 | 12.150 | 1.0000 |
| 21 | 12.837 | 12.938 | 1.0000 |
| 20 | 12.940 | 13.012 | 1.0000 |
| 22 | 15.107 | 15.200 | 1.0000 |
| 23 | 17.893 | 17.972 | 1.0000 |
| 24 | 18.089 | 18.179 | 1.0000 |
| 25 | 18.697 | 18.747 | 0.8669 |
| 26 | 21.440 | 21.504 | 0.9678 |
| 27 | 23.345 | 23.428 | 1.0000 |
| 29 | 29.215 | 29.330 | 1.0000 |
| 30 | 43.615 | 43.724 | 1.0000 |

| | |
|---|---|
| | **TP** |
| | **TTP** |
| | **FP** |

| | TN | TTN | FN |
|---|---|---|---|
| **VOC Label** | 28 | - | - |

Supplementary Table 3.2.33: Detailed evaluation of the results of the CNN-based system with VGG-8-1D analysis (Stage 2) of the testing clinical sample Test-07-BS03.

**Test_07_BS03** (Sample ID 33)

| VOC Label | Start detection $sRT$ | End detection $eRT$ | Confidence $T$ |
|---|---|---|---|
| 1 | 3.096 | 3.234 | 1.0000 |
| 2 | 3.301 | 3.441 | 1.0000 |
| 3 | 3.834 | 3.927 | 1.0000 |
| 4 | 3.930 | 4.015 | 1.0000 |
| 5 | 4.333 | 4.550 | 1.0000 |
| 6 | 4.553 | 4.633 | 0.9933 |
| 7 | 5.521 | 5.635 | 1.0000 |
| 8 | 5.845 | 5.935 | 1.0000 |
| 9 | 5.938 | 6.028 | 1.0000 |
| 10 | 6.171 | 6.283 | 1.0000 |
| 11 | 6.330 | 6.423 | 0.9995 |
| 12 | 6.540 | 6.635 | 0.9233 |
| 13 | 7.041 | 7.116 | 1.0000 |
| 14 | 7.516 | 7.606 | 1.0000 |
| 15 | 8.670 | 8.779 | 1.0000 |
| 16 | 9.091 | 9.187 | 1.0000 |
| 17 | 10.873 | 10.982 | 1.0000 |
| 18 | 11.581 | 11.706 | 1.0000 |
| 19 | 12.061 | 12.141 | 1.0000 |
| 21 | 12.830 | 12.931 | 1.0000 |
| 20 | 12.934 | 13.019 | 1.0000 |
| 22 | 15.111 | 15.188 | 1.0000 |
| 23 | 17.890 | 17.969 | 1.0000 |
| 24 | 18.108 | 18.169 | 0.9987 |
| 25 | 18.588 | 18.670 | 0.9997 |
| 26 | 21.276 | 21.345 | 0.9883 |
| 27 | 23.345 | 23.424 | 1.0000 |
| 29 | 29.214 | 29.322 | 1.0000 |
| 30 | 43.599 | 43.732 | 1.0000 |

| Colour | Legend |
|---|---|
| (green) | TP |
| (yellow) | TTP |
| (red) | FP |

| | TN | TTN | FN |
|---|---|---|---|
| VOC Label | 28 | 11 | - |

Supplementary Table 3.2.34: Detailed evaluation of the results of the CNN-based system with VGG-8-1D analysis (Stage 2) of the testing clinical sample Test-07-BS04.

**Test_07_BS04** (Sample ID 34)

| VOC Label | Start detection $sRT$ | End detection $eRT$ | Confidence $T$ |
|---|---|---|---|
| 1 | 3.111 | 3.233 | 1.0000 |
| 2 | 3.300 | 3.443 | 1.0000 |
| 3 | 3.833 | 3.921 | 1.0000 |
| 4 | 3.924 | 4.003 | 1.0000 |
| 5 | 4.332 | 4.550 | 1.0000 |
| 6 | 4.571 | 4.632 | 0.9834 |
| 7 | 5.521 | 5.632 | 1.0000 |
| 8 | 5.844 | 5.935 | 1.0000 |
| 9 | 5.937 | 6.025 | 1.0000 |
| 10 | 6.171 | 6.282 | 1.0000 |
| 11 | 6.325 | 6.417 | 0.9962 |
| 12 | 6.550 | 6.635 | 0.9711 |
| 13 | 7.041 | 7.115 | 1.0000 |
| 14 | 7.516 | 7.603 | 1.0000 |
| 15 | 8.675 | 8.781 | 1.0000 |
| 16 | 9.091 | 9.192 | 1.0000 |
| 17 | 10.876 | 10.984 | 1.0000 |
| 18 | 11.583 | 11.708 | 1.0000 |
| 19 | 12.061 | 12.143 | 1.0000 |
| 21 | 12.833 | 12.933 | 1.0000 |
| 20 | 12.936 | 13.018 | 1.0000 |
| 22 | 15.111 | 15.190 | 1.0000 |
| 23 | 17.892 | 17.974 | 1.0000 |
| 24 | 18.096 | 18.176 | 1.0000 |
| 25 | 18.584 | 18.675 | 1.0000 |
| 26 | 21.438 | 21.504 | 0.9657 |
| 27 | 23.347 | 23.432 | 1.0000 |
| 28 | 24.411 | 24.486 | 0.9964 |
| 29 | 29.211 | 29.336 | 1.0000 |
| 30 | 43.634 | 43.744 | 1.0000 |

| Colour | Legend |
|---|---|
| (green) | TP |
| (yellow) | TTP |
| (red) | FP |

| | TN | TTN | FN |
|---|---|---|---|
| VOC Label | - | 26 | - |

Supplementary Table 3.2.35: Detailed evaluation of the results of the CNN-based system with VGG-8-1D analysis (Stage 2) of the testing clinical sample Test-07-ES.

**Test_07_ES** (Sample ID 35)

| VOC Label | Start detection $s\mathcal{RT}$ | End detection $e\mathcal{RT}$ | Confidence $\mathcal{T}$ |
|---|---|---|---|
| 1 | 3.095 | 3.241 | 1.0000 |
| 2 | 3.315 | 3.422 | 1.0000 |
| 3 | 3.838 | 3.899 | 1.0000 |
| 4 | 3.902 | 4.005 | 1.0000 |
| 5 | 4.334 | 4.451 | 1.0000 |
| 6 | 4.517 | 4.639 | 1.0000 |
| 8 | 5.841 | 5.934 | 1.0000 |
| 9 | 5.936 | 6.026 | 1.0000 |
| 10 | 6.201 | 6.265 | 0.9956 |
| 12 | 6.528 | 6.636 | 1.0000 |
| 13 | 7.037 | 7.111 | 0.9996 |
| 14 | 7.517 | 7.604 | 1.0000 |
| 15 | 8.675 | 8.779 | 1.0000 |
| 16 | 9.089 | 9.190 | 1.0000 |
| 17 | 10.870 | 10.979 | 1.0000 |
| 18 | 11.586 | 11.692 | 1.0000 |
| 19 | 12.053 | 12.143 | 1.0000 |
| 21 | 12.827 | 12.925 | 1.0000 |
| 20 | 12.928 | 13.018 | 1.0000 |
| 22 | 15.099 | 15.192 | 1.0000 |
| 23 | 17.890 | 17.970 | 1.0000 |
| 24 | 18.084 | 18.177 | 1.0000 |
| 25 | 18.567 | 18.679 | 1.0000 |
| 26 | 21.282 | 21.388 | 1.0000 |
| 27 | 23.345 | 23.427 | 1.0000 |
| 29 | 29.218 | 29.332 | 1.0000 |
| 30 | 43.613 | 43.722 | 1.0000 |

| Colour | Key |
|---|---|
| (green) | TP |
| (yellow) | TTP |
| (red) | FP |

| | TN | TTN | FN |
|---|---|---|---|
| VOC Label | 7, 11, 28 | - | - |

Supplementary Table 3.2.36: Detailed evaluation of the results of the CNN-based system with VGG-8-1D analysis (Stage 2) of the testing clinical sample Test-08-BS01.

**Test_08_BS01** (Sample ID 36)

| VOC Label | Start detection $sRT$ | End detection $eRT$ | Confidence $\mathcal{T}$ |
|---|---|---|---|
| 1 | 3.071 | 3.202 | 1.0000 |
| 2 | 3.266 | 3.399 | 1.0000 |
| 3 | 3.754 | 3.839 | 1.0000 |
| 4 | 3.842 | 3.927 | 1.0000 |
| 5 | 4.226 | 4.439 | 1.0000 |
| 6 | 4.471 | 4.543 | 0.9946 |
| 7 | 5.356 | 5.478 | 1.0000 |
| 8 | 5.677 | 5.760 | 1.0000 |
| 9 | 5.762 | 5.858 | 1.0000 |
| 10 | 5.983 | 6.100 | 1.0000 |
| 11 | 6.158 | 6.291 | 1.0000 |
| 13 | 6.828 | 6.910 | 1.0000 |
| 14 | 7.292 | 7.388 | 1.0000 |
| 15 | 8.434 | 8.538 | 1.0000 |
| 16 | 8.841 | 8.923 | 0.9987 |
| 17 | 10.580 | 10.689 | 1.0000 |
| 18 | 11.283 | 11.406 | 1.0000 |
| 19 | 11.761 | 11.844 | 1.0000 |
| 21 | 12.531 | 12.629 | 1.0000 |
| 20 | 12.632 | 12.709 | 1.0000 |
| 22 | 14.787 | 14.877 | 1.0000 |
| 23 | 17.568 | 17.651 | 1.0000 |
| 24 | 17.754 | 17.850 | 1.0000 |
| 27 | 23.010 | 23.095 | 1.0000 |
| 29 | 28.828 | 28.943 | 1.0000 |
| 30 | 43.197 | 43.314 | 1.0000 |

| Colour | |
|---|---|
| (green) | **TP** |
| (yellow) | **TTP** |
| (red) | **FP** |

| | TN | TTN | FN |
|---|---|---|---|
| **VOC Label** | 12, 25, 26, 28 | 11 | - |

Supplementary Table 3.2.37: Detailed evaluation of the results of the CNN-based system with VGG-8-1D analysis (Stage 2) of the testing clinical sample Test-08-BS02.

**Test_08_BS02** (Sample ID 37)

| VOC Label | Start detection $\mathscr{sRT}$ | End detection $\mathscr{eRT}$ | Confidence $\mathscr{T}$ |
|---|---|---|---|
| 1 | 3.063 | 3.210 | 1.0000 |
| 2 | 3.266 | 3.413 | 1.0000 |
| 3 | 3.751 | 3.842 | 1.0000 |
| 4 | 3.845 | 3.930 | 1.0000 |
| 5 | 4.234 | 4.447 | 1.0000 |
| 6 | 4.474 | 4.535 | 0.9914 |
| 7 | 5.370 | 5.468 | 1.0000 |
| 8 | 5.681 | 5.766 | 1.0000 |
| 9 | 5.768 | 5.861 | 1.0000 |
| 10 | 5.986 | 6.108 | 1.0000 |
| 11 | 6.148 | 6.267 | 1.0000 |
| 13 | 6.833 | 6.915 | 1.0000 |
| 14 | 7.295 | 7.393 | 1.0000 |
| 15 | 8.434 | 8.540 | 1.0000 |
| 16 | 8.843 | 8.939 | 1.0000 |
| 17 | 10.581 | 10.690 | 1.0000 |
| 18 | 11.287 | 11.409 | 1.0000 |
| 19 | 11.763 | 11.848 | 1.0000 |
| 21 | 12.535 | 12.633 | 1.0000 |
| 20 | 12.636 | 12.715 | 1.0000 |
| 22 | 14.788 | 14.881 | 1.0000 |
| 23 | 17.576 | 17.655 | 1.0000 |
| 24 | 17.759 | 17.852 | 1.0000 |
| 26 | 21.142 | 21.192 | 0.7765 |
| 27 | 23.014 | 23.099 | 1.0000 |
| 28 | 24.053 | 24.135 | 0.9972 |
| 29 | 28.823 | 28.951 | 1.0000 |
| 30 | 43.206 | 43.312 | 1.0000 |

| | |
|---|---|
| | **TP** |
| | **TTP** |
| | **FP** |

| | TN | TTN | FN |
|---|---|---|---|
| **VOC Label** | 12, 25 | 11 | - |

Supplementary Table 3.2.38: Detailed evaluation of the results of the CNN-based system with VGG-8-1D analysis (Stage 2) of the testing clinical sample Test-08-ES.

**Test_08_ES** (Sample ID 38)

| VOC Label | Start detection $sRT$ | End detection $eRT$ | Confidence $T$ |
|---|---|---|---|
| 1 | 3.086 | 3.210 | 1.0000 |
| 2 | 3.287 | 3.386 | 0.9998 |
| 3 | 3.770 | 3.826 | 0.9951 |
| 4 | 3.829 | 3.946 | 1.0000 |
| 5 | 4.237 | 4.354 | 1.0000 |
| 6 | 4.357 | 4.521 | 1.0000 |
| 8 | 5.673 | 5.768 | 1.0000 |
| 9 | 5.771 | 5.861 | 1.0000 |
| 12 | 6.341 | 6.450 | 1.0000 |
| 13 | 6.837 | 6.912 | 0.9994 |
| 14 | 7.302 | 7.387 | 1.0000 |
| 15 | 8.429 | 8.533 | 1.0000 |
| 16 | 8.838 | 8.936 | 1.0000 |
| 17 | 10.577 | 10.689 | 1.0000 |
| 18 | 11.288 | 11.397 | 1.0000 |
| 19 | 11.758 | 11.845 | 1.0000 |
| 21 | 12.530 | 12.620 | 1.0000 |
| 20 | 12.622 | 12.705 | 0.9998 |
| 22 | 14.782 | 14.877 | 1.0000 |
| 23 | 17.573 | 17.653 | 1.0000 |
| 24 | 17.757 | 17.850 | 1.0000 |
| 25 | 18.226 | 18.338 | 1.0000 |
| 26 | 20.921 | 21.038 | 1.0000 |
| 27 | 23.013 | 23.098 | 1.0000 |
| 29 | 28.823 | 28.945 | 1.0000 |
| 30 | 43.214 | 43.301 | 0.9963 |

| | |
|---|---|
| (green) | **TP** |
| (yellow) | **TTP** |
| (red) | **FP** |

| | TN | TTN | FN |
|---|---|---|---|
| **VOC Label** | 7, 10, 11, 28 | - | - |

# 4 DenseNet-40-1D model – Results

Supplementary Table 4.1: Results of the testing clinical sample analysis with the CNN-based system with DenseNet-40-1D model. Results evaluated per each target VOC.

<u>*Label*</u> - the class label of VOC. <u>*TP*</u> - number of true positives detected per VOC. <u>*TTP*</u> - number of tentative true positives detected per VOC. <u>*FP*</u> - number of false positives detected per VOC. <u>*TTN*</u> - number of tentative true negatives detected per VOC. <u>*FN*</u> - number of false negatives detected per VOC. <u>*TN*</u> - number of true negatives detected per VOC (evaluation excluding *RT* position). <u>*FP**</u> - number of false positives detected per VOC (evaluation excluding *RT* position). <u>*TTP**</u> - number of tentative true positives detected per VOC (evaluation excluding *RT* position). <u>*Sensitivity (expert)*</u> - Sensitivity per VOC in relation to expert-derived ground truth benchmark; tentative true positives (TTP) are considered FP, tentative true negatives (TTN) are considered FN; sensitivity = TP/(TP+FN+TTN). <u>*Sensitivity (system)*</u> - Sensitivity per VOC in relation to system-derived correction benchmark; tentative true positives (TTP) are considered TP, tentative true negatives (TTN) are considered TN; sensitivity=(TP+TTP)/(TP+TTP+FN). <u>*Specificity (expert)*</u> - Specificity per VOC in relation to expert-derived ground truth benchmark; tentative true positives (TTP*) are considered FP*; specificity=TN/TN+FP*+TTP*. <u>*Specificity (system)*</u> - Specificity per VOC in relation to system-derived correction benchmark; tentative true positives (TTP*) are considered TP; specificity=TN/TN+FP*. <u>*AP (expert)*</u> - Average precision per VOC in relation to expert-derived ground truth benchmark. <u>*AP (system)*</u> - Average precision per VOC in relation to system-derived correction benchmark.

| Label | TP | TTP | FP | TTN | FN | TN | FP* | TTP* | Sensitivity (expert) | Sensitivity (system) | Specificity (expert) | Specificity (system) | AP (expert) | AP (system) |
|---|---|---|---|---|---|---|---|---|---|---|---|---|---|---|
| 1 | 20 | 18 | 0 | 0 | 0 | 0 | 0 | 18 | 1 | 1 | 0 | - | 0.6969 | 1 |
| 2 | 29 | 6 | 0 | 0 | 0 | 3 | 0 | 6 | 1 | 1 | 0.3333 | 1 | 0.9185 | 1 |
| 3 | 30 | 6 | 1 | 0 | 0 | 1 | 1 | 6 | 1 | 1 | 0.125 | 0.5 | 0.9925 | 0.9985 |
| 4 | 36 | 2 | 0 | 2 | 0 | 0 | 0 | 0 | 0.9474 | 1 | - | - | 0.9955 | 1 |
| 5 | 35 | 3 | 0 | 1 | 0 | 0 | 0 | 2 | 0.9722 | 1 | 0 | - | 0.9323 | 1 |
| 6 | 10 | 27 | 0 | 1 | 0 | 1 | 0 | 26 | 0.9091 | 1 | 0.037 | 1 | 0.7453 | 1 |
| 7 | 23 | 7 | 0 | 0 | 0 | 8 | 0 | 7 | 1 | 1 | 0.5333 | 1 | 0.9852 | 1 |
| 8 | 37 | 1 | 0 | 0 | 0 | 0 | 0 | 1 | 1 | 1 | 0 | - | 0.9744 | 1 |
| 9 | 38 | 0 | 0 | 0 | 0 | 0 | 0 | 0 | 1 | 1 | - | - | 1 | 1 |
| 10 | 30 | 7 | 0 | 0 | 0 | 1 | 0 | 7 | 1 | 1 | 0.125 | 1 | 0.9870 | 1 |
| 11 | 18 | 15 | 0 | 1 | 0 | 5 | 0 | 14 | 0.9474 | 1 | 0.2632 | 1 | 0.6717 | 1 |
| 12 | 22 | 11 | 0 | 1 | 2 | 3 | 0 | 10 | 0.88 | 0.9429 | 0.2308 | 1 | 0.9140 | 1 |
| 13 | 32 | 5 | 0 | 1 | 0 | 1 | 0 | 4 | 0.9697 | 1 | 0.2 | 1 | 0.9644 | 1 |
| 14 | 29 | 1 | 0 | 0 | 4 | 4 | 0 | 1 | 0.8788 | 0.8824 | 0.8 | 1 | 0.9989 | 1 |
| 15 | 17 | 10 | 0 | 1 | 5 | 7 | 0 | 9 | 0.7391 | 0.8438 | 0.4375 | 1 | 0.8225 | 1 |
| 16 | 19 | 3 | 4 | 1 | 3 | 10 | 3 | 2 | 0.8261 | 0.88 | 0.6667 | 0.7692 | 0.9839 | 0.9838 |
| 17 | 38 | 0 | 0 | 0 | 0 | 0 | 0 | 0 | 1 | 1 | - | - | 1 | 1 |
| 18 | 35 | 2 | 0 | 0 | 1 | 0 | 0 | 2 | 0.9722 | 0.9737 | 0 | - | 0.9490 | 1 |
| 19 | 26 | 5 | 0 | 0 | 0 | 7 | 0 | 5 | 1 | 1 | 0.5833 | 1 | 0.9143 | 1 |
| 20 | 35 | 0 | 0 | 0 | 2 | 1 | 0 | 0 | 0.9459 | 0.9459 | 1 | 1 | 1 | 1 |
| 21 | 20 | 17 | 0 | 6 | 1 | 0 | 0 | 11 | 0.7407 | 0.9737 | 0 | - | 0.9696 | 1 |
| 22 | 32 | 5 | 0 | 0 | 0 | 1 | 0 | 5 | 1 | 1 | 0.1667 | 1 | 0.9044 | 1 |
| 23 | 36 | 0 | 0 | 0 | 0 | 2 | 0 | 0 | 1 | 1 | 1 | 1 | 1 | 1 |
| 24 | 23 | 7 | 1 | 0 | 1 | 7 | 0 | 7 | 0.9583 | 0.9677 | 0.5 | 1 | 0.8926 | 1 |
| 25 | 7 | 4 | 0 | 0 | 0 | 26 | 0 | 4 | 1 | 1 | 0.8667 | 1 | 0.9107 | 1 |
| 26 | 21 | 8 | 0 | 0 | 1 | 8 | 0 | 8 | 0.9545 | 0.9667 | 0.5 | 1 | 0.9762 | 1 |
| 27 | 32 | 2 | 0 | 0 | 0 | 4 | 0 | 2 | 1 | 1 | 0.6667 | 1 | 0.9982 | 1 |
| 28 | 16 | 5 | 0 | 0 | 1 | 16 | 0 | 5 | 0.9412 | 0.9545 | 0.7619 | 1 | 0.8520 | 1 |
| 29 | 31 | 2 | 0 | 0 | 0 | 5 | 0 | 2 | 1 | 1 | 0.7143 | 1 | 0.9529 | 1 |
| 30 | 31 | 2 | 0 | 0 | 1 | 4 | 0 | 2 | 0.9688 | 0.9706 | 0.6667 | 1 | 0.9960 | 1 |
| **TOTAL** | **808** | **181** | **6** | **15** | **22** | **125** | **4** | **166** | **0.9562** | **0.9782** | **0.4237** | **0.969** | **mAP** | |
| | | | | | | | | | | | | | **0.93** | **0.9994** |

Supplementary Figures 4.1-4.8: Precision against recall graphs for VOCs 1-8.

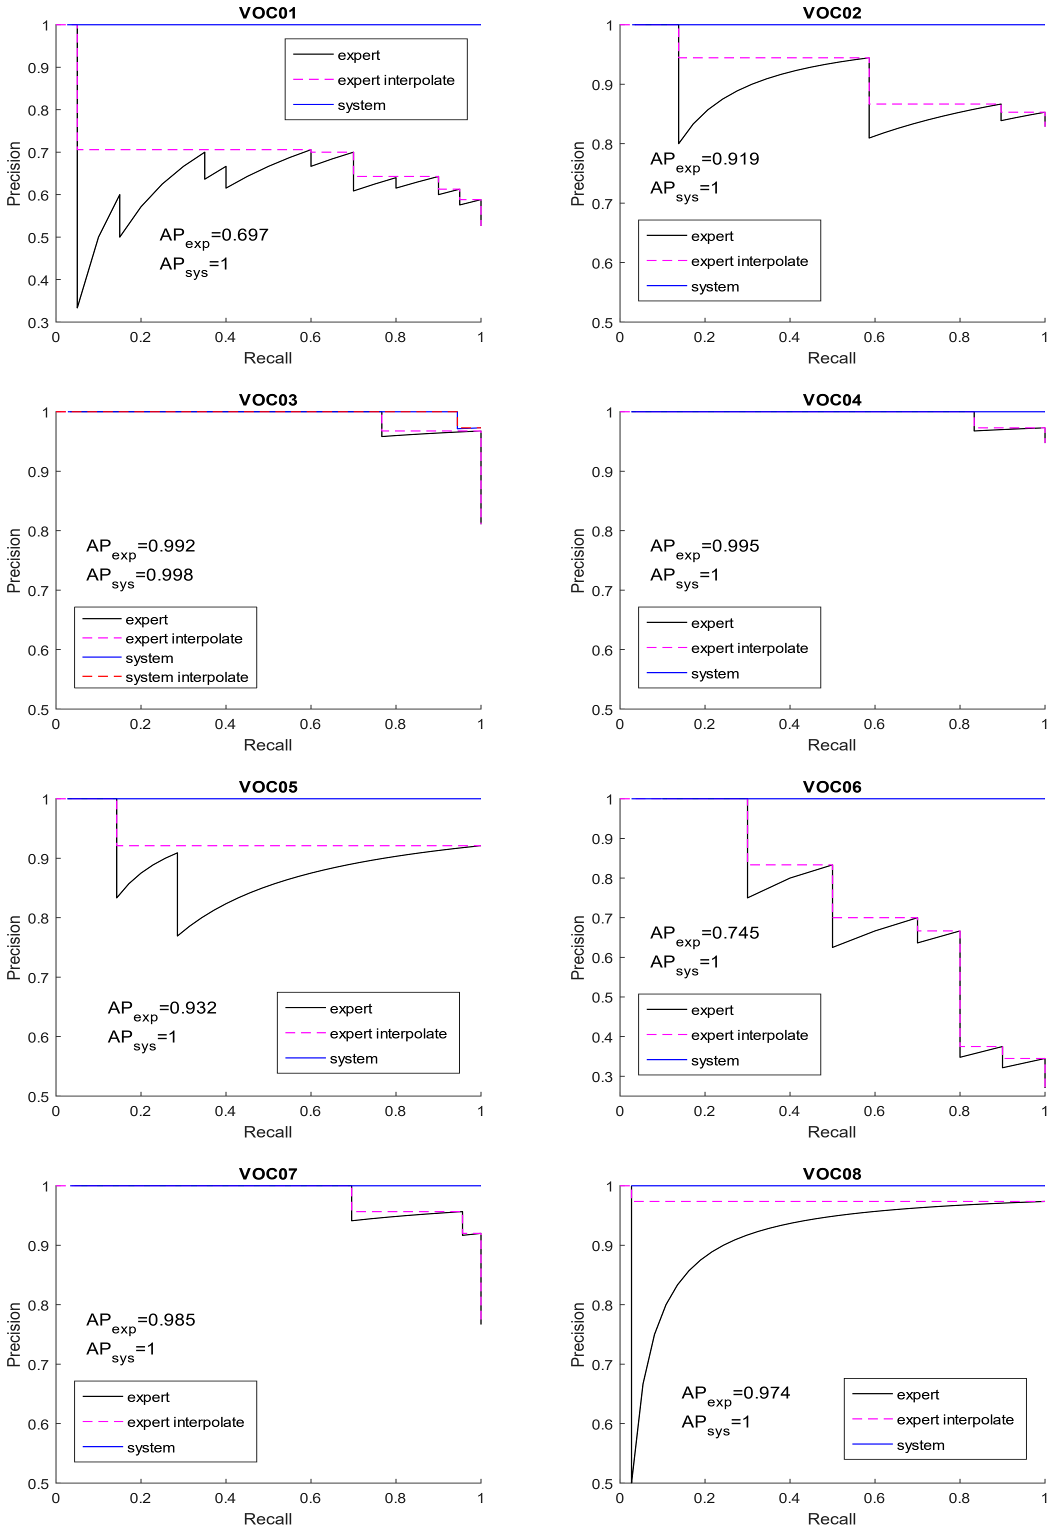

Supplementary Figures 4.9-4.16: Precision against recall graphs for VOCs 9-16.

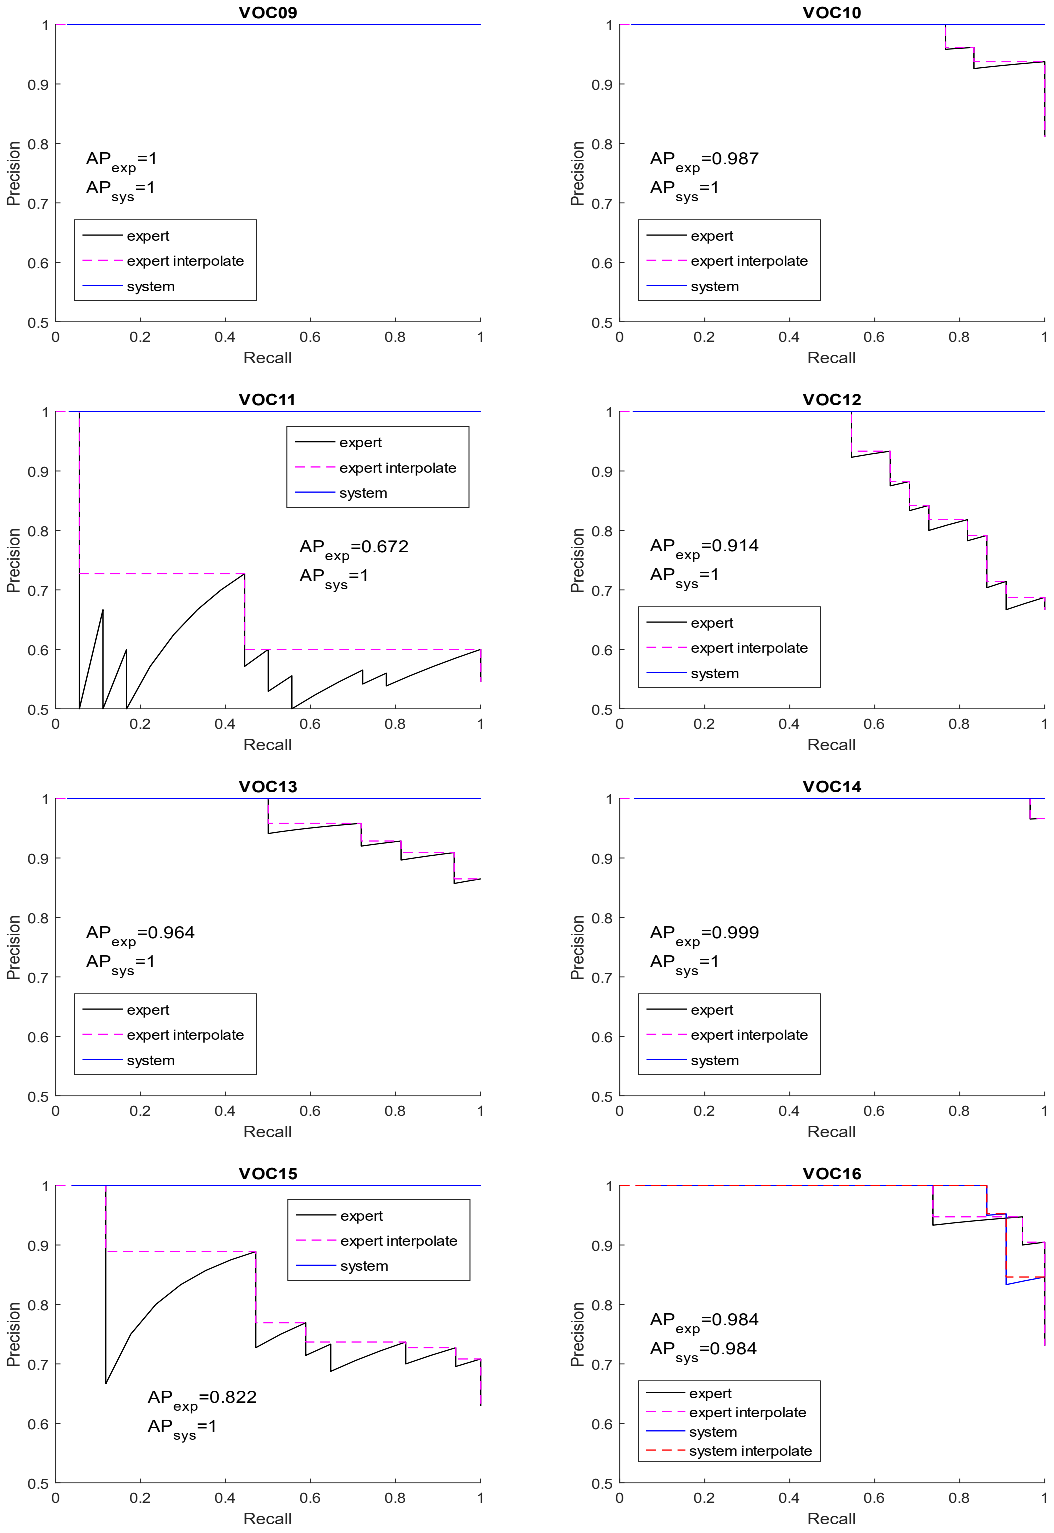

Supplementary Figures 4.17-4.24: Precision against recall graphs for VOCs 17-24.

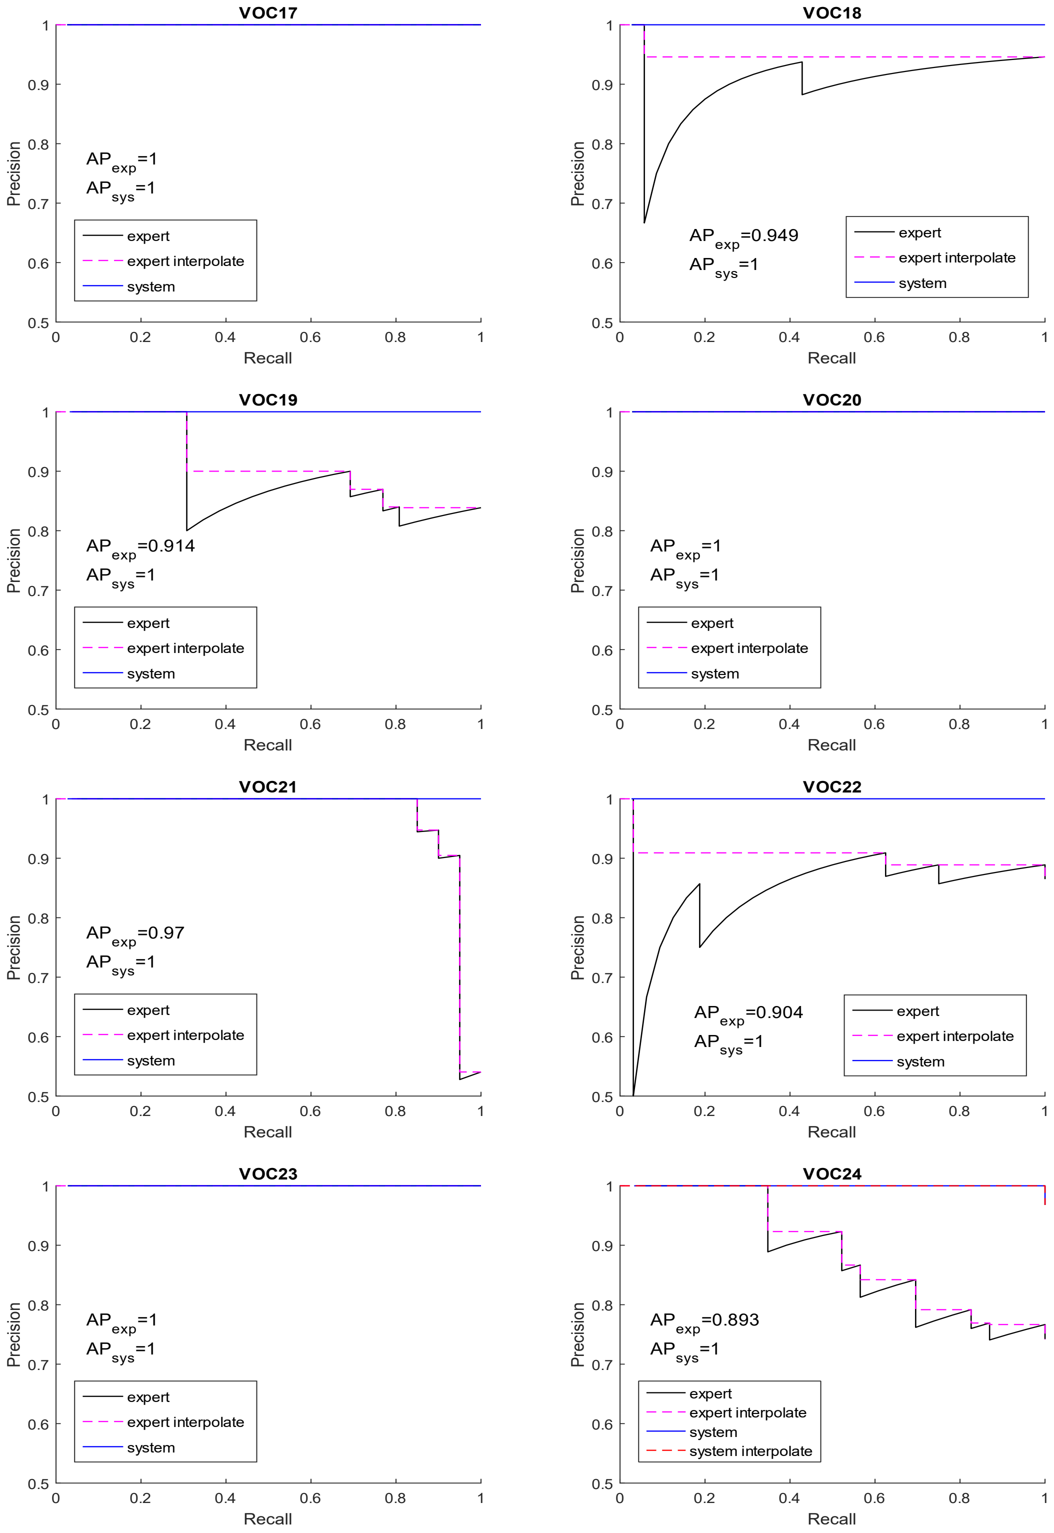

Supplementary Figures 4.25-4.30: Precision against recall graphs for VOCs 25-30.

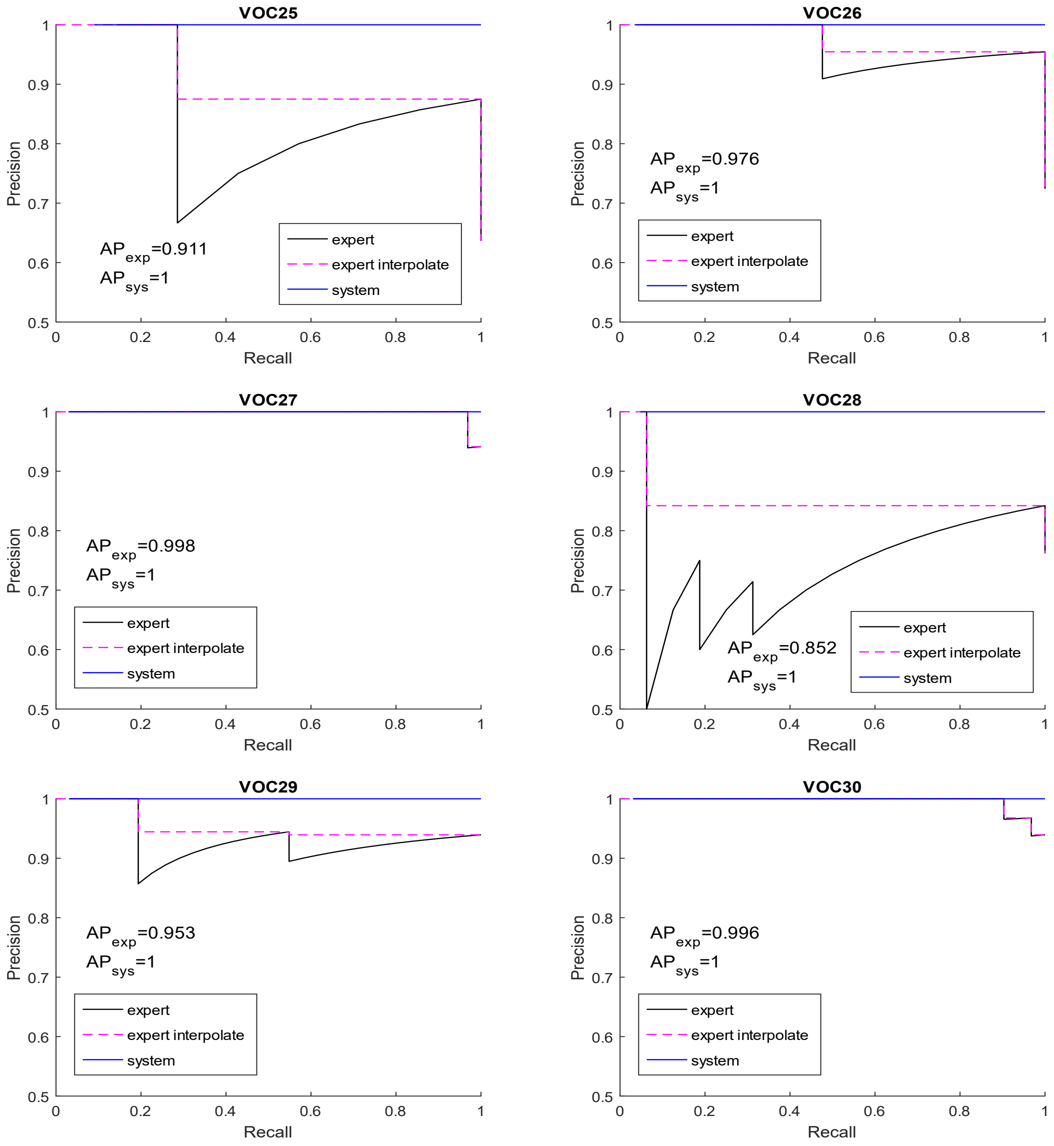

Supplementary Table 4.2: Results of the testing clinical sample analysis with the CNN-based system with DenseNet-40-1D model. Results evaluated per each testing sample.

*Sample ID* - number of a sample. *TP* - number of true positives detected per sample. *TTP* - number of tentative true positives detected per sample. *FP* - number of false positives detected per sample. *TTN* - number of tentative true negatives detected per sample. *FN* - number of false negatives detected per sample. *TN* - number of true negatives detected per sample (evaluation excluding $RT$ position). *FP** - number of false positives detected per sample (evaluation excluding $RT$ position). *TTP** - number of tentative true positives detected per sample (evaluation excluding $RT$ position). *Sensitivity (expert)* - Sensitivity per sample in relation to expert-derived ground truth benchmark; tentative true positives (TTP) are considered FP, tentative true negatives (TTN) are considered FN; sensitivity = TP/(TP+FN+TTN). *Sensitivity (system)* - Sensitivity per sample in relation to system-derived correction benchmark; tentative true positives (TTP) are considered TP, tentative true negatives (TTN) are considered TN; sensitivity=(TP+TTP)/(TP+TTP+FN). *Specificity (expert)* - Specificity per sample in relation to expert-derived ground truth benchmark; tentative true positives (TTP*) are considered FP*; specificity=TN/TN+FP*+TTP*. *Specificity (system)* - Specificity per sample in relation to system-derived correction benchmark; tentative true positives (TTP*) are considered TP; specificity=TN/TN+FP*.

| Sample ID | TP | TTP | FP | TTN | FN | TN | FP* | TTP* | Sensitivity (expert) | Sensitivity (system) | Specificity (expert) | Specificity (system) |
|---|---|---|---|---|---|---|---|---|---|---|---|---|
| 1 | 26 | 3 | 0 | 1 | 0 | 1 | 0 | 2 | 0.963 | 1 | 0.3333 | 1 |
| 2 | 24 | 5 | 0 | 1 | 0 | 1 | 0 | 4 | 0.96 | 1 | 0.2 | 1 |
| 3 | 26 | 3 | 0 | 2 | 0 | 1 | 0 | 1 | 0.9286 | 1 | 0.5 | 1 |
| 4 | 27 | 1 | 0 | 0 | 0 | 2 | 0 | 1 | 1 | 1 | 0.6667 | 1 |
| 5 | 16 | 6 | 0 | 0 | 0 | 8 | 0 | 6 | 1 | 1 | 0.5714 | 1 |
| 6 | 23 | 3 | 0 | 1 | 1 | 3 | 0 | 2 | 0.92 | 0.963 | 0.6 | 1 |
| 7 | 25 | 2 | 0 | 0 | 2 | 1 | 0 | 2 | 0.9259 | 0.931 | 0.3333 | 1 |
| 8 | 23 | 3 | 0 | 0 | 2 | 2 | 0 | 3 | 0.92 | 0.9286 | 0.4 | 1 |
| 9 | 24 | 2 | 0 | 0 | 2 | 2 | 0 | 2 | 0.9231 | 0.9286 | 0.5 | 1 |
| 10 | 9 | 5 | 0 | 0 | 2 | 14 | 0 | 5 | 0.8182 | 0.875 | 0.7368 | 1 |
| 11 | 23 | 5 | 0 | 0 | 1 | 1 | 0 | 5 | 0.9583 | 0.9655 | 0.1667 | 1 |
| 12 | 24 | 5 | 0 | 1 | 0 | 1 | 0 | 4 | 0.96 | 1 | 0.2 | 1 |
| 13 | 22 | 7 | 0 | 0 | 0 | 1 | 0 | 7 | 1 | 1 | 0.125 | 1 |
| 14 | 25 | 3 | 0 | 0 | 0 | 2 | 0 | 3 | 1 | 1 | 0.4 | 1 |
| 15 | 24 | 4 | 1 | 0 | 1 | 1 | 0 | 4 | 0.96 | 0.9655 | 0.2 | 1 |
| 16 | 22 | 3 | 0 | 2 | 1 | 4 | 0 | 1 | 0.88 | 0.9615 | 0.8 | 1 |
| 17 | 22 | 5 | 0 | 2 | 0 | 3 | 0 | 3 | 0.9167 | 1 | 0.5 | 1 |
| 18 | 23 | 2 | 1 | 1 | 2 | 3 | 0 | 1 | 0.8846 | 0.9259 | 0.75 | 1 |
| 19 | 24 | 3 | 0 | 0 | 0 | 3 | 0 | 3 | 1 | 1 | 0.5 | 1 |
| 20 | 22 | 2 | 0 | 0 | 2 | 4 | 0 | 2 | 0.9167 | 0.9231 | 0.6667 | 1 |
| 21 | 17 | 7 | 0 | 0 | 1 | 5 | 0 | 7 | 0.9444 | 0.96 | 0.4167 | 1 |
| 22 | 24 | 6 | 0 | 1 | 0 | 0 | 0 | 5 | 0.96 | 1 | 0 | - |
| 23 | 22 | 6 | 0 | 0 | 0 | 2 | 0 | 6 | 1 | 1 | 0.25 | 1 |
| 24 | 17 | 6 | 0 | 0 | 0 | 7 | 0 | 6 | 1 | 1 | 0.5385 | 1 |
| 25 | 22 | 6 | 0 | 0 | 0 | 2 | 0 | 6 | 1 | 1 | 0.25 | 1 |
| 26 | 15 | 8 | 0 | 0 | 1 | 6 | 0 | 8 | 0.9375 | 0.9583 | 0.4286 | 1 |
| 27 | 19 | 5 | 0 | 1 | 0 | 6 | 0 | 4 | 0.95 | 1 | 0.6 | 1 |
| 28 | 16 | 7 | 0 | 0 | 0 | 7 | 0 | 7 | 1 | 1 | 0.5 | 1 |
| 29 | 16 | 8 | 0 | 1 | 0 | 6 | 0 | 7 | 0.9412 | 1 | 0.4615 | 1 |
| 30 | 9 | 10 | 0 | 0 | 2 | 9 | 0 | 10 | 0.8182 | 0.9048 | 0.4737 | 1 |
| 31 | 19 | 8 | 1 | 0 | 0 | 2 | 1 | 8 | 1 | 1 | 0.1818 | 0.6667 |
| 32 | 20 | 5 | 1 | 0 | 1 | 3 | 1 | 5 | 0.9524 | 0.9615 | 0.3333 | 0.75 |
| 33 | 24 | 3 | 0 | 1 | 1 | 2 | 0 | 2 | 0.9231 | 0.9643 | 0.5 | 1 |
| 34 | 25 | 5 | 0 | 0 | 0 | 0 | 0 | 5 | 1 | 1 | 0 | - |
| 35 | 24 | 4 | 0 | 0 | 0 | 2 | 0 | 4 | 1 | 1 | 0.3333 | 1 |
| 36 | 21 | 6 | 1 | 0 | 0 | 2 | 1 | 6 | 1 | 1 | 0.2222 | 0.6667 |
| 37 | 23 | 4 | 0 | 0 | 0 | 3 | 0 | 4 | 1 | 1 | 0.4286 | 1 |
| 38 | 21 | 5 | 1 | 0 | 0 | 3 | 1 | 5 | 1 | 1 | 0.3333 | 0.75 |
| **TOTAL** | **808** | **181** | **6** | **15** | **22** | **125** | **4** | **166** | **0.9562** | **0.9782** | **0.4237** | **0.969** |

# 5 ResNet-34-1D model – Results

Supplementary Table 5.1: Results of the testing clinical sample analysis with the CNN-based system with ResNet-34-1D model. Results evaluated per each target VOC.

*Label* - the class label of VOC. *TP* - number of true positives detected per VOC. *TTP* - number of tentative true positives detected per VOC. *FP* - number of false positives detected per VOC. *TTN* - number of tentative true negatives detected per VOC. *FN* - number of false negatives detected per VOC. *TN* - number of true negatives detected per VOC (evaluation excluding *RT* position). *FP** - number of false positives detected per VOC (evaluation excluding *RT* position). *TTP** - number of tentative true positives detected per VOC (evaluation excluding *RT* position). *Sensitivity (expert)* - Sensitivity per VOC in relation to expert-derived ground truth benchmark; tentative true positives (TTP) are considered FP, tentative true negatives (TTN) are considered FN; sensitivity = TP/(TP+FN+TTN). *Sensitivity (system)* - Sensitivity per VOC in relation to system-derived correction benchmark; tentative true positives (TTP) are considered TP, tentative true negatives (TTN) are considered TN; sensitivity=(TP+TTP)/(TP+TTP+FN). *Specificity (expert)* - Specificity per VOC in relation to expert-derived ground truth benchmark; tentative true positives (TTP*) are considered FP*; specificity=TN/TN+FP*+TTP*. *Specificity (system)* - Specificity per VOC in relation to system-derived correction benchmark; tentative true positives (TTP*) are considered TP; specificity=TN/TN+FP*. *AP (expert)* - Average precision per VOC in relation to expert-derived ground truth benchmark. *AP (system)* - Average precision per VOC in relation to system-derived correction benchmark.

| Label | TP | TTP | FP | TTN | FN | TN | FP* | TTP* | Sensitivity (expert) | Sensitivity (system) | Specificity (expert) | Specificity (system) | AP (expert) | AP (system) |
|---|---|---|---|---|---|---|---|---|---|---|---|---|---|---|
| 1 | 20 | 18 | 0 | 0 | 0 | 0 | 0 | 18 | 1 | 1 | 0 | - | 0.7242 | 1 |
| 2 | 29 | 9 | 0 | 0 | 0 | 0 | 0 | 9 | 1 | 1 | 0 | - | 0.92 | 1 |
| 3 | 30 | 7 | 0 | 0 | 0 | 1 | 0 | 7 | 1 | 1 | 0.125 | 1 | 0.976 | 1 |
| 4 | 38 | 0 | 0 | 0 | 0 | 0 | 0 | 0 | 1 | 1 | - | - | 1 | 1 |
| 5 | 35 | 3 | 0 | 1 | 0 | 0 | 0 | 2 | 0.9722 | 1 | 0 | - | 0.9211 | 1 |
| 6 | 10 | 27 | 0 | 1 | 0 | 1 | 0 | 26 | 0.9091 | 1 | 0.037 | 1 | 0.7421 | 1 |
| 7 | 22 | 5 | 1 | 0 | 1 | 9 | 1 | 5 | 0.9565 | 0.9643 | 0.6 | 0.9 | 0.9941 | 1 |
| 8 | 37 | 1 | 0 | 0 | 0 | 0 | 0 | 1 | 1 | 1 | 0 | - | 0.9737 | 1 |
| 9 | 38 | 0 | 0 | 0 | 0 | 0 | 0 | 0 | 1 | 1 | - | - | 1 | 1 |
| 10 | 29 | 8 | 0 | 1 | 0 | 1 | 0 | 7 | 0.9667 | 1 | 0.125 | 1 | 0.9695 | 1 |
| 11 | 15 | 16 | 1 | 2 | 2 | 5 | 0 | 14 | 0.7895 | 0.9394 | 0.2632 | 1 | 0.6941 | 0.994 |
| 12 | 21 | 10 | 0 | 1 | 3 | 4 | 0 | 9 | 0.84 | 0.9118 | 0.3077 | 1 | 0.9216 | 1 |
| 13 | 30 | 6 | 0 | 1 | 2 | 0 | 0 | 5 | 0.9091 | 0.9474 | 0 | - | 0.9448 | 1 |
| 14 | 29 | 1 | 0 | 0 | 4 | 4 | 0 | 1 | 0.8788 | 0.8824 | 0.8 | 1 | 0.9977 | 1 |
| 15 | 18 | 10 | 0 | 1 | 4 | 6 | 0 | 9 | 0.7826 | 0.875 | 0.4 | 1 | 0.7106 | 1 |
| 16 | 18 | 4 | 6 | 1 | 4 | 8 | 4 | 3 | 0.7826 | 0.8462 | 0.5333 | 0.6667 | 0.9699 | 0.9512 |
| 17 | 38 | 0 | 0 | 0 | 0 | 0 | 0 | 0 | 1 | 1 | - | - | 1 | 1 |
| 18 | 36 | 2 | 0 | 0 | 0 | 0 | 0 | 2 | 1 | 1 | 0 | - | 0.9591 | 1 |
| 19 | 26 | 6 | 0 | 0 | 0 | 6 | 0 | 6 | 1 | 1 | 0.5 | 1 | 0.9035 | 1 |
| 20 | 35 | 0 | 0 | 0 | 2 | 1 | 0 | 0 | 0.9459 | 0.9459 | 1 | 1 | 1 | 1 |
| 21 | 21 | 16 | 0 | 5 | 1 | 0 | 0 | 11 | 0.7778 | 0.9737 | 0 | - | 0.9118 | 1 |
| 22 | 32 | 5 | 0 | 0 | 0 | 1 | 0 | 5 | 1 | 1 | 0.1667 | 1 | 0.9584 | 1 |
| 23 | 36 | 0 | 0 | 0 | 0 | 2 | 0 | 0 | 1 | 1 | 1 | 1 | 1 | 1 |
| 24 | 23 | 7 | 0 | 0 | 1 | 7 | 0 | 7 | 0.9583 | 0.9677 | 0.5 | 1 | 0.8597 | 1 |
| 25 | 7 | 5 | 1 | 0 | 0 | 25 | 1 | 5 | 1 | 1 | 0.8065 | 0.9615 | 0.9571 | 0.9936 |
| 26 | 21 | 5 | 0 | 0 | 1 | 11 | 0 | 5 | 0.9545 | 0.963 | 0.6875 | 1 | 0.9868 | 1 |
| 27 | 32 | 4 | 0 | 0 | 0 | 2 | 0 | 4 | 1 | 1 | 0.3333 | 1 | 0.9962 | 1 |
| 28 | 16 | 6 | 0 | 0 | 1 | 15 | 0 | 6 | 0.9412 | 0.9565 | 0.7143 | 1 | 0.8889 | 1 |
| 29 | 31 | 3 | 0 | 0 | 0 | 4 | 0 | 3 | 1 | 1 | 0.5714 | 1 | 0.9692 | 1 |
| 30 | 31 | 3 | 0 | 0 | 1 | 3 | 0 | 3 | 0.9688 | 0.9714 | 0.5 | 1 | 0.997 | 1 |
| **TOTAL** | **804** | **187** | **9** | **14** | **27** | **116** | **6** | **173** | **0.9515** | **0.9735** | **0.3932** | **0.9508** | **mAP** | |
| | | | | | | | | | | | | | **0.9282** | **0.998** |

Supplementary Figures 5.1-5.8: Precision against recall graphs for VOCs 1-8.

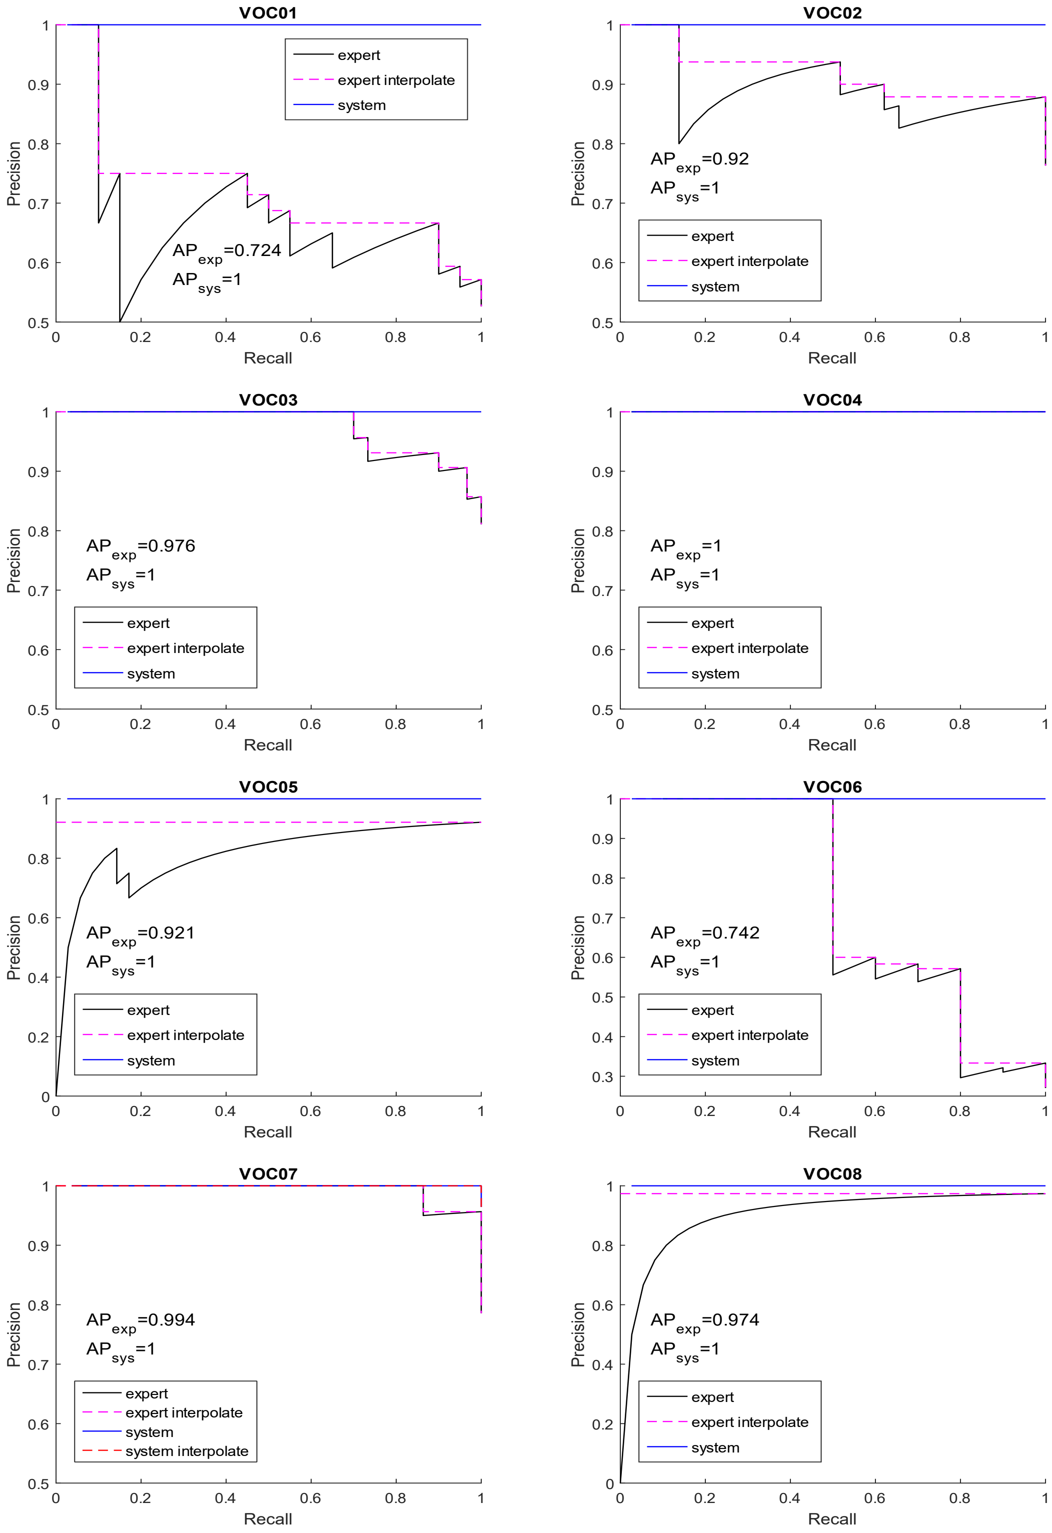

Supplementary Figures 5.9-5.16: Precision against recall graphs for VOCs 9-16.

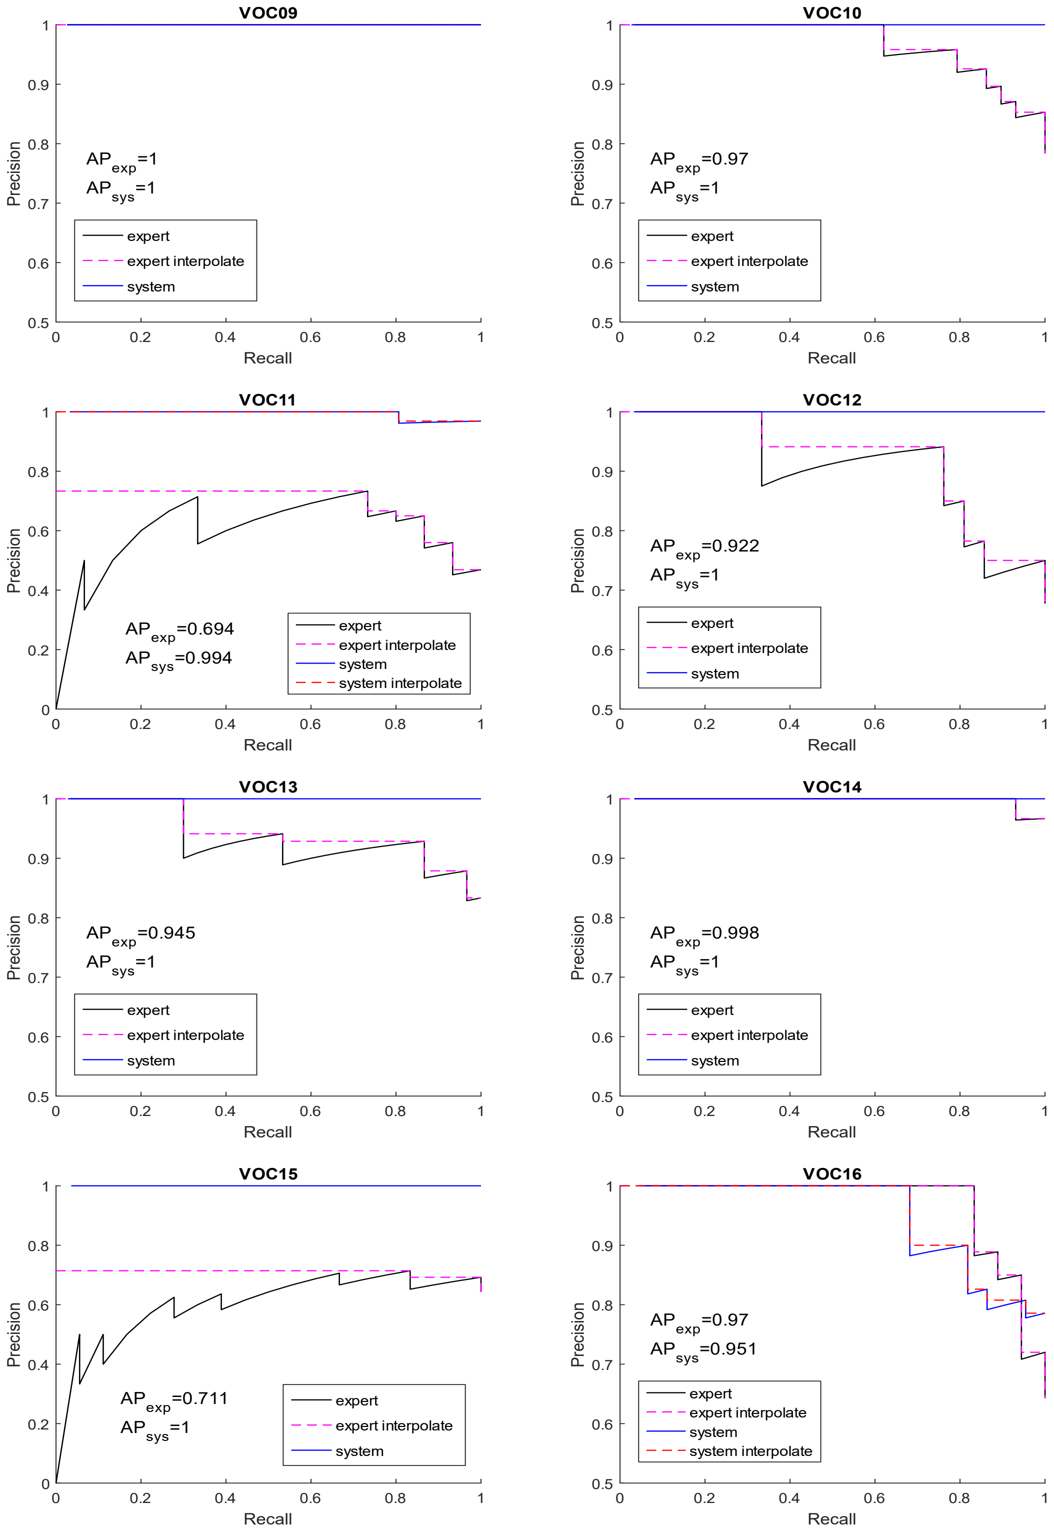

Supplementary Figures 5.17-5.24: Precision against recall graphs for VOCs 17-24.

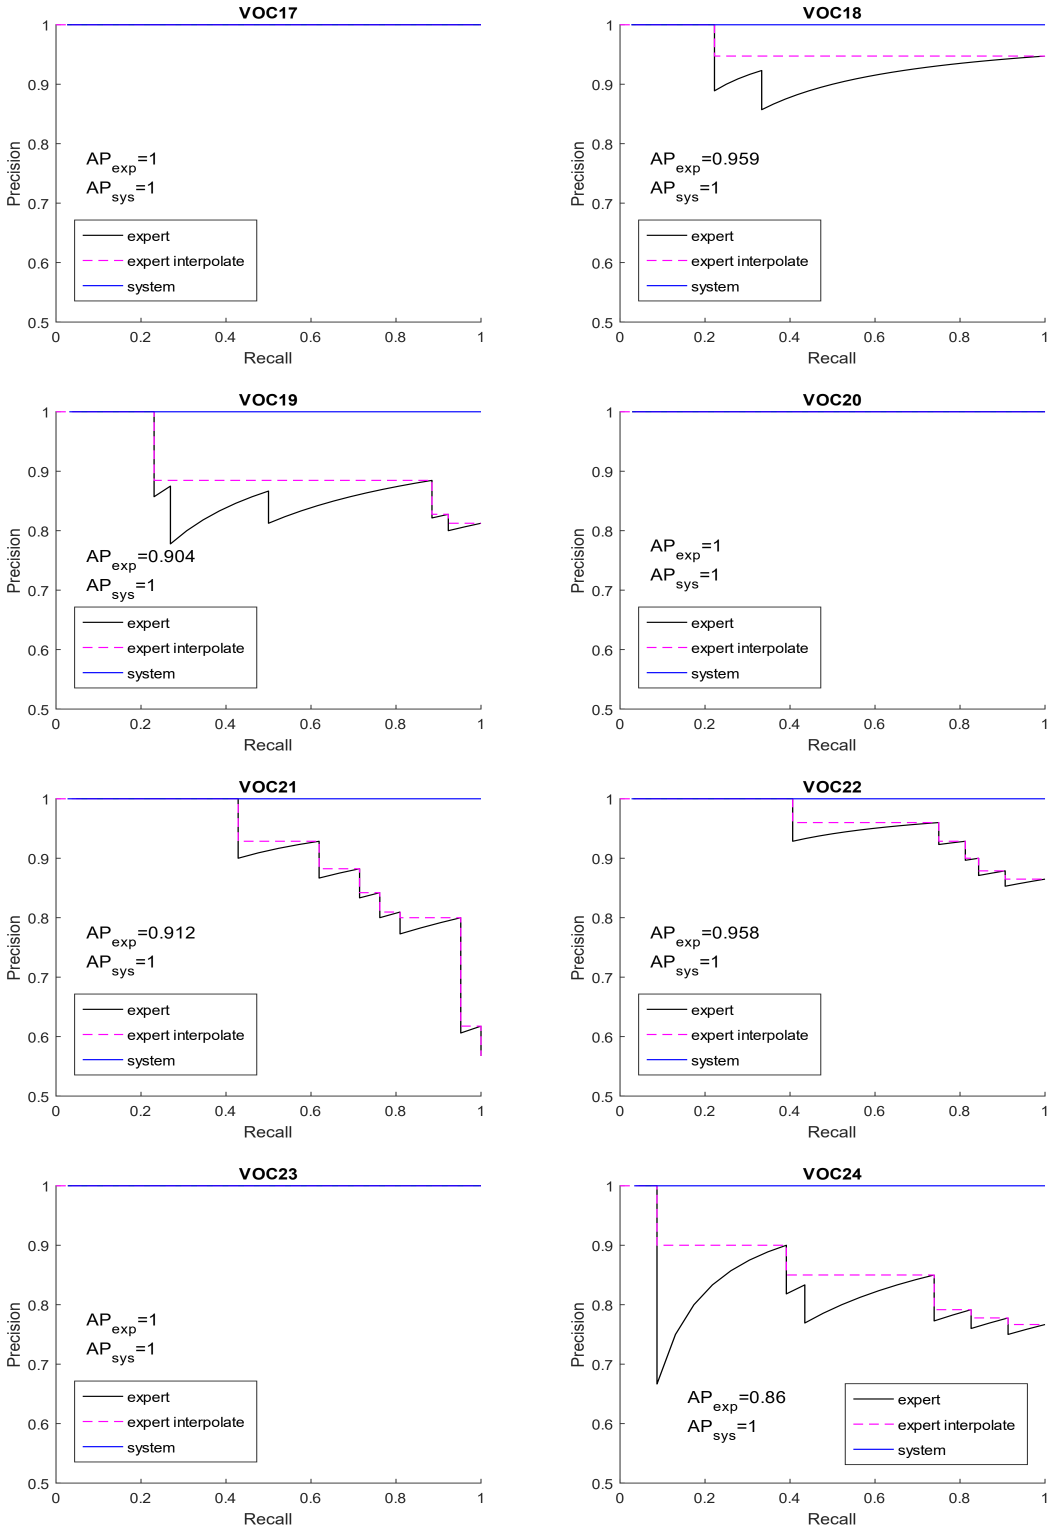

Supplementary Figures 5.25-5.30: Precision against recall graphs for VOCs 25-30.

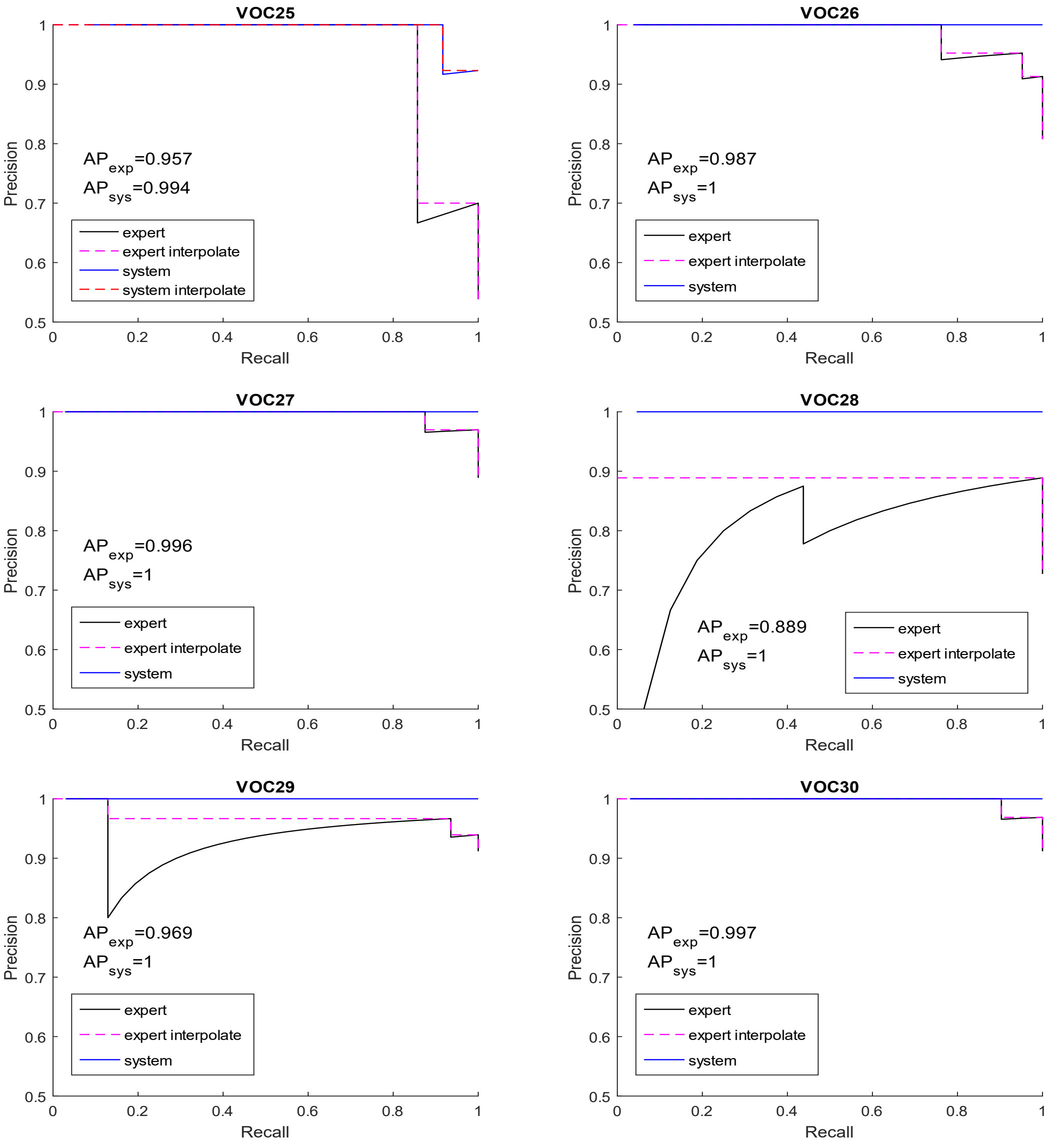

Supplementary Table 5.2: Results of the testing clinical sample analysis with the CNN-based system with ResNet-34-1D model. Results evaluated per each testing sample.

*Sample ID* - number of a sample. *TP* - number of true positives detected per sample. *TTP* - number of tentative true positives detected per sample. *FP* - number of false positives detected per sample. *TTN* - number of tentative true negatives detected per sample. *FN* - number of false negatives detected per sample. *TN* - number of true negatives detected per sample (evaluation excluding $RT$ position). *FP** - number of false positives detected per sample (evaluation excluding $RT$ position). *TTP** - number of tentative true positives detected per sample (evaluation excluding $RT$ position). *Sensitivity (expert)* - Sensitivity per sample in relation to expert-derived ground truth benchmark; tentative true positives (TTP) are considered FP, tentative true negatives (TTN) are considered FN; sensitivity = TP/(TP+FN+TTN). *Sensitivity (system)* - Sensitivity per sample in relation to system-derived correction benchmark; tentative true positives (TTP) are considered TP, tentative true negatives (TTN) are considered TN; sensitivity=(TP+TTP)/(TP+TTP+FN). *Specificity (expert)* - Specificity per sample in relation to expert-derived ground truth benchmark; tentative true positives (TTP*) are considered FP*; specificity=TN/TN+FP*+TTP*. *Specificity (system)* - Specificity per sample in relation to system-derived correction benchmark; tentative true positives (TTP*) are considered TP; specificity=TN/TN+FP*.

| Sample ID | TP | TTP | FP | TTN | FN | TN | FP* | TTP* | Sensitivity (expert) | Sensitivity (system) | Specificity (expert) | Specificity (system) |
|---|---|---|---|---|---|---|---|---|---|---|---|---|
| 1 | 27 | 2 | 0 | 0 | 0 | 1 | 0 | 2 | 1 | 1 | 0.3333 | 1 |
| 2 | 24 | 5 | 0 | 1 | 0 | 1 | 0 | 4 | 0.96 | 1 | 0.2 | 1 |
| 3 | 26 | 3 | 0 | 2 | 0 | 1 | 0 | 1 | 0.9286 | 1 | 0.5 | 1 |
| 4 | 27 | 1 | 0 | 0 | 0 | 2 | 0 | 1 | 1 | 1 | 0.6667 | 1 |
| 5 | 15 | 7 | 0 | 0 | 1 | 7 | 0 | 7 | 0.9375 | 0.9565 | 0.5 | 1 |
| 6 | 23 | 4 | 0 | 1 | 1 | 2 | 0 | 3 | 0.92 | 0.9643 | 0.4 | 1 |
| 7 | 24 | 2 | 0 | 0 | 3 | 1 | 0 | 2 | 0.8889 | 0.8966 | 0.3333 | 1 |
| 8 | 23 | 3 | 0 | 0 | 2 | 2 | 0 | 3 | 0.92 | 0.9286 | 0.4 | 1 |
| 9 | 24 | 2 | 0 | 0 | 2 | 2 | 0 | 2 | 0.9231 | 0.9286 | 0.5 | 1 |
| 10 | 9 | 7 | 0 | 0 | 2 | 12 | 0 | 7 | 0.8182 | 0.8889 | 0.6316 | 1 |
| 11 | 24 | 5 | 0 | 0 | 0 | 1 | 0 | 5 | 1 | 1 | 0.1667 | 1 |
| 12 | 24 | 5 | 0 | 1 | 0 | 1 | 0 | 4 | 0.96 | 1 | 0.2 | 1 |
| 13 | 22 | 6 | 1 | 0 | 0 | 1 | 1 | 6 | 1 | 1 | 0.125 | 0.5 |
| 14 | 24 | 3 | 1 | 0 | 1 | 2 | 0 | 3 | 0.96 | 0.9643 | 0.4 | 1 |
| 15 | 24 | 4 | 1 | 0 | 1 | 1 | 0 | 4 | 0.96 | 0.9655 | 0.2 | 1 |
| 16 | 19 | 5 | 1 | 3 | 3 | 3 | 0 | 2 | 0.76 | 0.8889 | 0.6 | 1 |
| 17 | 22 | 5 | 1 | 2 | 0 | 2 | 1 | 3 | 0.9167 | 1 | 0.3333 | 0.6667 |
| 18 | 23 | 2 | 0 | 1 | 2 | 3 | 0 | 1 | 0.8846 | 0.9259 | 0.75 | 1 |
| 19 | 23 | 3 | 0 | 1 | 0 | 4 | 0 | 2 | 0.9583 | 1 | 0.6667 | 1 |
| 20 | 22 | 2 | 0 | 0 | 2 | 4 | 0 | 2 | 0.9167 | 0.9231 | 0.6667 | 1 |
| 21 | 17 | 6 | 0 | 0 | 1 | 6 | 0 | 6 | 0.9444 | 0.9583 | 0.5 | 1 |
| 22 | 24 | 5 | 0 | 0 | 1 | 0 | 0 | 5 | 0.96 | 0.9667 | 0 | - |
| 23 | 22 | 5 | 1 | 0 | 0 | 2 | 1 | 5 | 1 | 1 | 0.25 | 0.6667 |
| 24 | 17 | 5 | 0 | 0 | 0 | 8 | 0 | 5 | 1 | 1 | 0.6154 | 1 |
| 25 | 22 | 6 | 0 | 0 | 0 | 2 | 0 | 6 | 1 | 1 | 0.25 | 1 |
| 26 | 16 | 8 | 0 | 0 | 0 | 6 | 0 | 8 | 1 | 1 | 0.4286 | 1 |
| 27 | 19 | 7 | 0 | 1 | 0 | 4 | 0 | 6 | 0.95 | 1 | 0.4 | 1 |
| 28 | 15 | 9 | 0 | 0 | 1 | 5 | 0 | 9 | 0.9375 | 0.96 | 0.3571 | 1 |
| 29 | 16 | 7 | 0 | 0 | 1 | 6 | 0 | 7 | 0.9412 | 0.9583 | 0.4615 | 1 |
| 30 | 10 | 13 | 0 | 0 | 1 | 6 | 0 | 13 | 0.9091 | 0.9583 | 0.3158 | 1 |
| 31 | 19 | 6 | 1 | 0 | 0 | 4 | 1 | 6 | 1 | 1 | 0.3636 | 0.8 |
| 32 | 20 | 5 | 1 | 0 | 1 | 3 | 1 | 5 | 0.9524 | 0.9615 | 0.3333 | 0.75 |
| 33 | 25 | 4 | 0 | 1 | 0 | 1 | 0 | 3 | 0.9615 | 1 | 0.25 | 1 |
| 34 | 24 | 5 | 0 | 0 | 1 | 0 | 0 | 5 | 0.96 | 0.9667 | 0 | - |
| 35 | 24 | 4 | 0 | 0 | 0 | 2 | 0 | 4 | 1 | 1 | 0.3333 | 1 |
| 36 | 21 | 5 | 1 | 0 | 0 | 3 | 1 | 5 | 1 | 1 | 0.3333 | 0.75 |
| 37 | 23 | 4 | 0 | 0 | 0 | 3 | 0 | 4 | 1 | 1 | 0.4286 | 1 |
| 38 | 21 | 7 | 0 | 0 | 0 | 2 | 0 | 7 | 1 | 1 | 0.2222 | 1 |
| **TOTAL** | **804** | **187** | **9** | **14** | **27** | **116** | **6** | **173** | **0.9515** | **0.9735** | **0.3932** | **0.9508** |

# 6 Intersection of the models – Results

Supplementary Table 6.1: Intersection of the results of the testing clinical sample analysis with the CNN-based system with all tested models (i.e. detections consistent in terms of label and *RT* location among all the models). Results evaluated per each target VOC.

Label - the class label of VOC. TP - number of true positives detected per VOC. TTP - number of tentative true positives detected per VOC. FP - number of false positives detected per VOC. TTN - number of tentative true negatives detected per VOC. FN - number of false negatives detected per VOC. TN - number of true negatives detected per VOC (evaluation excluding *RT* position). *FP** - number of false positives detected per VOC (evaluation excluding *RT* position). *TTP** - number of tentative true positives detected per VOC (evaluation excluding *RT* position). *Sensitivity (expert)* - Sensitivity per VOC in relation to expert-derived ground truth benchmark; tentative true positives (TTP) are considered FP, tentative true negatives (TTN) are considered FN; sensitivity = TP/(TP+FN+TTN). *Sensitivity (system)* - Sensitivity per VOC in relation to system-derived correction benchmark; tentative true positives (TTP) are considered TP, tentative true negatives (TTN) are considered TN; sensitivity=(TP+TTP)/(TP+TTP+FN). *Specificity (expert)* - Specificity per VOC in relation to expert-derived ground truth benchmark; tentative true positives (TTP*) are considered FP*; specificity=TN/TN+FP*+TTP*. *Specificity (system)* - Specificity per VOC in relation to system-derived correction benchmark; tentative true positives (TTP*) are considered TP; specificity=TN/TN+FP*. *AP (expert)* - Average precision per VOC in relation to expert-derived ground truth benchmark. *AP (system)* - Average precision per VOC in relation to system-derived correction benchmark.

| Label | TP | TTP | FP | TTN | FN | TN | FP* | TTP* | Sensitivity (expert) | Sensitivity (system) | Specificity (expert) | Specificity (system) | AP (expert) | AP (system) |
|---|---|---|---|---|---|---|---|---|---|---|---|---|---|---|
| 1 | 20 | 18 | 0 | 0 | 0 | 0 | 0 | 18 | 1 | 1 | - | - | 0.7436 | 1 |
| 2 | 29 | 6 | 0 | 0 | 0 | 3 | 0 | 6 | 1 | 1 | 0.3333 | - | 0.9173 | 1 |
| 3 | 30 | 6 | 0 | 0 | 0 | 2 | 0 | 6 | 1 | 1 | 0.25 | 1 | 0.9925 | 1 |
| 4 | 36 | 0 | 0 | 0 | 2 | 0 | 0 | 0 | 0.9474 | 0.9474 | - | - | 1 | 1 |
| 5 | 35 | 3 | 0 | 1 | 0 | 0 | 0 | 2 | 0.9722 | 1 | - | - | 0.9233 | 1 |
| 6 | 10 | 27 | 0 | 1 | 0 | 1 | 0 | 26 | 0.9091 | 1 | 0.037 | 1 | 0.8035 | 1 |
| 7 | 22 | 3 | 0 | 0 | 1 | 12 | 0 | 3 | 0.9565 | 0.9615 | 0.8 | 1 | 0.998 | 1 |
| 8 | 37 | 1 | 0 | 0 | 0 | 0 | 0 | 1 | 1 | 1 | - | - | 0.9737 | 1 |
| 9 | 38 | 0 | 0 | 0 | 0 | 0 | 0 | 0 | 1 | 1 | - | - | 1 | 1 |
| 10 | 29 | 4 | 0 | 0 | 1 | 4 | 0 | 4 | 0.9667 | 0.9706 | 0.5 | 1 | 0.992 | 1 |
| 11 | 12 | 7 | 0 | 0 | 7 | 12 | 0 | 7 | 0.6316 | 0.7308 | 0.6316 | 1 | 0.67 | 1 |
| 12 | 20 | 7 | 0 | 1 | 4 | 7 | 0 | 6 | 0.8 | 0.871 | 0.5385 | 1 | 0.9357 | 1 |
| 13 | 30 | 4 | 0 | 1 | 2 | 2 | 0 | 3 | 0.9091 | 0.9444 | 0.4 | - | 0.9518 | 1 |
| 14 | 28 | 1 | 0 | 0 | 5 | 4 | 0 | 1 | 0.8485 | 0.8529 | 0.8 | 1 | 0.9988 | 1 |
| 15 | 17 | 10 | 0 | 1 | 5 | 6 | 0 | 9 | 0.7391 | 0.8438 | 0.4 | 1 | 0.7873 | 1 |
| 16 | 18 | 1 | 1 | 0 | 3 | 15 | 0 | 1 | 0.8571 | 0.8636 | 0.9375 | 1 | 0.9971 | 0.9947 |
| 17 | 38 | 0 | 0 | 0 | 0 | 0 | 0 | 0 | 1 | 1 | - | - | 1 | 1 |
| 18 | 31 | 2 | 0 | 0 | 5 | 0 | 0 | 2 | 0.8611 | 0.8684 | - | - | 0.9511 | 1 |
| 19 | 26 | 4 | 0 | 0 | 0 | 9 | 0 | 4 | 1 | 1 | 0.6923 | 1 | 0.9108 | 1 |
| 20 | 35 | 0 | 0 | 0 | 2 | 1 | 0 | 0 | 0.9459 | 0.9459 | 1 | 1 | 1 | 1 |
| 21 | 20 | 5 | 0 | 3 | 4 | 9 | 0 | 2 | 0.7407 | 0.8621 | 0.8182 | - | 0.9808 | 1 |
| 22 | 32 | 5 | 0 | 0 | 0 | 1 | 0 | 5 | 1 | 1 | 0.1667 | 1 | 0.9416 | 1 |
| 23 | 36 | 0 | 0 | 0 | 0 | 2 | 0 | 0 | 1 | 1 | 1 | 1 | 1 | 1 |
| *24* | 23 | 6 | 0 | 0 | 2 | 7 | 0 | 6 | 0.92 | 0.9355 | 0.5385 | 1 | 0.8964 | 1 |
| 25 | 7 | 3 | 0 | 0 | 0 | 28 | 0 | 3 | 1 | 1 | 0.9032 | 1 | 0.9821 | 1 |
| *26* | 19 | 5 | 0 | 0 | 3 | 11 | 0 | 5 | 0.8636 | 0.8889 | 0.6875 | 1 | 0.9947 | 1 |
| 27 | 32 | 2 | 0 | 0 | 0 | 4 | 0 | 2 | 1 | 1 | 0.6667 | 1 | 0.9991 | 1 |
| 28 | 16 | 4 | 0 | 0 | 1 | 17 | 0 | 4 | 0.9412 | 0.9524 | 0.8095 | 1 | 0.8889 | 1 |
| 29 | 31 | 2 | 0 | 0 | 0 | 5 | 0 | 2 | 1 | 1 | 0.7143 | 1 | 0.9674 | 1 |
| 30 | 30 | 2 | 0 | 0 | 2 | 3 | 0 | 2 | 0.9375 | 0.9412 | 0.6 | 1 | 0.9978 | 1 |
| **TOTAL** | **787** | **138** | **1** | **8** | **49** | **165** | **0** | **130** | **0.9325** | **0.9497** | **0.5593** | **1** | **mAP** | |
| | | | | | | | | | | | | | **0.9398** | **1** |

Supplementary Figures 6.1-6.8: Precision against recall graphs for VOCs 1-8.

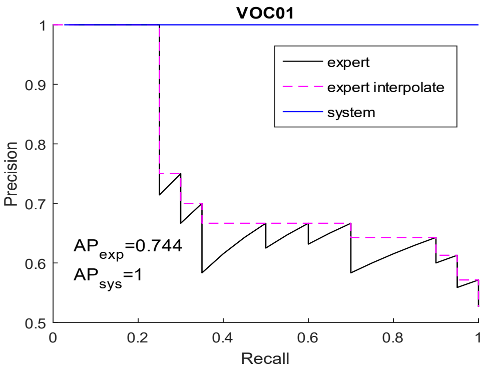


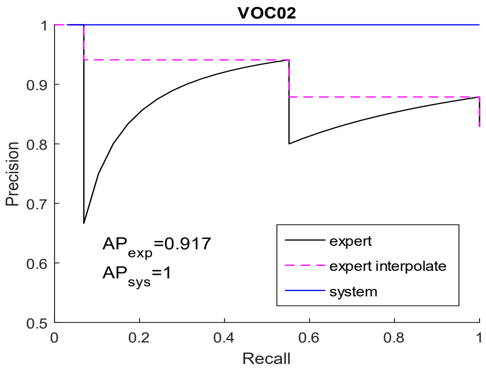


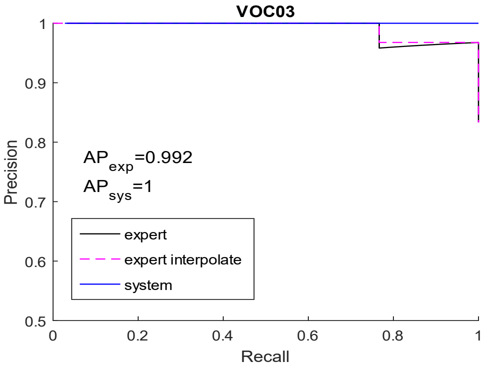


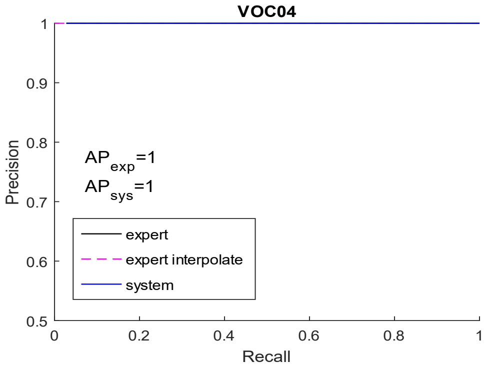


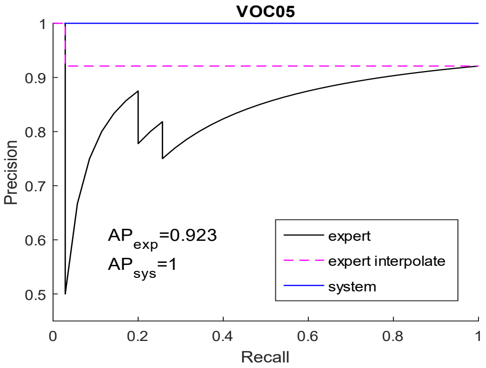


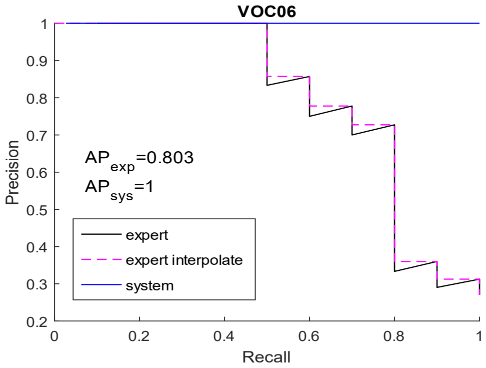


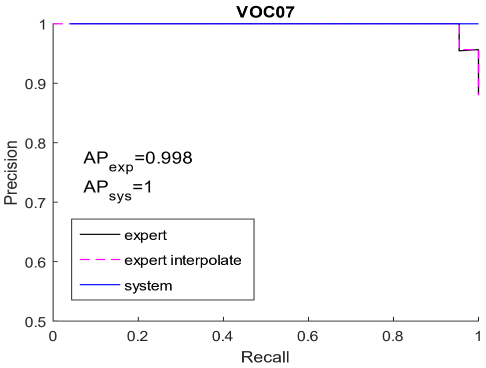


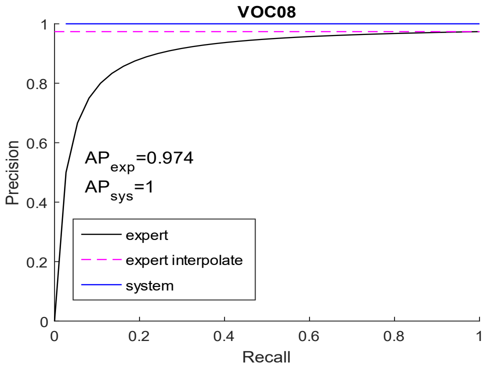

Supplementary Figures 6.9-6.16: Precision against recall graphs for VOCs 9-16.

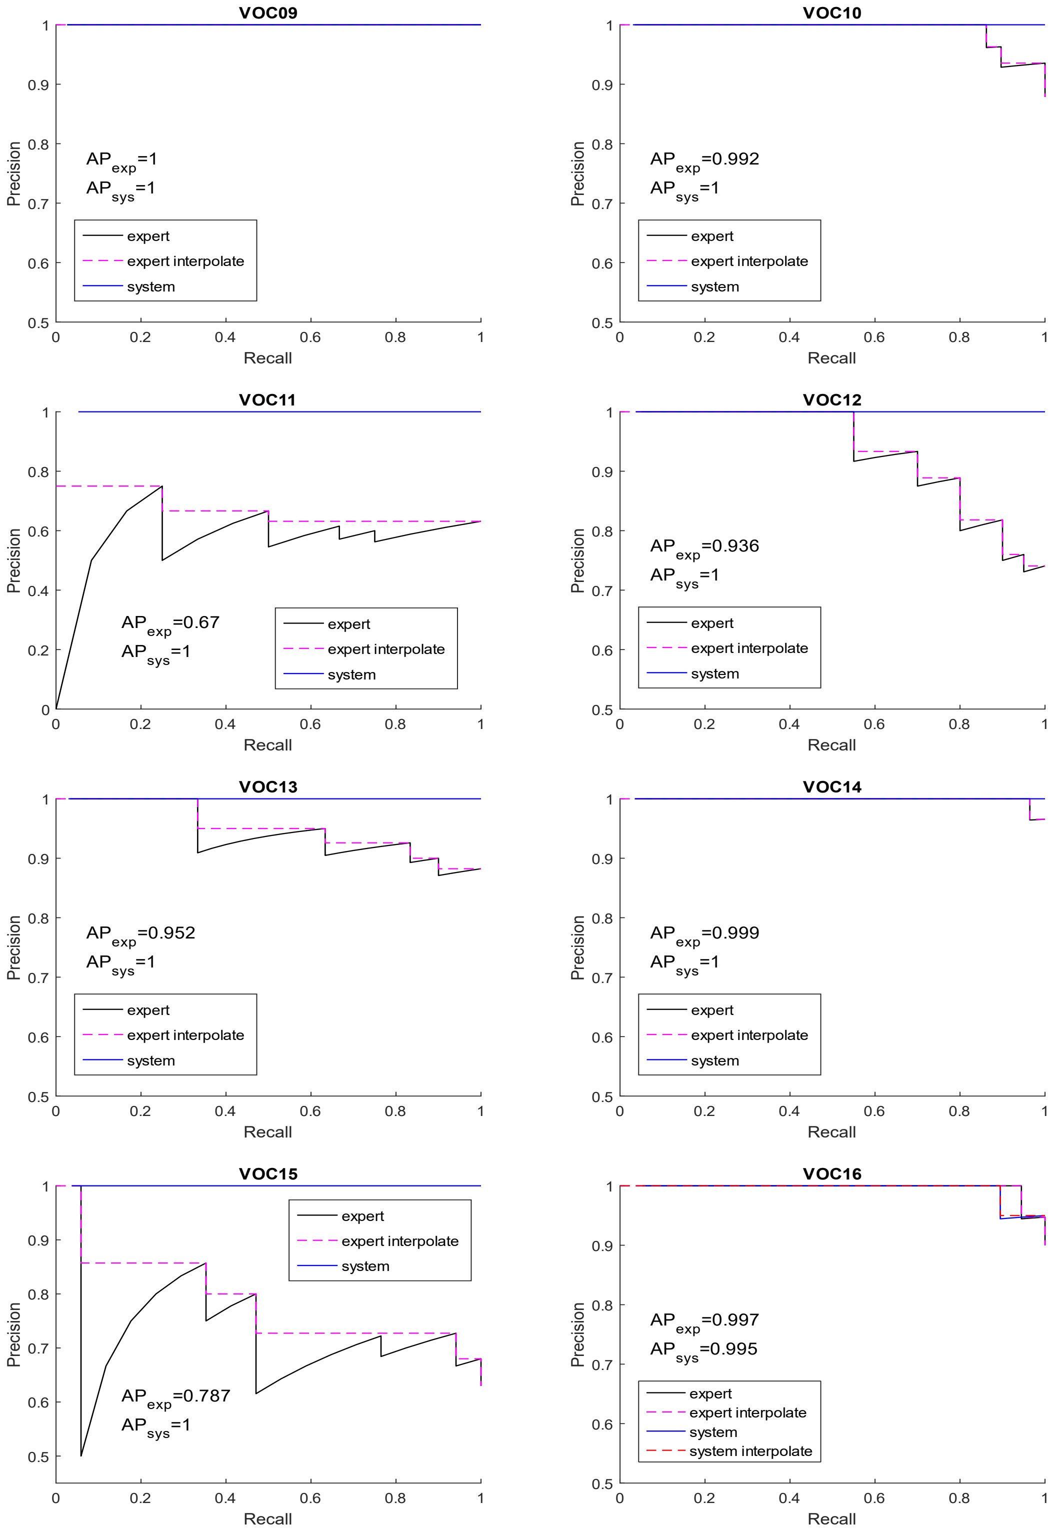

Supplementary Figures 6.17-6.24: Precision against recall graphs for VOCs 17-24.

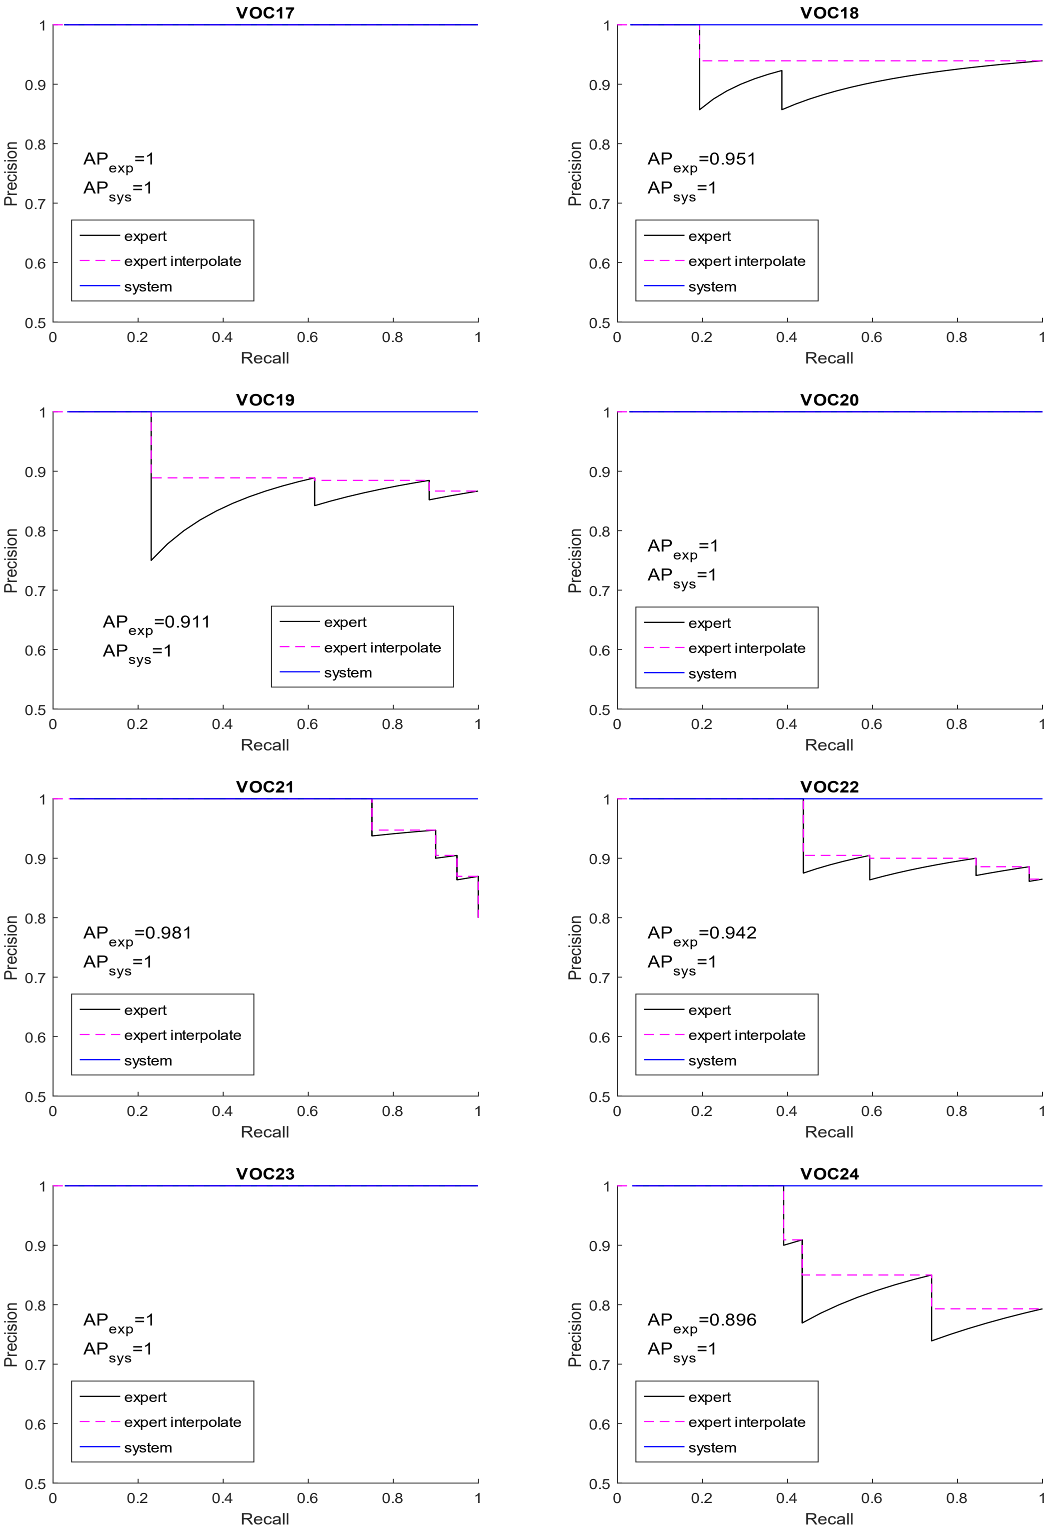

Supplementary Figures 6.25-6.30: Precision against recall graphs for VOCs 25-30.

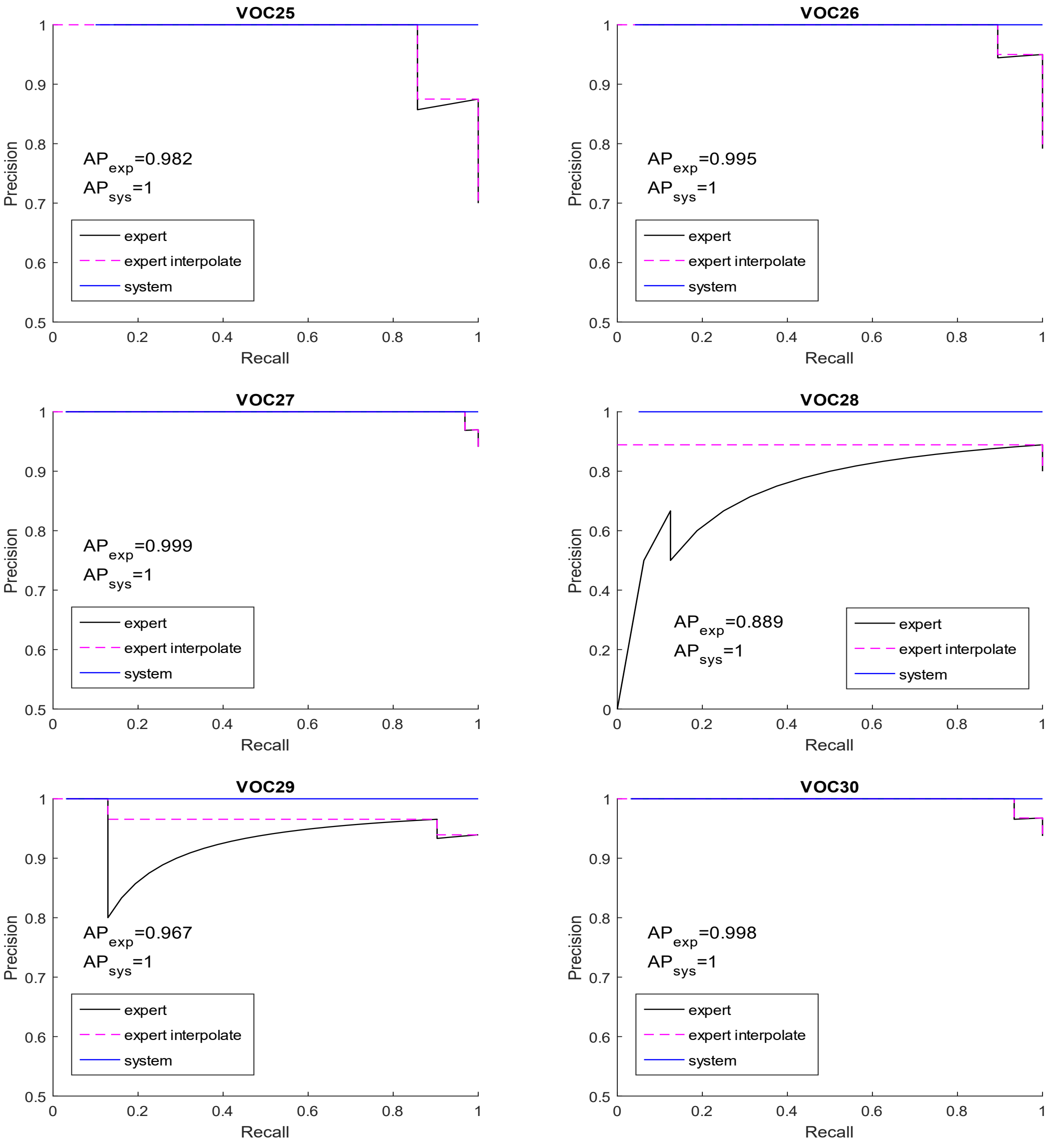

Supplementary Table 6.2: Intersection of the results of the testing clinical sample analysis with the CNN-based system with all tested models (i.e. detections consistent in terms of label and $RT$ location among all the models). Results evaluated per each testing sample.

Label - the class label of VOC. TP - number of true positives detected per VOC. TTP - number of tentative true positives detected per VOC. FP - number of false positives detected per VOC. TTN - number of tentative true negatives detected per VOC. FN - number of false negatives detected per VOC. TN - number of true negatives detected per VOC (evaluation excluding $RT$ position). *FP** - number of false positives detected per VOC (evaluation excluding $RT$ position). *TTP** - number of tentative true positives detected per VOC (evaluation excluding $RT$ position). *Sensitivity (expert)* - Sensitivity per VOC in relation to expert-derived ground truth benchmark; tentative true positives (TTP) are considered FP, tentative true negatives (TTN) are considered FN; sensitivity = TP/(TP+FN+TTN). *Sensitivity (system)* - Sensitivity per VOC in relation to system-derived correction benchmark; tentative true positives (TTP) are considered TP, tentative true negatives (TTN) are considered TN; sensitivity=(TP+TTP)/(TP+TTP+FN). *Specificity (expert)* - Specificity per VOC in relation to expert-derived ground truth benchmark; tentative true positives (TTP*) are considered FP*; specificity=TN/TN+FP*+TTP*. *Specificity (system)* - Specificity per VOC in relation to system-derived correction benchmark; tentative true positives (TTP*) are considered TP; specificity=TN/TN+FP*.

| Sample ID | TP | TTP | FP | TTN | FN | TN | FP* | TTP* | Sensitivity (expert) | Sensitivity (system) | Specificity (expert) | Specificity (system) |
|---|---|---|---|---|---|---|---|---|---|---|---|---|
| 1 | 26 | 2 | 0 | 0 | 1 | 1 | 0 | 2 | 1 | 1 | 0.3333 | 1 |
| 2 | 24 | 4 | 0 | 0 | 1 | 1 | 0 | 4 | 1 | 1 | 0.2 | 1 |
| 3 | 26 | 2 | 0 | 1 | 1 | 1 | 0 | 1 | 0.963 | 0.9655 | 0.5 | 1 |
| 4 | 27 | 0 | 0 | 0 | 0 | 3 | 0 | 0 | 1 | 1 | - | - |
| 5 | 15 | 4 | 0 | 0 | 1 | 10 | 0 | 4 | 1 | 1 | 0.2 | 1 |
| 6 | 23 | 2 | 0 | 1 | 1 | 4 | 0 | 1 | 0.9583 | 0.9615 | 0.5 | 1 |
| 7 | 24 | 1 | 0 | 0 | 3 | 2 | 0 | 1 | 1 | 1 | 0.75 | 1 |
| 8 | 23 | 2 | 0 | 0 | 2 | 3 | 0 | 2 | 1 | 1 | 0.5 | 1 |
| 9 | 24 | 1 | 0 | 0 | 2 | 3 | 0 | 1 | 1 | 1 | 0.6667 | 1 |
| 10 | 9 | 5 | 0 | 0 | 2 | 14 | 0 | 5 | 1 | 1 | 0.2857 | 1 |
| 11 | 23 | 4 | 0 | 0 | 1 | 2 | 0 | 4 | 1 | 1 | 0.2 | 1 |
| 12 | 24 | 4 | 0 | 1 | 0 | 2 | 0 | 3 | 0.96 | 0.9655 | - | - |
| 13 | 22 | 5 | 0 | 0 | 0 | 3 | 0 | 5 | 1 | 1 | - | - |
| 14 | 24 | 2 | 0 | 0 | 1 | 3 | 0 | 2 | 1 | 1 | 0.3333 | 1 |
| 15 | 24 | 3 | 1 | 0 | 0 | 2 | 0 | 3 | 0.96 | 1 | - | - |
| 16 | 18 | 2 | 0 | 1 | 6 | 4 | 0 | 1 | 0.9474 | 0.9524 | 0.8571 | 1 |
| 17 | 21 | 5 | 0 | 2 | 1 | 3 | 0 | 3 | 0.913 | 0.9286 | 0.25 | 1 |
| 18 | 22 | 2 | 0 | 1 | 3 | 3 | 0 | 1 | 0.9565 | 0.96 | 0.75 | 1 |
| 19 | 22 | 2 | 0 | 0 | 2 | 4 | 0 | 2 | 1 | 1 | 0.5 | 1 |
| 20 | 21 | 2 | 0 | 0 | 3 | 4 | 0 | 2 | 1 | 1 | 0.6 | 1 |
| 21 | 16 | 4 | 0 | 0 | 2 | 8 | 0 | 4 | 1 | 1 | 0.3333 | 1 |
| 22 | 23 | 4 | 0 | 0 | 2 | 1 | 0 | 4 | 1 | 1 | 0.3333 | - |
| 23 | 21 | 4 | 0 | 0 | 1 | 4 | 0 | 4 | 1 | 1 | 0.2 | 1 |
| 24 | 17 | 5 | 0 | 0 | 0 | 8 | 0 | 5 | 1 | 1 | - | - |
| 25 | 22 | 4 | 0 | 0 | 0 | 4 | 0 | 4 | 1 | 1 | - | - |
| 26 | 15 | 6 | 0 | 0 | 1 | 8 | 0 | 6 | 1 | 1 | 0.1429 | 1 |
| 27 | 19 | 5 | 0 | 1 | 0 | 6 | 0 | 4 | 0.95 | 0.96 | - | - |
| 28 | 15 | 7 | 0 | 0 | 1 | 7 | 0 | 7 | 1 | 1 | 0.125 | 1 |
| 29 | 16 | 7 | 0 | 0 | 1 | 6 | 0 | 7 | 1 | 1 | 0.125 | 1 |
| 30 | 9 | 10 | 0 | 0 | 2 | 9 | 0 | 10 | 1 | 1 | 0.1667 | 1 |
| 31 | 19 | 4 | 0 | 0 | 0 | 7 | 0 | 4 | 1 | 1 | - | - |
| 32 | 20 | 4 | 0 | 0 | 1 | 5 | 0 | 4 | 1 | 1 | 0.2 | 1 |
| 33 | 23 | 2 | 0 | 0 | 3 | 2 | 0 | 2 | 1 | 1 | 0.6 | 1 |
| 34 | 23 | 4 | 0 | 0 | 2 | 1 | 0 | 4 | 1 | 1 | 0.3333 | - |
| 35 | 24 | 3 | 0 | 0 | 0 | 3 | 0 | 3 | 1 | 1 | - | - |
| 36 | 20 | 4 | 0 | 0 | 1 | 5 | 0 | 4 | 1 | 1 | 0.2 | 1 |
| 37 | 22 | 3 | 0 | 0 | 1 | 4 | 0 | 3 | 1 | 1 | 0.25 | 1 |
| 38 | 21 | 4 | 0 | 0 | 0 | 5 | 0 | 4 | 1 | 1 | - | - |
| **TOTAL** | **787** | **138** | **1** | **8** | **49** | **165** | **0** | **130** | **0.9325** | **0.9497** | **0.5593** | **1** |

# 7 GC-MS instrumentation

Supplementary Table 7: GC-MS instrumentation parameters.

| Thermal desorption | | Gas chromatography | | Mass spectrometer | |
|---|---|---|---|---|---|
| **Parameters** | **Setting** | **Parameters** | **Setting** | **Parameters** | **Setting** |
| ***t*** - Primary desorption | 1 min | ***F*** - He carrier gas | 2 $cm^3$ $min^{-1}$ | Scan type | Full scan (+ve) |
| ***F*** - Primary desorption | 40 $cm^3$ $min^{-1}$ | ***T*** - Initial | 40°C | Mass range | 40 to 550 m/z |
| ***T*** - Primary desorption | 300°C | ***t*** - Initial hold | 0 min | Ionisation type | EI |
| ***t*** - Secondary desorption | 5 min | ***T*** - program | 5°C $min^{-1}$ to 300°C | ***v*** - scan | 3 Hz |
| ***F*** - Secondary desorption | 50 $cm^3$ $min^{-1}$ | ***T*** - End | 300 °C | ***T*** - line temperature | 300°C |
| ***T*** - Secondary desorption | 300°C | ***t*** - End hold | 0 min | ***T*** - Quadrupole | 150°C |
| ***F*** - Cold trap | 20 $cm^3$ $min^{-1}$ | ***t*** - Total run | 60 min | ***T*** - Manifold | 230°C |
| ***T*** - Cold trap | -10°C | ***T*** - Post run | 45°C | ***t*** - Solvent delay | 5 min |
| $(\delta T/\delta t)_{trap}$ | Max °C $min^{-1}$ | ***t*** - Post run | 0 min | | |
| ***T*** - Trap high | 300°C | | | | |
| ***t*** - Trap hold | 5 min | | | | |
| ***T*** - Flow path | 200°C | | | | |
| Mode | Spitless | | | | |

Note: ***t***, time; ***F***, flow; ***T***, temperature; and ***v***, frequency.
